# Supplementary material for: Causal Inference in Possibly Nonlinear Factor Models
Source: arXiv:2008.13651 source file (2026-09-30)
Supplement: Supplementary file 1 [file supp.tex]

\documentclass[12pt]{article} 
\pdfoutput=1 
\usepackage{amsfonts,amssymb,amsmath,amsthm,dsfont,graphicx,hyperref,mathrsfs,euscript,enumitem,framed, bm}
\usepackage[title, titletoc]{appendix}
\usepackage[top=1in,bottom=1in,left=1in,right=1in]{geometry} % the layout package
\usepackage[onehalfspacing]{setspace}
\usepackage{ifthen,caption,subcaption,lscape}
\hypersetup{pdfborder = {0 0 0},colorlinks=true,linkcolor=blue,urlcolor=blue,citecolor=blue}
\usepackage{chngcntr} 
\usepackage{natbib}
\usepackage{longtable}
\usepackage{placeins}

\newtheorem{thm}{Theorem}
\newtheorem{coro}{Corollary}
\newtheorem{lem}{Lemma}
\newtheorem{assumption}{Assumption}

\theoremstyle{definition}
\newtheorem{definition}{Definition}
%%% REMARK
\theoremstyle{definition}
\newtheorem{remark_tmp}{Remark}[section]
\newenvironment{remark}
{ \begin{remark_tmp} 	}
	{ 
		%\renewcommand{\bqedsymbol}{$\bm{\ell}acksquare$}
		%\medskip\bqed 
		\medskip\hfill{\LARGE$\lrcorner$}
	\end{remark_tmp} 
}

\newtheorem{exmp}{Example}[section]

\allowdisplaybreaks[1]

%New operators: trace, argmin, argmax, etc
\DeclareMathOperator*{\argmin}{arg\,min}
\DeclareMathOperator*{\argmax}{arg\,max}

\DeclareMathOperator*{\tr}{Tr}

\DeclareMathOperator*{\diag}{diag}

%independence
\newcommand\inde{\protect\mathpalette{\protect\independenT}{\perp}}
\def\independenT#1#2{\mathrel{\rlap{$#1#2$}\mkern2mu{#1#2}}}

% % % % % % % % % % % % % % Some Notations % % % % % % % % % % % % % %
\renewcommand{\P}{\mathbb{P}}
\newcommand{\E}{\mathbb{E}}
\newcommand{\V}{\mathbb{V}}

\newcommand{\I}{\mathds{1}}

% % % % % % % % % Special subscript  % % % % % % % % %%
\newcommand{\subi}{\langle i \rangle}
\newcommand{\gr}[1]{\cdot\mathcal{C}_{#1}}

% % % % % % % % % % % % % % Bold letters % % % % % % % % % % % % % %
\newcommand{\bA}{\bm{A}}
\newcommand{\bH}{\bm{H}}

\newcommand{\bB}{\bm{B}}

\newcommand{\bF}{\bm{F}}
\newcommand{\bG}{\bm{G}}
\newcommand{\bff}{\mathbf{f}}
\newcommand{\bI}{\bm{I}}
\newcommand{\bL}{\bm{L}}
\newcommand{\bM}{\bm{M}}

\newcommand{\bP}{\bm{P}}
\newcommand{\bQ}{\bm{Q}}

\newcommand{\bU}{\bm{U}}
\newcommand{\bT}{\bm{T}}
\newcommand{\bV}{\bm{V}}
\newcommand{\bW}{\bm{W}}

\newcommand{\ba}{\bm{a}}
\newcommand{\bb}{\bm{b}}
\newcommand{\bc}{\bm{c}}
\newcommand{\bg}{\bm{g}}
\newcommand{\be}{\bm{e}}

\newcommand{\bh}{\bm{h}}
\newcommand{\bp}{\bm{p}}

\newcommand{\br}{\bm{r}}
\newcommand{\bt}{\bm{t}}
\newcommand{\bu}{\bm{u}}
\newcommand{\bv}{\bm{v}}
\newcommand{\bx}{\bm{x}}

\newcommand{\bw}{\bm{w}}
\newcommand{\bz}{\bm{z}}

\newcommand{\balpha}{\boldsymbol{\alpha}}
\newcommand{\bepsilon}{\boldsymbol{\epsilon}}
\newcommand{\bveps}{\boldsymbol{\varepsilon}}
\newcommand{\bbeta}{\boldsymbol{\beta}}

\newcommand{\bmu}{\boldsymbol{\mu}}
\newcommand{\bgamma}{\boldsymbol{\gamma}}

\newcommand{\bxi}{\boldsymbol{\xi}}
\newcommand{\bvth}{\boldsymbol{\vartheta}}

\newcommand{\bpsi}{\boldsymbol{\psi}}
\newcommand{\bSigma}{\boldsymbol{\Sigma}}
\newcommand{\bUpsilon}{\boldsymbol{\Upsilon}}

\newcommand{\blambda}{\boldsymbol{\lambda}}
\newcommand{\bLambda}{\boldsymbol{\Lambda}}
\newcommand{\bmeta}{\boldsymbol{\eta}}
\newcommand{\bvrho}{\boldsymbol{\varrho}}

\newcommand{\bpi}{\boldsymbol{\pi}}
\newcommand{\bomega}{\boldsymbol{\omega}}

\newcommand{\ttd}{\mathsf{d}}
\newcommand{\tts}{\mathsf{s}}
\newcommand{\tty}{\mathsf{y}}

\setlength{\parindent}{1em}

\setlength{\bibsep}{0.0pt}

 % I just don't like typing out varepsilon

\setenumerate[1]{label=\bf(\alph*)}

%%%%%%%%%%%%%%%%%%%%%%%%%%%%%

%\renewcommand{\theprop}{SA\arabic{prop}}\setcounter{prop}{0}

%\numberwithin{assumption}{section}
\numberwithin{equation}{section}
\numberwithin{thm}{section}
\numberwithin{lem}{section}
\numberwithin{assumption}{section}
\numberwithin{coro}{thm}

%\renewcommand{\thepart}{SA-\arabic{part}}
%\setcounter{part}{-1}
%\counterwithin{section}{part}
%\renewcommand*\thesection{\thepart.\arabic{section}}
%%%%%%%%%%%%%%%%%%%%%%%%%%%%%
\newcommand{\forloop}[5][1]{\setcounter{#2}{#3}\ifthenelse{#4}{#5\addtocounter{#2}{#1}\forloop[#1]{#2}{\value{#2}}{#4}{#5}}{}}

%%%%%%%%%%%%%%%%%%%
\usepackage{tocloft}
\addtolength{\cftsecnumwidth}{25pt}
\addtolength{\cftsubsecnumwidth}{25pt}
\addtolength{\cftsubsubsecnumwidth}{25pt}
%%%%%%%%%%%%%%%%%%%

\begin{document}

% % % % % % % % % % % % % % Title Page % % % % % % % % % % % % % %
\title{\vspace{-0.25in}\Large Causal Inference in Possibly Nonlinear Factor Models\\
	\medskip
	Supplemental Appendix
\bigskip }
\author{
	Yingjie Feng\thanks{School of Economics and Management, Tsinghua University.}}
\maketitle

%\vspace{-1em}
%\centerline{
%	\href{https://drive.google.com/file/d/1IxNBLhLOnpShBQQTFQsl18nQnkCpPMZo/view?usp=sharing}{\Large click here for the latest version}
%}
\vspace{1em}

\begin{abstract}
This supplement gives omitted theoretical proofs of the results discussed in the main paper, and additional technical results, which may be of independent interest. Section \ref{SA-sec: general LPSA} presents the theory for local principal subspace approximation underlying the analysis in the main paper. Section \ref{SA-sec: setup} sets up a general treatment effects model with noisily measured confounders. Section \ref{SA-sec: example} discusses several typical applications. 
Section \ref{SA-sec: estimation} describes the main estimation procedure. Theoretical results for the main analysis is presented in Section \ref{SA-sec: main results}, and all proofs are given in Section \ref{SA-sec: proofs}.
\end{abstract}

\thispagestyle{empty}
%\textit{Keywords:} nonparametric regression, series methods, linear sieve methods, robust bias correction, uniform inference, tuning parameter selection.

\newpage\tableofcontents

\thispagestyle{empty}
\clearpage

%\doublespacing
\setcounter{page}{1}
\pagestyle{plain}

% % % % % % % % % % % % % % Beginning of the Document % % % % % % % % % % % % % %

\section{Overview}  \label{SA-sec: overview}
This supplemental appendix is organized as follows. Section \ref{SA-sec: general LPSA} presents a general local principal subspace approximation method, which is the key building block of the results in the main paper and may be of independent interest. Specifically, Section \ref{SA-sec: matching} concerns the properties of indirect $K$-nearest neighbors ($K$-NN) matching, and Section \ref{SA-sec: LPCA} studies local principal component analysis (PCA) under a set of high-level conditions. Section \ref{SA-sec: setup} sets up a theoretical framework that accommodates the discussion about incorporating high-rank covariates in Section 5.2 of the main paper. Section \ref{SA-sec: example} discusses several typical applications. Section \ref{SA-sec: estimation} describes the main estimation procedure. Compared with that presented in Section 3 of the main paper, Step 1 (latent variables extraction) takes account of high-rank regressors, and Step 2 (factor-augmented regression) estimates generalized partially linear models based on a local quasi-maximum likelihood method. Section \ref{SA-sec: main results} presents the main theoretical results. 
All proofs are given in Section \ref{SA-sec: proofs}.

%SUMMARIZE and COMPARE RESULTS

\medskip
\subsection{Notation}

\textbf{Latent functions.} For a generic sequence of functions $\{h_t(\cdot)\}_{t=1}^M$ defined on a compact support, let $\nabla^{\ell}\bh_t(\cdot)$ be a vector of $\ell$th-order partial derivatives of $h_t(\cdot)$, and define $\mathscr{D}^{[\kappa]}\bh_t(\cdot)=(\nabla^{0}\bh_t(\cdot)', \cdots, \nabla^{\kappa}\bh_t(\cdot)')'$, i.e., a column vector that stores all partial derivatives of $h_t(\cdot)$ up to order $\kappa\geq 0$. The derivatives on the boundary are understood as limits with the arguments ranging within the support.
When $\ell=1$, $\nabla\bh_t(\cdot):=\nabla^1\bh_t(\cdot)$ is the gradient vector, and the Jacobian matrix is 
$\nabla\bh(\cdot):=(\nabla\bh_1(\cdot), \cdots, \nabla\bh_{M}(\cdot))'$.

\textbf{Matrices.}
Several matrix norms are used throughout the paper. For a vector $\bv\in\mathbb{R}^{\ttd}$, $\|\bv\|_2=\sqrt{\bv'\bv}$ denotes its Euclidean norm. For an $m\times n$ matrix $\bA$, the Frobenius matrix norm is denoted by $\|\bA\|_F=\sqrt{\tr(\bA\bA')}$, %the nuclear norm by $\|\bA\|_*=\sum_{l=1}^{\min\{m,n\}}s_l(\bA)$, 
$L_2$ operator norm by $\|\bA\|_2=s_1(\bA)$, and the entrywise sup-norm by $\|\bA\|_{\max}=\max_{1\leq i\leq m, 1\leq j\leq n}|a_{ij}|$, where $s_l(A)$ denotes the $l$th largest singular value of $\bA$.  To be more explicit, I write $s_{\max}(\bA):=s_1(\bA)$ and $s_{\min}(\bA):=s_{\min\{m,n\}}(\bA)$.  
%For conformable matrices $\bA$ and $\bB$, their inner product is $\langle\mathbf{A}, \mathbf{B}\rangle=\tr(\mathbf{A}'\mathbf{B})$. 
%and  $\dot{\bA}=\bA-\frac{1}{n}\bA\biota_n\biota_n'$ denotes its row-wise demeaned matrix, where $\biota_n$ is an $n$-vector of ones. 
Also, I use $\bA_{i\cdot}$ to denote the $i$th row and $\bA_{\cdot t}$ the $t$th column of $\bA$. More generally, for $\mathcal{C}\subseteq\{1,\cdots,n\}$ and $\mathcal{R}\subseteq\{1,\cdots, m\}$,  $\bA_{\cdot\mathcal{C}}$ denotes the submatrix of $\bA$ with column indices in $\mathcal{C}$, and $\bA_{\mathcal{R}\cdot}$ is the submatrix of $\bA$ with row indices in $\mathcal{R}$.

\textbf{Asymptotics.}
For sequences of numbers or random variables, $a_n\lesssim b_n$ denotes that $\limsup_n|a_n/b_n|$ is finite, and $a_n\lesssim_\P b_n$ or $a_n=O_\P(b_n)$ denotes  $\limsup_{\varepsilon\rightarrow\infty}\limsup_n\P[|a_n/b_n|\geq\varepsilon]=0$. $a_n=o(b_n)$ implies $a_n/b_n\rightarrow 0$, and $a_n=o_\P(b_n)$ implies $a_n/b_n\rightarrow_\P 0$, where $\rightarrow_\P$ denotes convergence in probability. $a_n\asymp b_n$ implies that $a_n\lesssim b_n$ and $b_n\lesssim a_n$, and $a_n\asymp_\P b_n$ implies $a_n\lesssim_\P b_n$ and $b_n\lesssim_\P a_n$. $\rightsquigarrow$ denotes convergence in distribution. For a sequence of random quantities $\{a_{n,i}\}_{i=1}^n$ indexed by $i$, $a_{n,i}$ is said to be $O_\P(b_n)$ (or $o_\P(b_n)$) uniformly over $1\leq i\leq n$, if $\max_{1\leq i\leq n}|a_{n,i}|=O_\P(b_n)$ (or $\max_{1\leq i\leq n}|a_{n,i}|=o_\P(b_n)$). %For two random variables $X$ and $Y$, $X=_d Y$ implies that they have the same probability distribution.
In addition, ``w.p.a. 1'' means ``with probability approaching one''.

\textbf{Others.}
For a sequence of variables $\{w_i\}_{i=1}^n$, I use $\E_n[w_i]=\frac{1}{n}\sum_{i=1}^{n}w_i$ to denote the average. For two numbers $a$ and $b$, $a\vee b=\max\{a,b\}$ and $a\wedge b=\min\{a,b\}$. For a finite set $\mathcal{S}$, $|\mathcal{S}|$ denotes its cardinality.
As mentioned in the main paper, I will consider two choices of distance metrics. Given a sequence of $p$-vectors $\{\bv_i\}_{i=1}^n$, for any $1\leq i,j\leq n$, Euclidean distance is $\mathfrak{d}_2(\bv_i, \bv_j)=\frac{1}{\sqrt{p}}\|\bv_i-\bv_j\|_2$, and
pseudo-max distance is  
$\mathfrak{d}_\infty(\bv_i, \bv_j)=\max_{\ell\neq i, j} |\frac{1}{p}(\bv_i-\bv_j)'\bv_\ell|$.

%%%%%%%%%%%%%%%%%%%%%%%%%%%%%%%%%%%%%%%%%%%%%%%%%%%%%%%%%%%%%%%%%%%%%%%%%
\section{Local Principal Subspace Approximation}\label{SA-sec: general LPSA}

This section discusses the general local principal subspace approximation procedure. The main results can be applied to any variable with a nonlinear factor structure, including the large-dimensional covariates $\{\bx_{i}\}_{i=1}^n$ and $\{\bw_{i,\ell}\}_{i=1}^n$ for $\ell=1,\ldots, \ttd_w$ used in the main paper. 

To reflect this generality and make this section self-contained, I first introduce more notation. Specifically, let $\ba\in\mathbb{R}^p$ be a (large-dimensional) random variable of interest. A random sample $\{\ba_{i}\}_{i=1}^n$ is available, which is i.i.d across $1\leq i\leq n$ and stored in a $p\times n$ data matrix $\bA=(\ba_1,\cdots, \ba_n)$. $\ba_i=(a_{i1},\cdots,a_{ip})$ admits a pure nonlinear factor structure:
\begin{equation} \label{SA-eq: pure nonlinear factor}
a_{it}=\mu_{t,A}(\bxi_i)+\varepsilon_{it}, \qquad \E[\varepsilon_{it}|\mathcal{F}_A]=0,
\end{equation} 
where $\{\bxi_i\}_{i=1}^n$ is i.i.d over a compact support $\mathcal{X}_\xi\subseteq\mathbb{R}^{\ttd_\xi}$ and $\mathcal{F}_A$ is the $\sigma$-field generated by $\{\bxi_i\}_{i=1}^n$ and $\{\mu_{t,A}(\cdot)\}_{t=1}^p$. Define $p\times n$ matrices $\bL$ and  $\bveps$ with their $(t,i)$th entry given by $\mu_{t,A}(\bxi_i)$ and  $\varepsilon_{it}$ respectively. Write $\bmu_A(\cdot)=(\mu_{1,A}(\cdot), \cdots, \mu_{p,A}(\cdot))'$, and recall that
\[
\nabla\bmu_{t,A}(\bxi)=\Big(\frac{\partial\mu_{t,A}(\bxi)}{\partial\xi_1}, \cdots, \frac{\partial\mu_{t,A}(\bxi)}{\partial\xi_{\ttd_\xi}}\Big)' 
\quad\text{and}\quad
\nabla\bmu_{A}(\bxi)=\Big(\nabla\bmu_{1,A}(\bxi), \cdots, \nabla\bmu_{p, A}(\bxi)\Big)'.
\]

The analysis in the following will be further decomposed into two subsections, one for indirect matching and the other for local principal component analysis.
I will use a row-wise sample splitting scheme to separate the two steps. For simplicity, I assume $p=2T$ and randomly split row indices of $\bA$ into two subsets $\mathcal{T}_1$ and $\mathcal{T}_2$ with $|\mathcal{T}_1|=|\mathcal{T}_2|=T$.  Define  $\bA^{\dagger}=\bA_{\mathcal{T}_1\cdot}$, which is used for matching, and $\bA^{\ddagger}=\bA_{\mathcal{T}_2\cdot}$, which is used for local principal component analysis.
$\bL^{\dagger}$, $\bL^{\ddagger}$, $\bveps^{\dagger}$ and $\bveps^{\ddagger}$ are defined similarly. Thus, the superscripts $\dagger$ and $\ddagger$ denote that a quantity is defined on $\mathcal{T}_1$ and $\mathcal{T}_2$ respectively.

Next, recall that Assumptions 3, 4 and 5 in the main paper impose key geometric conditions on the nonlinear manifold generated by latent functions. For convenience of later expressions, I restate them as definitions applied to the generic sequence of random functions $\{\mu_{t,A}(\cdot)\}_{t\in\mathcal{T}^\sharp}$ and random variables $\{\bxi_i\}_{i=1}^n$ for a subset of indices $\mathcal{T}^\sharp\subseteq\{1,\cdots, T\}$ with   $T^\sharp=|\mathcal{T}^\sharp|$. Let $\bmu_{A}^\sharp(\cdot)=(\mu_{t,A}(\cdot))_{t\in\mathcal{T}^\sharp}$ be a $T^\sharp\times 1$ column vector of functions.

\begin{definition} \label{SA-Definition: nonsingularity}
	The sequence of random functions $\{\mu_{t,A}(\cdot)\}_{t\in\mathcal{T}^\sharp}$ evaluated on $\{\bxi_i\}_{i=1}^n$ is said to be \textit{asymptotically nonsingular} with respect to a distance metric $\mathfrak{d}(\cdot,\cdot)$ if for every $\epsilon>0$,
	\begin{equation}\label{eq: def of nonsingularity}
	\lim_{\Delta\rightarrow 0}\limsup_{n,T^\sharp\rightarrow\infty}\;
	\P\Big\{\max_{1\leq i\leq n}\;
	\max_{j:\mathfrak{d}(\bmu_{A}^\sharp(\bxi_i),\bmu_{A}^\sharp(\bxi_j))<\Delta}\;
	\|\bxi_i-\bxi_j\|_2>\epsilon\Big\}=0.
	\end{equation}
\end{definition}

\begin{definition} \label{SA-Definition: non-degenerate}
	The sequence of functions $\{\mu_{t,A}(\cdot)\}_{t\in\mathcal{T}^\sharp}$ evaluated on $\{\bxi_i\}_{i=1}^n$ is said to be \textit{asymptotically non-degenerate} up to order $\kappa\geq 0$ if for some $\underline{c}>0$,
	\begin{equation}\label{eq: def of nondegenerate to order kappa}
	\lim_{n,T^\sharp\rightarrow\infty}\;\P\Big\{
	\min_{1\leq i\leq n}s_{\min}\Big(\frac{1}{T^\sharp}\sum_{t\in\mathcal{T}^\sharp}
	(\mathscr{D}^{[\kappa]}\bmu_{t,A}(\bxi_i))(\mathscr{D}^{[\kappa]}\bmu_{t,A}(\bxi_i))'\Big)\geq\underline{c}\Big\}=1,
	\end{equation}
	provided all such derivatives exist.	
\end{definition}

Let $\mathscr{P}_{\bxi_0}[\cdot]$ be the projection operator onto the $\ttd_\xi$-dimensional space (embedded in $\mathbb{R}^{T^\sharp}$) spanned by the local tangent basis $\nabla\bmu_A^\sharp(\bxi_0)$ at $\bmu_A^\sharp(\bxi_0)$. Take an orthogonalized basis of this tangent space, and denote by $\mathscr{P}_{\bxi_0,j}[\cdot]$ the projection operator onto the $j$th direction of the tangent space. 

\begin{definition} \label{SA-Definition: non-collapsing}
	The sequence of functions $\{\mu_{t,A}(\cdot)\}_{t\in\mathcal{T}^\sharp}$ evaluated on $\{\bxi_i\}_{i=1}^n$ is said to be \textit{asymptotically non-collapsing} if 
	there exists an absolute constant $\underline{c}'>0$ such that
	\begin{equation}\label{eq: def of non-collapsing}
	\lim_{n,T^\sharp\rightarrow\infty}\;
	\P\Big\{
	\min_{1\leq \ell\leq \ttd_\xi}
	\min_{1\leq i\leq n}
	\sup_{\bxi\in\mathcal{X}_\xi}
	\frac{1}{T^\sharp}\Big\|\mathscr{P}_{\bxi_i,\ell}[\bmu^\sharp(\bxi)]\Big\|_2^2\geq \underline{c}'\Big\}=1,
	\end{equation}
	provided that the projectors $\mathscr{P}_{\bxi_i,\ell}[\cdot]$ are well defined.
\end{definition}

%%%%%%%%%%%%%%%%%%%%%%%%%%%%%%%%%%%%%%%%%%%%%%%%%%%

\subsection{Indirect Matching} \label{SA-sec: matching}

This section analyzes the discrepancy of latent variables induced by $K$-NN matching. Its validity relies on the following conditions.

\begin{assumption}[Indirect Matching] 
	\label{SA Assumption: Matching}\leavevmode
	\begin{enumerate}[label=(\alph*)]
		\item 
		$\{\bxi_i\}_{i=1}^n$ is i.i.d over a compact convex support with densities bounded and bounded away from zero;
		
		\item $\{\mu_{t,A}(\cdot)\}_{t=1}^T$ is $\bar{m}$-times continuously differentiable for some $\bar{m}\geq 2$ with all partial derivatives of order no greater than $\bar{m}$ bounded by a universal constant;
		%$\|\nabla^{\kappa}\mu_{t,A}(\bxi)\|_{\max}\lesssim 1$ for all $\bxi\in\mathcal{X}_\xi$ and $\kappa\leq \bar{m}$;
		
		\item $\{\varepsilon_{it}:1\leq i\leq n,1\leq t\leq p\}$ is independent over $i$ and $t$ conditional on $\mathcal{F}_A$, and 
		for some $\nu>0$,
		$\max_{1\leq i\leq n,1\leq t\leq p}\E[|\varepsilon_{it}|^{2+\nu}|\mathcal{F}_A]<\infty$  a.s. on $\mathcal{F}_A$;
		
		\item $\{\mu_{t,A}(\cdot)\}_{t\in\mathcal{T}_1}$ is asymptotically nonsingular with respect to a distance metric $\mathfrak{d}(\cdot,\cdot)$ and non-degenerate up to order $1$;
				
		\item $\{\mu_{t,A}(\cdot)\}_{t\in\mathcal{T}_1}$ is asymptotically non-collapsing.
	\end{enumerate}
\end{assumption}

I first derive a bound for the direct matching discrepancy of latent variables when $K$ is large. Specifically, for any fixed point $\bxi_0\in\mathcal{X}_{\xi}$, let  $\mathcal{N}_{\bxi_0}^*=\{j_k^*(\bxi_0):1\leq k\leq K\}$ denote the set of indices for the $K$ nearest neighbors of $\bxi_0$ in terms of the Euclidean distance. The ordering of $\{j_1^*(\bxi_0), \cdots, j_K^*(\bxi_0)\}$ is based on that of the original sequence $\{\bxi_i\}_{i=1}^n$ rather than the closeness to $\bxi_0$.

\begin{lem} \label{lem: direct matching}
	Suppose that Assumption \ref{SA Assumption: Matching}(a) holds. If $\log (n/K)/K=o(1)$
	and $K\log n/n=o(1)$, then for some absolute constants $c,C>0$, 
	\[
	c(K/n)^{\frac{1}{\ttd_\xi}}\leq\inf_{\bxi_0\in\mathcal{X}_\xi}\max_{1\leq k\leq K}\|\bxi_{j_k^*(\bxi_0)}-\bxi_0\|_2
	\leq \sup_{\bxi_0\in\mathcal{X}_\xi}\max_{1\leq k\leq K}\|\bxi_{j_k^*(\bxi_0)}-\bxi_0\|_2
	\leq C(K/n)^{\frac{1}{\ttd_\xi}},\;
	\text{w.p.a.} 1.
	\]
\end{lem}

%Now, consider the implicit discrepancy induced by $K$-NN matching on the observed $\{\bA^\dagger_{\cdot j}\}_{j=1}^n$. 
Let $\mathcal{N}_i=\{j_k(i): k=1, \ldots, K\}$ be a set of indices for the $K$ nearest neighbors of unit $i$ in terms of the distance $\mathfrak{d}(\bA^{\dagger}_{\cdot i}, \bA^{\dagger}_{\cdot j})$ for $j=1,\cdots, n$, where $\mathfrak{d}(\cdot, \cdot)$ is a metric specified by users. Again, $\{j_1(i), \cdots, j_K(i)\}$ is arranged according to the original ordering of $\{\bA^{\dagger}_{\cdot j}\}_{j=1}^n$. 
The next lemma shows that there exists a lower bound on the maximum (Euclidean) distance between $\bxi_i$ and $\bxi_j$ for $j\in \mathcal{N}_i$. %It immediately follows by definition of nearest neighbors.

\begin{lem} \label{lem: matching discrepancy lower bound}
	Under the conditions of Lemma \ref{lem: direct matching}, there exists an absolute constant $c>0$,
	\[
	\min_{1\leq i\leq n}\max_{1\leq k\leq K} \|\bxi_i-\bxi_{j_k(i)}\|_2\geq 
	c(K/n)^{\frac{1}{\ttd_\xi}}, \; \text{w.p.a.} 1.
	\]
\end{lem}

The next theorem constructs an upper bound on the implicit matching discrepancy.

\begin{thm}[Indirect Matching: Homoskedasticity] \label{thm: IMD hom}
   Let $\mathfrak{d}(\cdot, \cdot)=\mathfrak{d}_2(\cdot, \cdot)$. Suppose that Assumption \ref{SA Assumption: Matching}(a)-(d) hold. In addition, assume that  $\frac{1}{T}\sum_{t\in\mathcal{T}_1}\E[\varepsilon_{it}^2|\mathcal{F}_A]=\sigma^2$ for all $1\leq i\leq n$ and $\max_{1\leq i\leq n,1\leq t\leq p}\E[|\varepsilon_{it}|^{4+2\nu}|\mathcal{F}_A]<\infty$  a.s. on $\mathcal{F}_A$.  If $\frac{n^{\frac{4}{\nu}}(\log n)^{\frac{\nu-2}{\nu}}}{T}\lesssim 1$, then
   \[
   \max_{1\leq i\leq n}\max_{1\leq k\leq K}
   \|\bxi_i-\bxi_{j_k(i)}\|_2
   \lesssim_\P (K/n)^{\frac{1}{\ttd_\xi}}+(\log n/T)^{\frac{1}{4}}.%=:h_{K,\xi}^2.
   \]
\end{thm}

The condition in this theorem is stringent since conditional heteroskedasticity of $\varepsilon_{it}$ across $i$ is excluded. Using the distance metric $\mathfrak{d}_\infty(\cdot, \cdot)$ helps avoid this restriction.

\begin{thm}[Indirect Matching: Heteroskedasticity] \label{thm: IMD hsk}
	Let $\mathfrak{d}(\cdot, \cdot)=\mathfrak{d}_\infty(\cdot, \cdot)$. Suppose that Assumption \ref{SA Assumption: Matching}(a)-(d) hold. 
	If $\frac{n^{\frac{4}{\nu}}(\log n)^{\frac{\nu-2}{\nu}}}{T}\lesssim 1$. Then,
	\[
	\max_{1\leq i\leq n}\max_{1\leq k\leq K}
	\|\bxi_i-\bxi_{j_k(i)}\|_2
	\lesssim_\P (K/n)^{\frac{1}{2\ttd_\xi}}+(\log n/T)^{\frac{1}{4}}.%=:h_{K,\xi}^2.
	\]
	If Assumption \ref{SA Assumption: Matching}(e) also holds, then 
	\[
	\max_{1\leq i\leq n}\max_{1\leq k\leq K}
	\|\bxi_i-\bxi_{j_k(i)}\|_2
	\lesssim_\P (K/n)^{\frac{1}{\ttd_\xi}}+(\log n/T)^{\frac{1}{2}}.%=:h_{K,\xi}.
	\]
\end{thm}

\begin{remark}
	Assumption \ref{SA Assumption: Matching}(e) is the key to understanding the improved error rate in the second result of Theorem \ref{thm: IMD hsk}.
	Intuitively, it ensures that the manifold generated by $\{\mu_{t,A}(\cdot)\}_{t\in\mathcal{T}_1}$ does not lose dimensionality when projected onto a tangent space at any point. To see how the improvement arises, note an intermediate result in the proof of Lemma \ref{thm: IMD hsk}:
	\[
	\max_{1\leq i\leq n}\max_{1\leq k\leq K}\max_{\ell\neq i, j_k(i)}
	\Big|\frac{1}{T}(\bL^{\dagger}_{\cdot i}-\bL^{\dagger}_{\cdot j_k(i)})'\bL^{\dagger}_{\cdot\ell}\Big|\lesssim_\P (K/n)^{1/\ttd_\xi}+\sqrt{\log n/T}.
	\]
	$\bL^{\dagger}_{\cdot i}-\bL^{\dagger}_{\cdot j_k(i)}$ approximately lies on the tangent space at unit $i$. If we can choose a particular unit $\ell'$ such that it is not too orthogonal to this tangent space and its magnitude is not too small, then a bound on their inner product translates to that for the difference between unit $i$ and $j_k(i)$ without an additional penalty. 
\end{remark}

Before closing this subsection, I give two useful lemmas concerning the distributional feature of the matched sample and the maximum number of times a unit used for matching.

\begin{lem} \label{lem: conditional independence of KNN}
	Let $\widehat{R}_i=\max_{1\leq k\leq K} \mathfrak{d}(\bA^{\dagger}_{\cdot i}, \bA^{\dagger}_{\cdot j_k(i)})$ for $\mathfrak{d}(\cdot, \cdot)=\mathfrak{d}_2(\cdot, \cdot)$, or $\mathfrak{d}_\infty(\cdot, \cdot)$.
	Under Assumption \ref{SA Assumption: Matching}, $\{\bxi_{j_k(i)}\}_{k=1}^K$ is independent conditional on $\widehat{R}_i$ and $\bA^{\dagger}_{\cdot i}$.
\end{lem}

\begin{remark}
	In the proof of Lemma \ref{lem: conditional independence of KNN}, I describe the form of the conditional joint density of these nearest neighbors. Compared with that for the nearest neighbors based on direct matching on $\bxi_i$, the existence of errors leads to an additional adjustment factor $\P(\mathcal{S}_{\widehat{R}_i}|\bxi_k):=\int f_{A|\xi}(\ba_k|\bv_k)\I(\ba_k\in \mathcal{S}_{\widehat{R}_i})d\ba_k$, where $f_{A|\xi}(\cdot|\cdot)$ is the conditional density of $\bA^{\dagger}_{\cdot j}$ given $\bxi_j$ and  $\mathcal{S}_{\widehat{R}_i}=\{\bz: \mathfrak{d}(\bz, \bA^{\dagger}_{\cdot i})<\widehat{R}_i\}$.  The effect of such adjustment reflects the fact that the indirect matching may allow for inclusion of some units with $\bxi_j$'s very far away from $\bxi_i$ or exclusion of some very close to $\bxi_i$. Despite this fact, in view of Lemma \ref{lem: matching discrepancy lower bound}, Theorem \ref{thm: IMD hom} and Theorem \ref{thm: IMD hsk}, the probability of such misclassification should be small if their distance goes beyond a range proportional to $T^{-1/4}$ or $T^{-1/2}$ up to a log penalty. 
\end{remark}

\begin{lem}\label{lem: number of times for matching}
	For each unit $i$, let $S_K(i)=\sum_{j=1}^n\I(i\in\mathcal{N}_j)$ be the number of times unit $i$ is used for matching. Consider the following two cases:
	\begin{enumerate}[label=(\roman*)]
		\item If the conditions in Theorem \ref{thm: IMD hom} hold, then assume $(K/n)^{1/\ttd_\xi}\gtrsim (\log n/T)^{1/4}$;
		\item If the conditions in Theorem \ref{thm: IMD hsk} hold, then assume $(K/n)^{1/\ttd_\xi}\gtrsim(\log n/T)^{1/2}$.
	\end{enumerate}
Then,	$\max_{1\leq i\leq n}S_K(i)\lesssim_\P K$.
\end{lem}

%%%%%%%%%%%%%%%%%%%%%%%%%%%%%%%%%%%%%%%%%%%%

\subsection{Local Principal Component Analysis} \label{SA-sec: LPCA}

This subsection considers the properties of local PCA. As mentioned before, row-wise sample splitting is used to separate the matching and PCA steps. 
Throughout this subsection, I assume that the local neighborhood $\mathcal{N}_i$ for each $i$ has been obtained using $\bA^\dagger$, and then local PCA is implemented using $\bA^\ddagger$.

\subsubsection{Local Factor Structure}
\label{SA-subsec: local factor structure}
%The matching technique analyzed in the previous section implicitly selects a \textit{bandwidth} reflected by the matching discrepancy, though the unobservability of latent variables restricts the range of bandwidths one may choose from. In contrast, in classical nonparametric kernel-based estimation, users have complete freedom of bandwidth selection, e.g., oversmoothing or undersmoothing. 

%The results in the previous section suffices for local constant smoothing. To implement higher-order approximation, 

Formally, define a vector-valued function 
$$\bxi\in\mathcal{X}_\xi\mapsto\blambda(\bxi):=(\lambda_1(\bxi), \ldots, \lambda_{\ttd_\lambda}(\bxi))',$$ 
which plays the role of a linear approximation basis. Accordingly, 
\[
\bLambda_{\subi}=\Big(\blambda_{j_1(i)}, \cdots, \blambda_{j_K(i)}\Big)',\quad
\bF_{\subi}=\E_{\mathcal{N}_i}[\bL_{\subi}\bLambda_{\subi}]\E_{\mathcal{N}_i}[\bLambda_{\subi}'\bLambda_{\subi}]^{-1},
\]
where $\blambda_{j_k(i)}=\blambda(\bxi_{j_k(i)})$ and $\bL_{\subi}=(\bL^{\ddagger}_{\cdot j_1(i)},\cdots, \bL^{\ddagger}_{\cdot j_K(i)})$.
Recall that the $T\times n$ matrix $\bL^{\ddagger}$ denotes the submatrix of $\bL$ with row indices in $\mathcal{T}_2$ and $\bL^{\ddagger}_{\cdot j}$ is the $j$th column of $\bL^{\ddagger}$. The subscript $\subi$ of these quantities indicates that they are defined based on the $K$ nearest neighbors of unit $i$.
Also,  $\E_{\mathcal{N}_i}[\cdot]$ denotes an expectation operator conditional  on $\widehat{R}_i$ (or the information used in matching).
Now, define the following local principal component decomposition around unit $i$:
\begin{equation}\label{eq: LPCA}
\begin{split}
&\bA_{\subi}=\bF_{\subi}\bLambda_{\subi}'+\br_{\subi}+\bveps_{\subi},
\quad \text{where}\\
&\bA_{\subi}=(\bA^{\ddagger}_{\cdot j_1(i)}, \cdots, \bA^{\ddagger}_{\cdot j_K(i)}),\quad
\bveps_{\subi}=(\bveps^{\ddagger}_{\cdot j_1(i)}, \cdots, \bveps^{\ddagger}_{\cdot j_K(i)}).
\end{split}
\end{equation} 
The linear factor structure $\bF_{\subi}\bLambda_{\subi}'$ forms a local approximation subspace for the underlying nonlinear manifold, and $\br_{\subi}$ is the resultant approximation error. From now on, the $T\times \ttd_\lambda$ matrix $\bF_{\subi}$ will be referred to as the \textit{factor} and the $K\times \ttd_\lambda$ matrix $\bLambda_{\subi}$ is the \textit{loading}. By definition, the linear factor component can be viewed as the $L_2$ projection of the unknown function $\bmu_{A}(\cdot)$ onto the space spanned by $\blambda(\cdot)$, and therefore, $\br_{\subi}$ is the $L_2$ projection error. 

Equation \eqref{eq: LPCA} is simply a representation. In fact, the approximation subspace is not unique, and neither $\bF_{\subi}$ nor $\bLambda_{\subi}$ can be identified without further restrictions. Also, the number of approximation terms governed by the number of principal components differentiated from noise and different choices of approximation bases impact the approximation power reflected by the magnitude of $\br_{\subi}$.
%As a simple illustration, one may let $\blambda(\cdot)$ be a linear basis: $\blambda(\bxi)=(1, (\bxi-\bxi_i)')'$. Then, the decomposition \eqref{eq: LPCA} is similar to the first step of local tangent space alignment (LTSA, \citealp{Zhang-Zha_2004_SIAM}). %Also note that when the latent variables are known, the above approximation is identical to local linear regression with a uniform kernel. 

If the approximation error $\br_{\subi}$ is ignored, 
Equation \eqref{eq: LPCA} can be viewed as a (localized) linear factor model. An important distinguishing feature is that the factor loadings in $\bLambda_{\subi}$ are of different magnitude. If more factors (higher-order approximation functions) are included, they get \textit{weaker} in the sense that their loadings are asymptotically approaching zero. 

For each neighborhood $\mathcal{N}_i$, extract leading $\ttd_\lambda$ eigenvectors:
\[
\frac{1}{TK}\bA_{\subi}\bA_{\subi}'\widehat{\bF}_{\subi}=\widehat{\bF}_{\subi}\widehat{\bV}_{\subi}
\]
where $\widehat{\bF}_{\subi}$ satisfies  $\frac{1}{T}\widehat{\bF}_{\subi}'\widehat{\bF}_{\subi}=\bI_{\ttd_\lambda}$ and $\widehat\bV_{\subi}=\diag\{\widehat{v}_{1,\subi}, \cdots, \widehat{v}_{\ttd_\lambda,\subi}\}$ is a diagonal matrix with $\ttd_\lambda$ leading eigenvalues $\widehat{v}_{1,\subi}\geq \cdots\geq\widehat{v}_{\ttd_\lambda,\subi}$ on the diagonal. Accordingly, for $1\leq j\leq \ttd_\lambda$, let $v_{j,\subi}$ denote the $j$th eigenvalue of $\frac{1}{TK}\bF_{\subi}\bLambda_{\subi}'\bLambda_{\subi}\bF_{\subi}'$.
The estimated factor loading is given by
$\widehat{\bLambda}_{\subi}=\frac{1}{T}\bA_{\subi}'\widehat{\bF}_{\subi}$.
They are merely scaled right singular vectors of $\bA_{\subi}$, or equivalently, the leading $\ttd_{\lambda}$ eigenvectors of $\frac{1}{TK}\bA_{\subi}'\bA_{\subi}$ such that   $\frac{1}{K}\widehat{\bLambda}_{\subi}'\widehat{\bLambda}_{\subi}=\widehat{\bV}_{\subi}$. The estimated factor component then is given by $\widehat{\bL}_{\subi}=\widehat{\bF}_{\subi}\widehat{\bLambda}_{\subi}'$. %Note that as discussed in the main paper, the PCA procedure implicitly corresponds to particular choices to $\bF_{\subi}$ and $\bLambda_{\subi}$ in Equation \eqref{eq: LPCA}.

\bigskip

\textbf{Notation:} Since the eigenstructure in this problem involves factors of different strength, more notation is introduced for ease of presentation.
First, partition $\ttd_\lambda$ leading approximation terms into $m$ groups, which is identical to a partition of index set: $\{1,\cdots, \ttd_\lambda\}=\cup_{\ell=0}^{m-1}\mathcal{C}_\ell$ with $|\mathcal{C}_\ell|=\ttd_{\lambda,\ell}$, where $\mathcal{C}_\ell$ corresponds to the polynomial basis of degree $\ell$. To properly normalize the basis, define $\bUpsilon=\diag\{\bI_{\ttd_{\lambda,0}},\; h_{K,\xi}\bI_{\ttd_{\lambda,1}},\;\cdots,\; h_{K,\xi}^{m-1}\bI_{\ttd_{\lambda,m-1}}\}$ where $h_{K,\xi}=(K/n)^{1/\ttd_\xi}$. Then, partition the eigenvalues and eigenvectors accordingly. Following the notation set up at the beginning of this supplement, for any generic $p\times \ttd_\lambda$ matrix $\bG_{\subi}$ (defined locally for unit $i$), $\bG_{\gr{\ell},\subi}$ denotes the submatrix of $\bG_{\subi}$ with column indices in $\mathcal{C}_\ell$. For example, $\bF_{\gr{0},\subi}$ denotes the first $\ttd_{\lambda,0}$ columns of $\bF_{\subi}$. I also denote by $\bff_{t,\subi}'$ (and $\widehat{\bff}_{t,\subi}'$) the $t$th row of $\bF_{\subi}$ (and $\widehat{\bF}_{\subi}$). 
Moreover, let $\delta_{KT}=(K^{1/2}\wedge T^{1/2})/\sqrt{\log (n\vee T)}$, and for a generic matrix $\bG$, $\bP_{\bG}$ and $\bM_{\bG}$ denote the projection matrices onto the column space of $\bG$ and its orthogonal complement respectively.

\subsubsection{Results}

The main analysis of this section is based on the following high-level condition.

\begin{assumption}[Local Approximation] \label{SA Assumption: LPCA}
	$\bA_{\subi}$ admits Decomposition \eqref{eq: LPCA} and the following conditions hold:
	\begin{enumerate}[label=(\alph*)]
		\item 
		$\max_{1\leq i\leq n}\|\bLambda_{\subi}\bUpsilon^{-1}\|_{\max}\lesssim_\P1$ and 
		\[
		1\lesssim_\P \min_{1\leq i\leq n}s_{\min}\Big(\frac{1}{K}\bUpsilon^{-1}\bLambda_{\subi}'\bLambda_{\subi}\bUpsilon^{-1}\Big)\leq
		\max_{1\leq i\leq n}s_{\max}\Big(\frac{1}{K}\bUpsilon^{-1}\bLambda_{\subi}'\bLambda_{\subi}\bUpsilon^{-1}\Big)\lesssim_\P 1;
		\]

	    \item $1\lesssim_\P\min_{1\leq i\leq n}s_{\min}\Big(\frac{1}{T}\bF_{\subi}'\bF_{\subi}\Big)\leq
	    \max_{1\leq i\leq n}s_{\max}\Big(\frac{1}{T}\bF_{\subi}'\bF_{\subi}\Big)\lesssim_\P 1$; 
	    
	    \item There exists some $m\leq\bar{m}$ such that 
	     $\max_{1\leq i\leq n}\|\br_{\subi}\|_{\max}\lesssim_\P h_{K,\xi}^m$ and $\delta_{KT}^{-1}/h_{K,\xi}^{m-1}=o(1)$.
    \end{enumerate}
\end{assumption}
\begin{remark}
	Part (a) imposes \textit{heterogeneous} bounds on factor loadings and requires that the loading matrix be non-degenerate with proper normalization. 
    Part (b) implies that there indeed exist $\ttd_\lambda$ leading approximation factors. Part (c) specifies to what extent PCA approach may remove the potential smoothing bias, where the rate condition links the effective sample size $\delta_{KT}$ and bandwidth $h_{K,\xi}$.
    These conditions, by nature, is high-level and can be justified under more primitive conditions, as shown in Lemma \ref{lem: verify SA LPCA}.
    
    It should be noted that in high-dimensional linear factor analysis, the so-called \textit{semi-strong} factor models impose similar conditions. The name implies that the strength of factors may be heterogeneous but still stronger than noise. In this sense, the results derived below may be easily applied to such models with minor changes.
  \end{remark}

Before moving onto the main analysis, I first verify Assumption \ref{SA Assumption: LPCA} under more primitive conditions. The following lemma is one example, which motivates the lower-level conditions used in the main paper and Section \ref{SA-sec: main results} of this supplement.

\begin{lem}[Verification of Assumption \ref{SA Assumption: LPCA}]\label{lem: verify SA LPCA}
	Suppose that Assumption \ref{SA Assumption: Matching} holds with $\mathfrak{d}(\cdot,\cdot)=\mathfrak{d}_\infty(\cdot,\cdot)$, $\{\mu_{t,A}(\cdot)\}_{t\in\mathcal{T}_2}$ is nondegenerate up to order $m-1$ (see Definition \ref{SA-Definition: non-degenerate}) for some $2\leq m\leq \bar{m}$, $\delta_{KT}^{-1}=o(1)$ and $\delta_{KT}^{-1}/h_{K,\xi}^{m-1}=o(1)$. 
	%Consider the following two cases:
	%(i) when the conditions in Theorem \ref{thm: IMD hom} hold,  assume $(K/n)^{1/\ttd_\xi}\gtrsim (\log n/T)^{1/4}$;
    %(ii) when the conditions in Theorem \ref{thm: IMD hsk} hold, assume %$(K/n)^{1/\ttd_\xi}\gtrsim(\log n/T)^{1/2}$.
	Then, Assumption \ref{SA Assumption: LPCA} is satisfied by setting  $\mathsf{d}_\lambda=\binom{m-1+\ttd_\xi}{\ttd_\xi}$. As a result, $v_{j,\subi}\asymp_\P\Upsilon_{jj}$ for each $j=1,\cdots, \mathsf{d}_\lambda$.
\end{lem}

On the other hand, a bound on the operator norm of the error matrix is given by the following lemma based on the assumption imposed in this paper.

\begin{lem}[Operator Norm of Errors] \label{lem: operator norm of eps}
	Under Assumption \ref{SA Assumption: Matching}, if $\frac{n^{\frac{4}{\nu}}(\log n)^{\frac{\nu-2}{\nu}}}{T}\lesssim 1$, then
	\[
	\max_{1\leq i\leq n}\|\bveps_{\subi}\|_2\lesssim_\P\sqrt{K
	}+\sqrt{T\log (n\vee T)}.
	\]
\end{lem}

With these preparations, I am ready to study the estimated eigenstructure. I begin with the analysis of leading terms.

\begin{lem} \label{lem: eigenstructure 1st order}
	Under Assumptions \ref{SA Assumption: Matching} and \ref{SA Assumption: LPCA}, if $\delta_{KT}h_{K,\xi}^{m-1}\rightarrow\infty$,  $\frac{n^{\frac{4}{\nu}}(\log n)^{\frac{\nu-2}{\nu}}}{T}\lesssim 1$ and 
	$\frac{(nT)^{\frac{2}{\nu}}(\log (n\vee T))^{\frac{\nu-2}{\nu}}}{K}\lesssim 1$, 
	then 
	(i) $\max_{1\leq i\leq n}|\widehat{v}_{j,\subi}/v_{j,\subi}-1|=o_\P(1)$, for $1\leq j\leq \ttd_{\lambda,0}$; 
	(ii) there exists a matrix $\tilde{\bH}_{\subi}$ such that
	$\max_{1\leq i\leq n}\frac{1}{\sqrt{T}}\|\widehat{\bF}_{\gr{1},\subi}-\bF_{\subi}\tilde{\bH}_{\gr{1},\subi}\|_F\lesssim_\P \delta_{KT}^{-1}+h_{K,\xi}^{2m}$; 
	and (iii) $\max_{1\leq i\leq n}\|\bM_{\widehat{\bF}_{\gr{1},\subi}}-\bM_{\bF_{\gr{1},\subi}}\|_F\lesssim_\P\delta_{KT}^{-1}+h_{K,\xi}^2$.
\end{lem}

%Once consistency of the estimated leading eigenstructure is established, we may further consider the eigenvalues and eigenvectors in the second-order approximation, if the remaining bias is still of greater magnitude compared with the  errors. %Recall that the second-order approximation contains $\ttd_{\lambda,2}$ terms (apart from the $\ttd_\xi$ first-order terms). 
To extend these results  to higher-order terms in the eigenstructure, I exploit the fact that for any $1\leq j\leq \ttd_\lambda$, the $j$th eigenvalue is
\[
\widehat{v}_{j,\subi}=
\max_{\bv\in\mathbb{R}^{T}: \|\bv\|_2=1 \atop\bv'\widehat{\bF}_{1:(j-1),\subi}=0}\quad \frac{1}{TK}\bv'\bA_{\subi}\bA_{\subi}'\bv=
\max_{\bv\in\mathbb{R}^{T}:\|\bv\|_2=1}\quad \frac{1}{TK}\bv'\bM_{\widehat{\bF}_{1:(j-1),\subi}}\bA_{\subi}\bA_{\subi}'\bM_{\widehat{\bF}_{1:(j-1),\subi}}\bv,
\]
where $\widehat{\bF}_{1:(j-1),\subi}$ denotes $1$ to $(j-1)$ columns of $\widehat{\bF}_{\subi}$. 
General results concerning the estimated eigenvalues and factors are presented in the next theorem.

\begin{thm}\label{thm: consistency eigenstructure}
	Under Assumptions \ref{SA Assumption: Matching} and \ref{SA Assumption: LPCA}, if $\delta_{KT}h_{K,\xi}^{m-1}\rightarrow\infty$, $\frac{n^{\frac{4}{\nu}}(\log n)^{\frac{\nu-2}{\nu}}}{T}\lesssim 1$ and 
	$\frac{(nT)^{\frac{2}{\nu}}(\log (n\vee T))^{\frac{\nu-2}{\nu}}}{K}\lesssim 1$, then for $j=1, \ldots, \mathsf{d}_\lambda$, 
	(i) $\max_{1\leq i\leq n}|\widehat{v}_{j,\subi}/v_{j,\subi}-1|=o_\P(1)$;
	and (ii) there exists some $\check{\bH}_{\subi}$ such that $\max_{1\leq i\leq n}\frac{1}{\sqrt{T}}\|\widehat{\bF}_{\cdot j,\subi}-\bF_{\subi}\check{\bH}_{\cdot j,\subi}\|_2\lesssim_\P
	\delta_{KT}^{-1}\Upsilon_{jj}^{-1}+h_{K,\xi}^{2m}\Upsilon_{jj}^{-2}$. 
\end{thm}

Since the estimated factor loadings are simply eigenvectors of $\frac{1}{TK}\bA'\bA$, the analysis of $\widehat{\bF}_{\subi}$ may also be applied to  $\widehat{\bLambda}_{\subi}$ with a proper rescaling. %Specifically, it can be shown that under the same conditions there exists some rotation matrix $\check{\bH}_{\subi}$ $\frac{1}{K}\|\widehat{\bLambda}_{:j,\subi}-\bLambda_{\subi}\check{\bH}_{:j,\subi}\|_2\lesssim_\P
%\delta_{KT}^{-1}+h_K^{2m}v_{j,\subi}^{-1/2}.$

The above result shows the convergence of the estimated factors in the mean squared error sense. It is neither pointwise nor uniform across $t$ or $i$. In the following, Lemma \ref{lem: eigenvector bound} establishes a sup-norm bound on the estimated singular vectors, and then uniform convergence of the estimated factors and loadings is given in Theorem \ref{thm: uniform convergence of factors}.

\begin{lem}\label{lem: eigenvector bound}
	Under Assumption \ref{SA Assumption: Matching} and \ref{SA Assumption: LPCA}, if $\delta_{KT}h_{K,\xi}^{m-1}\rightarrow\infty$, $\frac{n^{\frac{4}{\nu}}(\log n)^{\frac{\nu-2}{\nu}}}{T}\lesssim 1$,  and $(nT)^{\frac{2}{\nu}}\delta_{KT}^{-2}\lesssim 1$,
	\iffalse
	%%%% This is a more precise requirement
	$\frac{(nT)^{\frac{1}{1+\nu}}\log^{\frac{\nu}{1+\nu}} (n\vee T)}{K}\lesssim 1$ and
	$\frac{(nT)^{\frac{1}{1+\nu}}\log^{\frac{\nu}{1+\nu}} (n\vee T)}{K}\lesssim 1$,
	\fi 
	then 
	\[
	\max_{1\leq i\leq n}
	\|\widehat{\bF}_{\subi}\|_{\max}\lesssim_\P 1, \quad
	\max_{1\leq i\leq n}\|\widehat{\bLambda}_{\gr{\ell},\subi}\|_{\max}\lesssim_\P h_{K,\xi}^{\ell}, \quad \text{for }\; \ell=1, \cdots, m-1.
	\]
\end{lem}

\begin{thm} 
	\label{thm: uniform convergence of factors}
	Under Assumptions \ref{SA Assumption: Matching} and \ref{SA Assumption: LPCA}, if $\delta_{KT}h_{K,\xi}^{m-1}\rightarrow\infty$, $\frac{n^{\frac{4}{\nu}}(\log n)^{\frac{\nu-2}{\nu}}}{T}\lesssim 1$,  and $(nT)^{\frac{2}{\nu}}\delta_{KT}^{-2}\lesssim 1$, then for $j=1, \ldots, \mathsf{d}_\lambda$, 
	there exists $\bH_{\subi}$ such that 
	\[
	\begin{split}
	&\max_{1\leq i\leq n}\|\widehat{\bF}_{\cdot j,\subi}-\bF_{\subi}((\bH_{\subi}')^{-1})_{\cdot j}\|_{\max}\lesssim_\P
	\delta_{KT}^{-1}\Upsilon_{jj}^{-1}
	+h_{K,\xi}^{m}\Upsilon_{jj}^{-1},\\
	&\max_{1\leq i\leq n}\|\widehat{\bLambda}_{\cdot j,\subi}-\bLambda_{\subi}\bH_{\cdot j,\subi}\|_{\max}\lesssim_\P
	\delta_{KT}^{-1}+h_{K,\xi}^{m}.
	\end{split}
	\]
	Moreover, $1\lesssim_\P \min_{1\leq i\leq n}s_{\min}(\bH_{\subi})\leq \max_{1\leq i\leq n}s_{\max}(\bH_{\subi})\lesssim_\P 1$.
\end{thm}

Finally, the following theorem shows that the estimated mean structure is consistent.
\begin{thm}\label{thm: consistency of latent mean}
	Under the conditions of Theorem \ref{thm: uniform convergence of factors}, $$\max_{1\leq i\leq n,1\leq j\leq K,t\in\mathcal{T}_2}
	|\widehat{L}_{tj,\subi}-L_{tj,\subi}|\lesssim_\P \delta_{KT}^{-1}+h_{K,\xi}^m.$$
\end{thm}

\subsection{Discussion of Three Geometric Conditions}
At the beginning of this section, I introduce three definitions concerning the geometry of the underlying manifold generated by latent functions. This section discusses these properties with examples and deduce some lower-level conditions for verification.

I first want to remind readers that Definitions \ref{SA-Definition: nonsingularity}-\ref{SA-Definition: non-collapsing} are stated in a probabilistic sense, the probability sign $\P(\cdot)$ involves the randomness across both dimensions, and the i.i.d. sequence $\{\bxi_i\}$ plays the role of random evaluation points. However, if the maxima or minima over the evaluation points in these conditions are replaced by suprema or infima over the whole support, then they no longer rely on the ``cross-sectional'' (indexed by $i$) randomness and concern the features of latent functions only. 

In addition, the randomness of the latent functions $\{\mu_{t,A}(\cdot)\}_{t=1}^T$ can be understood in several ways. For example, they could be a sample of functional random variables (f.r.v) satisfying certain smoothness conditions. See \cite{Ferraty-Vieu_2006_book} for general discussion of functional data analysis. Alternatively, it may be generated based on a more restrictive but practically interesting specification:
$\mu_{t,A}(\bxi_i):=\mu_A(\bm{\varpi}_t;\bxi_i)$,
where $\mu_A(\cdot;\cdot)$ is a fixed function and the randomness across the $t$ dimension is induced by a sequence of random variables $\{\bm{\varpi}_t\}_{t=1}^T$ with some distribution $F_{\varpi}(\cdot)$ on $\mathcal{Z}$.
For simplicity, attention will be restricted to this specific case in the following discussion. 

\subsubsection*{Definition \ref{SA-Definition: nonsingularity}}
The nonsingularity condition \eqref{eq: def of nonsingularity} can be viewed as the continuity of the inverse map of $\bmu_{A}(\cdot)$. To see this, let us understand $\mu_A(\bm{\varpi}_t;\bxi_i)$ as a function indexed by $\bxi_i\in\mathcal{E}$ where $\mathcal{E}$ denotes the support of $\bxi_i$. For $\mathfrak{d}(\cdot,\cdot)=\mathfrak{d}_2(\cdot,\cdot)$, under mild regularity conditions in the  literature, we may establish the following uniform convergence result:
\[
\sup_{\bxi,\bxi'\in\mathcal{E}}\Big|\frac{1}{T}\sum_{t=1}^{T}\Big(\mu_A(\bm{\varpi}_t;\bxi)-\mu_A(\bm{\varpi}_t;\bxi')\Big)^2-\E\Big[\Big(\mu_A(\bm{\varpi}_t;\bxi)-\mu_A(\bm{\varpi}_t;\bxi')\Big)^2\Big]\Big|=o_\P(1),
\]
where the expectation is taken against the distribution of $\bm{\varpi}_t$.
Then, we can safely remove the randomness arising from $\bm{\varpi}_t$ and impose conditions on the limit only. Specifically, the condition in Definition \ref{SA-Definition: nonsingularity} reduces to: for any $\epsilon>0$, there exists $\Delta$ such that for all $\bxi,\bxi'\in\mathcal{E}$, 
\[
\int \Big(\mu_A(\bm{\varpi};\bxi)-\mu_A(\bm{\varpi};\bxi')\Big)^2dF_{\varpi}(\bm{\varpi})< \Delta
\Rightarrow\|\bxi-\bxi'\|_2< \epsilon,
\]
where ``$\Rightarrow$'' means ``implies''.
Conceptually, if we define $g: \bxi\mapsto\mu_A(\cdot;\bxi)$ which is a map from $\mathcal{E}$ to $L^2(\mathcal{Z})$ (a set of square-integrable functions on $\mathcal{Z}$ equipped with $L_2$-norm), then the above condition essentially says that the inverse map $g^{-1}$ exists and uniformly continuous.

\begin{exmp}[Polynomial]
Let $\mu_A(\varpi;\xi)=1+\varpi\xi+\varpi^2\xi^2$,  $\mathcal{Z}=\mathcal{E}=[0,1]$, and $F_\varpi$ be a uniform distribution. Then, for $\xi,\xi'\in\mathcal{E}$,
$\int_{[0,1]}(\mu_A(\varpi;\xi)-\mu_A(\varpi;\xi'))^2dF_{\varpi}(\varpi)=(\xi-\xi',\xi^2-(\xi')^2)
(\int_{[0,1]}(\varpi,\varpi^2)'(\varpi,\varpi^2)d\varpi)
(\xi-\xi',\xi^2-(\xi')^2)'$.
The matrix in the middle is simply one block in the Hilbert matrix with the minimum eigenvalue bounded away from zero. Then, the desired result immediately follows.
\hfill\qedsymbol
\end{exmp}

\begin{exmp}[Trigonometric function]
	Let $\mu_A(\varpi;\xi)=\sin(\pi(\varpi+\xi))$, $\mathcal{Z}=\mathcal{E}=[0,1]$, and $F_\varpi$ be a uniform distribution. Take any two points $\xi,\xi'\in\mathcal{E}$ such that $\xi\neq\xi'$. Without loss of generality, assume $\xi>\xi'=0$ and $\epsilon=\xi-\xi'$. Consider the following cases: when $0\leq\epsilon<\xi<1/2$,  $|\mu_A(\varpi;\xi)-\mu_A(\varpi;\xi')|\geq\frac{1}{\sqrt{2}}(1-\cos\epsilon)$ for all $\varpi\in(0,1/2)$; and when $1/2\leq \epsilon<\xi\leq 1$, $|\mu_A(\varpi;\xi)-\mu_A(\varpi;\xi')|\geq \sin\varpi$ for all $\varpi\in[0,1/2]$. This suffices to show that for each $\epsilon>0$, there exists $\Delta_\epsilon>0$ such that for all $|\xi-\xi'|>\epsilon$,  $\int(\mu_A(\varpi;\xi)-\mu_A(\varpi;\xi'))^2d\varpi>\Delta_\epsilon$, which is simply the contrapositive of the desired result.
\hfill\qedsymbol
\end{exmp}

The two dimensions indexed by $i$ and $t$ are treated symmetrically in the above examples. However, the smoothness in the $t$ dimension is unnecessary in my framework. For example, consider a simple artificial specification:
$\mu_{t,A}(\xi)=\xi^2+1$ for $t=1$ and $\mu_{t,A}(\xi)=2\xi^2+1$ for $t>1$.
Clearly, the first period is distinct from all other periods. However, for any $\xi,\tilde{\xi}\in\mathcal{E}=[0,1]$ such that $|\xi-\tilde{\xi}|>\epsilon$,
$\frac{1}{T}\sum_{t=1}^{T}(\mu_{t,A}(\xi)-\mu_{t,A}(\tilde{\xi}))^2
	\geq 4(\xi^2-\tilde{\xi}'^2)^2 \geq 4\epsilon^4$.
Multiple regime shifts and more complex factor structures are allowed as long as there are sufficiently many ``dimensions'' in which the difference in values of $\xi$ can be detected. 

Until now, I have only discussed the condition corresponding to the Euclidean distance. However, the above condition will be sufficient when $\mathfrak{d}_\infty(\cdot,\cdot)$ is used as well. To see this, first remove the randomness by uniform law of large numbers:
$\sup_{\bxi,\bxi',\bxi''\in\mathcal{E}}|\frac{1}{T}\sum_{t=1}^{T}(\mu_A(\bm{\varpi}_t;\bxi)-\mu_A(\bm{\varpi}_t;\bxi'))\mu_A(\bm{\varpi};\bxi'')-\E[(\mu_A(\bm{\varpi}_t;\bxi)-\mu_A(\bm{\varpi}_t;\bxi'))\mu_A(\bm{\varpi}_t;\bxi'')]|=o_\P(1)$. Next, note that
$\max_{\bxi''\in\mathcal{E}}|\E[(\mu_A(\bm{\varpi}_t;\bxi)-\mu_A(\bm{\varpi}_t;\bxi'))\mu_A(\bm{\varpi}_t;\bxi'')]|=o(1)$ implies
$\E[(\mu_A(\bm{\varpi}_t;\bxi)-\mu_A(\bm{\varpi}_t;\bxi'))^2]=o(1)$. 
Combining this with the previous condition for Euclidean metric $\mathfrak{d}_2(\cdot,\cdot)$, we can establish the asymptotic nonsingularity with respect to $\mathfrak{d}_\infty(\cdot,\cdot)$.

\subsubsection*{Definition \ref{SA-Definition: non-degenerate}}
Definition \ref{SA-Definition: non-degenerate} simply requires that the nonlinearity of $\bmu_A(\cdot)$ exist. Again, under mild conditions, we can make the sample average across $t$ converge and restate the condition in terms of the limit. For $\kappa=1$, it becomes
\[
\int \Big(\mu_A(\bm{\varpi}_t;\bxi),\,\frac{\partial}{\partial\bxi}\mu_A(\bm{\varpi}_t;\bxi)\Big)\Big(\mu_A(\bm{\varpi}_t;\bxi),\,\frac{\partial}{\partial\bxi}\mu_A(\bm{\varpi}_t;\bxi)\Big)'dF_\varpi(\bm{\varpi})\geq\underline{c}>0
\] 
uniformly over $\bxi$.

\begin{exmp}[Polynomial, continued]
The first-order derivative is $\frac{d}{d\xi}\mu_A(\varpi;\xi)=\varpi+2\varpi^2\xi$. Let $\bg(\varpi;\xi)=(1+\varpi\xi+\varpi^2\xi^2,\, \varpi+2\varpi^2\xi)'$. Then,
\begin{align*}
\int_{[0,1]}\bg(\varpi;\xi)\bg(\varpi;\xi)'d\varpi&=
\tilde{\bg}(\xi)\Big(\int_{[0,1]}(1,\varpi,\varpi^2)'(1,\varpi,\varpi^2)d\varpi\Big)
\tilde{\bg}(\xi)'\\
&\gtrsim\tilde{\bg}(\xi)\tilde{\bg}'(\xi),\qquad\text{for}\quad
\tilde{\bg}(\xi)=\bigg(\begin{array}{ccc}
1&\xi&\xi^2\\
0&1&2\xi
\end{array}
\bigg).
\end{align*}
$\tilde{\bg}(\xi)\tilde{\bg}(\xi)'$ is positive definite for any $\xi$. The coefficients of its characteristic functions are continuous on a compact support, and thus by Theorem 3.9.1 of \cite{Tyrtyshnikov_2012_book}, their eigenvalues are also continuous on the support. Then, the desired result follows.
\hfill\qedsymbol
\end{exmp}

\begin{exmp}[Trigonometric function, continued]
	Note $\frac{d}{d\xi}\mu_A(\varpi;\xi)=\pi\cos(\pi(\varpi+\xi))$. Let $\bg(\varpi;\xi)=(\sin(\pi(\varpi+\xi)), \pi\cos(\pi(\varpi+\xi)))'$. Then,
	\[
	\begin{split}
	&\int_{[0,1]}\bg(\varpi;\xi)\bg(\varpi;\xi)'d\varpi=
	\tilde{\bc}\Big(\int_{[0,1]}\tilde{\bg}(\varpi;\xi)\tilde{\bg}(\varpi;\xi)'d\varpi\Big)\tilde{\bc}
	=\frac{1}{2\pi}\tilde{\bc}\bigg(\begin{array}{cc}
	\pi&0\\
	0&\pi
	\end{array}\bigg)\tilde{\bc},	
	\quad\text{where}\\
	&\tilde{\bg}(\varpi;\xi)=(\sin(\pi(\varpi+\xi)), \cos(\pi(\varpi+\xi)))', \quad\tilde{\bc}=\bigg(\begin{array}{cc}
	1&0\\
	0&\pi
	\end{array}
	\bigg).
	\end{split}
	\]
	Then, the desired result follows.
	\hfill\qedsymbol
\end{exmp}

\subsubsection*{Definition \ref{SA-Definition: non-collapsing}}
Finally, consider Definition \ref{SA-Definition: non-collapsing}. When the conditions of Definition \ref{SA-Definition: non-degenerate} hold up to order $\kappa\geq 1$, the tangent space is well defined at every point. Letting all the sample averages converge to the limits, we can replace the sample-based projection operator $\mathscr{P}_{\bxi}$ by the population-based one. The condition can be restated as
\[
\inf_{\bxi\in\mathcal{E}}\sup_{\tilde{\bxi}\in\mathcal{E}}\Big\|
\int\Big(\frac{\partial}{\partial \bxi}\mu_A(\bm{\varpi};\bxi)\Big)\mu_A(\bm{\varpi};\tilde{\bxi})dF_\varpi(\bm{\varpi})\Big\|_2\geq \underline{c}'>0.
\]

\begin{exmp}[Polynomial, continued]
	In this scenario,
	\[
	\sup_{\tilde{\xi}}\Big|\int_{[0,1]}\Big(\frac{d}{d\xi}\mu_A(\varpi;\xi)\Big)\mu_A(\varpi;\tilde{\xi})d\varpi\Big|=
	\sup_{\tilde{\xi}}\Big|\frac{1}{2}+\frac{\tilde{\xi}}{3}+\frac{\tilde{\xi}^2}{4}+\Big(\frac{2}{3}+\frac{\tilde{\xi}}{2}+\frac{2\tilde{\xi}^2}{5}\Big)\xi\Big|\geq \frac{13}{12}
	\]
	by taking $\tilde{\xi}=1$. Then, the result follows.
	\hfill\qedsymbol
\end{exmp}

\begin{exmp}[Trigonometric function, continued]
	In this scenario,
	\[
	\begin{split}
	\sup_{\tilde{\xi}}\Big|\int_{[0,1]}\Big(\frac{d}{d\xi}\mu_A(\varpi;\xi)\Big)\mu_A(\varpi;\tilde{\xi})d\varpi\Big|&=
	\sup_{\tilde{\xi}}\Big|\int_{[0,1]}\pi\cos(\pi(\varpi+\xi))\sin(\pi(\varpi+\tilde\xi))d\varpi\Big|\\
	&=\pi\sup_{\tilde{\xi}}\Big|\frac{\sin(\pi(\xi-\tilde{\xi}))}{2}\Big|
	\geq \pi/2,
	\end{split}
	\]
	by simply taking $|\tilde{\xi}-\xi|=0.5$.
    Then, the result follows.
    \hfill\qedsymbol
\end{exmp}

%%%%%%%%%%%%%%%%%%%%%%%%%%%%%%%%%%%%%%%%%%%%%%%%%%%%%%%%%%%%%%%
%%%%%%%%%%%%%%%%%%%%%%%%%%%%%%%%%%%%%%%%%%%%%%%%%%%%%%%%%%%%%%%
\section{Treatment Effects Model} \label{SA-sec: setup}

This section sets up a theoretical framework which generalizes the basic one considered in the main paper in two aspects: a set of variables $\bw_i$ enter the nonlinear factor model for $\bx_i$ as additional high-rank regressors, and the potential outcomes and treatment assignment are characterized by  generalized partially linear models. 
 
Suppose that a researcher observes a random sample $\{(y_{i}, s_{i}, \bx_{i}, \bw_i, \bz_{i})\}_{i=1}^n$, where $y_{i}\in\mathcal{Y}\subseteq\mathbb{R}$ is an observed outcome, $s_i\in\mathcal{J}=\{0,\cdots, J\}$ denotes the  treatment status, and $\bx_{i}\in\mathbb{R}^{T}$, $\bw_i\in\mathbb{R}^{T\ttd_w}$ and $\bz_i\in\mathbb{R}^{\ttd_z}$ are vectors of covariates. $\bx_i$, $\bw_i$ and $\bz_i$ play different roles: $\bx_i$ and $\bw_i$ are used to extract information on latent confounders, while $\bz_i$ is a set of control variables that need to be controlled for in counterfactual analysis. The asymptotic theory in this paper is developed assuming $n$ and $T$ simultaneously go to infinity whereas $\ttd_w$ and $\ttd_z$ are fixed. 
 
Let $y_i(\jmath)$ denote the potential outcome of unit $i$ at treatment level $\jmath$, and construct an indicator variable $d_{i}(\jmath)=\I(s_{i}=\jmath)$. The observed outcome then can be written as $y_{i}=\sum_{\jmath=0}^{J}d_{i}(\jmath)y_{i}(\jmath)$. 
For each treatment level $\jmath\in\mathcal{J}$, the potential outcome is modeled by 
\begin{equation}
y_{i}(\jmath)=\varsigma_{i,\jmath}+\epsilon_{i,\jmath}, \qquad \psi_{\tty}^{-1}(\varsigma_{i,\jmath})=\bz_i'\bbeta_\jmath+\mu_\jmath(\balpha_i), \qquad \E[\epsilon_{i,\jmath}|\bz_i,\balpha_i]=0,\label{SA-eq: outcome}
\end{equation}
where $\balpha_i\in\mathbb{R}^{\ttd_\alpha}$ is a set of \textit{unobserved} variables with $\ttd_{\alpha}$ fixed, and 
$\psi_{\tty}^{-1}(\cdot):\mathbb{R}\mapsto\mathbb{R}$ is a (strictly monotonic) link function. On the other hand, the treatment assignment is characterized by
\begin{equation}
\bm{d}_{i}=\bm{p}_{i}+\bv_{i},\qquad
\bpsi^{-1}_{\tts}(\bm{p}_{i})=\bgamma\bz_{i}+\bm{\rho}(\balpha_i),\qquad 
\E[\bv_{i}|\bz_i,\balpha_i]=0, \label{SA-eq: treatment}
\end{equation}
where $\bm{d}_i=(d_i(0),\cdots, d_i(J))'$, $\bm{p}_i=(p_{i,0},\cdots, p_{i,J})'$ such that $\sum_{\jmath=0}^{J}p_{i,\jmath}=1$, $\bgamma=(\bgamma_1,\cdots,\bgamma_J)'$,
$\bm{\rho}(\cdot)=(\rho_1(\cdot),\cdots,\rho_J(\cdot))'$, $\bv_i=(v_{i,0},\cdots, v_{i,J})$, 
and $\bpsi^{-1}_{\tts}(\cdot):(0,1)^{J+1}\mapsto\mathbb{R}^{J}$ is a link function associated with the multi-valued treatment. Note that $\jmath=0$ is set as the base level.

$\varsigma_{i,\jmath}$ in Equation \eqref{SA-eq: outcome} is the conditional mean of the potential outcome at level $\jmath$ given the observed covariates and unobserved latent variables.
Similarly, each $p_{i,\jmath}$ in Equation \eqref{SA-eq: treatment} denotes the conditional probability of treatment level $\jmath$. 

Equations \eqref{SA-eq: outcome} and \eqref{SA-eq: treatment} essentially assume that $\varsigma_{i,\jmath}$ and $p_{i,\jmath}$ take generalized partially linear forms. The observed covariates $\bz_{i}$ enter the model parametrically, the unobserved variables $\balpha_i$ enter the model nonparametrically through some unknown functions $\mu_\jmath(\cdot)$ and $\rho_\jmath(\cdot)$, and two parts are additively separable (within the link function). Since the latent variables $\balpha_i$ are unobservable, the standard estimation methods in the semiparametrics literature cannot be applied directly.

\subsection{Structure of Large-Dimensional Measurements}
I assume $\bx_i$ takes a particular covariates-adjusted nonlinear factor structure.
Specifically, partition $\bw_i\in\mathbb{R}^{T\ttd_w}$ into
\[
\bw_i=(\bw'_{i,1},\cdots, \bw'_{i,\ttd_w})', 
\]
where
$\bw_{i,\ell}=(w_{i1, \ell}, \cdots, w_{iT,\ell})'$,
$\ell=1, \cdots, \ttd_w$. The covariates 
$\bx_{i}=(x_{i1}, \cdots, x_{iT})'$ are the main source of learning $\balpha_i$. It is modeled as a mixture of high-rank components formed by $\{\bw_{i,\ell}\}_{\ell=1}^{\ttd_w}$ and a nonlinear factor component about $\balpha_i$:
\begin{equation}\label{SA-eq: HD covariate}
x_{it}=\sum_{\ell=1}^{\ttd_w}
\vartheta_\ell w_{it,\ell}+\eta_{t}(\balpha_i)+u_{it}, \quad \E[u_{it}|\mathcal{F}_0,\{\bw_i\}_{i=1}^n]=0,
\end{equation}
where $\mathcal{F}_0$ is the $\sigma$-field generated by  $\{\balpha_i\}_{i=1}^n$ and $\{\eta_t(\cdot)\}_{t=1}^T$. 
Let 
$\bmeta_i=(\eta_1(\balpha_i),\cdots, \eta_T(\balpha_i))'$, 
%$\bL_{i}=(L_{i1}, \cdots, L_{iT})'$, 
$\bu_{i}=(u_{i1},\cdots,u_{iT})'$, $\bW_{i}=(\bw_{i,1},\cdots \bw_{i,\ttd_w})$, and $\bvth=(\vartheta_1,\cdots, \vartheta_\ell)'$. 
Equation \eqref{SA-eq: HD covariate} can then be written in matrix form:
\[
\bx_i=\bW_{i}\bvth+\bmeta_i+\bu_{i}, \quad i=1, \cdots, n.
\]

%%%%%%%%%%%%%%%%%%%%%%%%%%%%%%%%%%%%%%%%%%%%%%%%%%%%%%%%%%%%%%%%%%%%%%
\section{Typical Applications} \label{SA-sec: example}
In addition to the empirical example of synthetic control analysis illustrated in Section 3 in the main paper, the methods developed in this paper are applicable to many other problems. In this section, I discuss some typical applications and explain how the analysis can be conducted within the general framework given in Section \ref{SA-sec: setup}. %The first application, synthetic control design, will be illustrated using a real dataset in Section \ref{sec: estimation} below.

\subsection{Staggered Adoption}
As in the synthetic control design, the researcher observes the outcome $Q$ of $n$ units in $T+T'$ periods, and the treatment starts at time $T+1$. However, different units may adopt the treatment in different periods. This setting is referred to as staggered adoption design in \cite{Athey-Imbens_2018_wp} and can be analyzed in a multi-valued treatment framework. Specifically, let $S$ be the random treatment date taking values in $\mathcal{J}=\{T+1, \cdots, T+T',\infty\}$. The treatment $s_i$ is the observed adoption time, which may be censored from the right: a unit $i$ remains always untreated if $s_i>T+T'$, denoted by $s_i=\infty$. For $t>T$, we can use $q_{it}(\jmath)$ to denote the potential outcome of unit $i$ at time $t$ if it adopted the treatment in some period $\jmath\in\mathcal{J}$. As in the synthetic control design, the outcomes prior to the treatment can be used as the large-dimensional covariates $\bx_i$.
With this more flexible treatment pattern, the researcher may define many interesting parameters. For example, let the potential outcomes of interest be $y_i(\jmath)=q_{it}(\jmath)$ and $y_i(\infty)=q_{it}(\infty)$. Then,  $\theta=\E[y_{i}(\jmath)-y_{i}(\infty)|s_i=\jmath]$ is the average treatment effect relative to the never-treated status on those adopting the treatment in period $\jmath\in\mathcal{J}$, which is measured in period $t\geq \jmath$.

\subsection{Recommender System}
Observational recommendation data usually contain information on which item each user likes. Formally, let $i$ index users and $t$ index items. A sequence of binary variables $\{q_{it}:1\leq i\leq n,1 \leq t\leq T\}$ records whether or not each user $i$ likes (``clicks on'') the $T$ items. A binary treatment of particular interest in practice is the exposure to a ``new'' item $T+1$: $s_{i}$ equals 1 if user $i$ has an \textit{opportunity} to click on item $T+1$. The goal is to infer users' preference and predict whether users not exposed to item $T+1$ will like it. The potential outcome $y_i(1)$ in this scenario is the indicator of whether or not user $i$ likes item $T+1$ given her exposure to it. A parameter of interest may be $\theta=\E[y_i(1)|s_i=0]$,
the probability of ``clicking on'' item $T+1$ if the group of unexposed users had been exposed to it. The large-dimensional covariates $\bx_i=(q_{i1},\cdots,q_{iT})'$ is simply the users' ``clicking'' history. See  \cite{Liang-et-al_2016_wp} for an example of causal recommendation model. For more discussion of recommendation problems based on matrix estimation method, see \citet[Chapter 10]{Wainwright_book_2019}.

\subsection{Causal Inference with Measurement Error}
In previous examples, $\bx_i$ is a collection of past outcomes, but it need not be. The framework in this paper naturally covers the case in which many highly correlated proxies $\bx_i\in\mathbb{R}^T$ characterize some unmeasured traits $\balpha_i\in\mathbb{R}^{\ttd_\alpha}$ of subjects. Therefore, the method developed in this paper is similar to the pre-processing technique popular in the recent machine learning literature. For example, \cite{Kallus-Mao-Udell_2018_inbook} develops a causal inference method based on matrix factorization to handle noisy covariates. Also, other methods for nonlinear models with measurement errors exist in the literature. See \cite{Schennach_2016_ARE} for a review.

\subsection{Diffusion Index Forecasts}
The idea of this paper is connected with diffusion index forecasts in macroeconomics \citep{Stock-Watson_2002_JASA,Stock-Watson_2002_JBES}, where the goal is to predict a scalar time series $y_{t+1}$ characterized by a linear model of factors (diffusion indexes) $\bff_t$ and lags of $y_t$. An $n$-dimensional multiple time series $\bx_t=(x_{1t}, \cdots, x_{nt})'$ of predictors is available for $t=1, \cdots, T$. $x_{it}$ is assumed to take a linear factor structure: $x_{it}=\blambda_i'\bff_t+u_{it}$. Such models are usually estimated in two steps: estimate the diffusion index $\bff_t$ based on $\{\bx_t\}_{t=1}^T$, and then run a linear regression of $y_{t+1}$ on the estimated $\bff_t$ and $y_t$ (lags). $\bff_t$ in this scenario plays a similar role as $\balpha_i$ in my framework. The main difference is that $x_{it}$ in this paper is allowed to take a possibly nonlinear factor structure.

\subsection{Network Analysis}
The key idea used to extract information on latent variables in this paper is related to the graphon estimation method in network literature \citep{Gao-Lu-Zhou_2015_AoS,Zhang-Levina-Zhu_2017_BIMA}. In that context, an adjacency matrix $\bA\in\mathbb{R}^{n\times n}$ is generated from a probability matrix $\bP\in\mathbb{R}^{n\times n}$. The probability $P_{ij}$ for a generic pair $(i,j)$ is assumed to be $P_{ij}=\eta(\alpha_i,\alpha_j)$ for $\alpha_i\sim \mathsf{U}[0,1]$, where $\eta(\cdot,\cdot)$ is referred to as the graphon function. The framework in this paper may be adapted for this model. In particular, my proposed method can be used to estimate $P_{ij}$ and conduct causal inference for social networks exploiting the latent information contained in adjacency matrices. For a review of econometric methods for network data, see \cite{Graham_2020_inbook}.

%%%%%%%%%%%%%%%%%%%%%%%%%%%%%%%%%%%%%%%%%%%%%%%%%%%%%%%%%%%%%%%%%%%
\section{Estimation Procedure} \label{SA-sec: estimation}

This section presents the main estimation procedure that accommodates the more general model described above.

\subsection{Local Principal Subspace Approximation}
To begin with, I summarize the general local principal subspace approximation (LPSA) procedure formally treated in Section \ref{SA-sec: general LPSA}. Later it will be applied to extract latent variables based on Equation \eqref{SA-eq: HD covariate}. 

Suppose that the data $\{\ba_i\in\mathbb{R}^T:1\leq i\leq n\}$ admit a pure nonlinear factor structure as in Equation \eqref{SA-eq: pure nonlinear factor}. In later applications, $\{\ba_i\}$ will be $\{\bx_i\}$, $\{\bw_{i,1}\},\cdots, $ or $\{\bw_{i,\ttd_w}\}$. For the moment, $\{\ba_i\}_{i=1}^n$ denotes a generic sequence of variables. Let $\bA_{T\times n}=(\ba_1,\cdots, \ba_n)$.

\textbf{\textit{Row-wise Splitting.}} Split the row index set $\mathcal{T}=\{1,\cdots, T\}$ of $\bA$ into two parts randomly: $\mathcal{T}=\mathcal{T}^\dagger\cup\mathcal{T}^\ddagger$. Accordingly, the data matrix $\bA$ is divided into two submatrices $\bA^{\dagger}=\bA_{\mathcal{T}^\dagger\cdot}$ and $\bA^{\ddagger}=\bA_{\mathcal{T}^\ddagger\cdot}$. This step is needed only when local PCA is implemented.

\textbf{\textit{$K$-Nearest Neighbors Matching.}} For a generic unit $1\leq i\leq n$, define a set of indices $\mathcal{N}_i(\bA^{\dagger})=\{j_1(i), \cdots, j_K(i)\}$ for $K$ nearest neighbors (including unit $i$ itself) in terms of  $\mathfrak{d}(\bA^{\dagger}_{\cdot i}, \bA^{\dagger}_{\cdot j})$ for every $j$, where $\mathfrak{d}(\cdot, \cdot)$ is either the Euclidean distance $\mathfrak{d}_2(\cdot,\cdot)$ or the pseudo-max distance $\mathfrak{d}_\infty(\cdot,\cdot)$.

Given an outcome variable of interest, if local constant approximation is desirable, then for each unit $i$, simply take the local average of outcomes for units within the neighborhood $\mathcal{N}_i(\bA^\dagger)$. A sequence of neighborhoods $\{\mathcal{N}_i(\bA^\dagger)\}_{i=1}^n$ is the only quantity carried to the treatment effects analysis. Local PCA in the next step can be skipped and row-wise sample splitting is unnecessary.

\textbf{\textit{Local Principal Component Analysis.}} 
Given each neighborhood $\mathcal{N}_i(\bA^{\dagger})$ from the previous step, define a $T\times K$ matrix $\bA_{\subi}=(\bA^{\ddagger}_{\cdot j_1(i)}, \cdots, \bA^{\ddagger}_{\cdot j_K(i)})$ based on the subsample $\bA^{\ddagger}$. %Intuitively, by localizing the data, we can approximate the unknown function $\eta_t(\cdot)$ by a linear combination of basis functions of $\balpha_i$ using, for example, Taylor's expansion. By this observation, if we ignore approximation errors, the data matrix $\bA^{\ddagger}_{\subi}$ admits a low-rank factor structure.  
Implement the following local principal component analysis on $\bA_{\subi}$:
\[
(\widehat{\bF}_{\subi}, \widehat{\bLambda}_{\subi})=
\underset{\bF_{\subi}\in\mathbb{R}^{|\mathcal{T}_2|\times \ttd_\lambda}, \bLambda_{\subi}\in\mathbb{R}^{K\times \ttd_\lambda}}{\argmin}\tr\Big[\Big(\bA_{\subi}-\bF_{\subi}\bLambda_{\subi}'\Big)\Big(\bA_{\subi}-\bF_{\subi}\bLambda_{\subi}')'\Big],
\]
such that $\frac{1}{|\mathcal{T}_2|}\bF_{\subi}'\bF_{\subi}=\bI_{\ttd_{\lambda}}$ and $\frac{1}{K}\bLambda_{\subi}'\bLambda_{\subi}$ is diagonal. $\ttd_\lambda$ is a user-specified number of approximation terms.
$\{\mathcal{N}_i(\bA^\dagger)\}_{i=1}^n$ and  $\{\widehat{\bLambda}_{\subi}\}_{i=1}^n$ are desired quantities containing information on latent variables.
Let $\widehat{\blambda}_{i,\subi}$ be the column in $\widehat{\bLambda}_{\subi}$ that corresponds to unit $i$. Then,
the predicted value for $\bA^{\ddagger}_{\cdot i}$ is  $\widehat{\bA}^{\ddagger}_{\cdot i}=\widehat{\bF}_{\subi}\widehat{\blambda}_{i,\subi}$. 

\subsection{Main Procedure}
\subsubsection{Step 1: Latent Variables Extraction} \label{SA-subsec: latent variable extraction}
The main steps to extract latent variables based on Equation \eqref{SA-eq: HD covariate} are as follows:

\begin{enumerate}[label=(\alph*)]
	\item Split the row index set $\mathcal{T}=\{1, \cdots, T\}$ into three (non-overlapping) portions: $\mathcal{T}=\mathcal{T}_1\cup\mathcal{T}_2\cup\mathcal{T}_3$. $|\mathcal{T}_1|$, $|\mathcal{T}_2|$, and $|\mathcal{T}_3|$ are all proportional to $T$.
	
	\item On $\mathcal{T}_1\cup\mathcal{T}_2$, for each $\ell=1, \ldots, \ttd_w$, apply LPSA to each high-rank covariate, i.e., let $\{\ba_i\}_{i=1}^n=\{\bw_{i,\ell}\}_{i=1}^n$. Obtain residuals  $\widehat{\be}_{i,\ell}:=\bw_{i,\ell}-\widehat{\bw}_{i,\ell}$. $\mathcal{T}_1$ is used for matching and $\mathcal{T}_2$ for local PCA.
	
	\item On $\mathcal{T}_1\cup\mathcal{T}_2$, apply LPSA to $\{\ba_i\}_{i=1}^n=\{\bx_{i}\}_{i=1}^n$. The obtained residuals are $\widehat{\bu}^{\natural}_{i}=\bx_{i}-\widehat{\bx}_{i}$.
	
	\item Let $\widehat{\be}_{i}=(\widehat{\be}_{i,1},\cdots, \widehat{\be}_{i,\ttd_w})'$. Estimate $\bvth$ by
	\[
	\widehat{\bvth}=\Big(\frac{1}{n}\sum_{i=1}^{n}\widehat{\be}_{i}\widehat{\be}_{i}'\Big)^{-1}\Big(\frac{1}{n}\sum_{i=1}^{n}\widehat{\be}_{i}\widehat{\bu}^{\natural}_{i}\Big).
	\]
	
	\item On $\mathcal{T}_2\cup\mathcal{T}_3$, apply LPSA to the covariates-adjusted $\bx_{i}$, i.e., $\{\ba_i\}_{i=1}^n=\{\bx_{i}-\bW_{i}\widehat{\bvth}\}_{i=1}^n$. The index sets for nearest neighbors and factor loadings obtained in this step are denoted by $\{\mathcal{N}_i\}_{i=1}^n$ and $\{\widehat{\bLambda}_{\subi}\}_{i=1}^n$ respectively, which are only quantities carried to next steps.  
\end{enumerate}
\begin{remark}
Here are some remarks on the role of sample splitting in the above procedure. Since the matching step has implicitly used the information on noise, without sample splitting across $1\leq t\leq T$, the factor component would have been correlated with noise within a local neighborhood. Therefore, each time the local PCA is implemented, I split the sample to separate matching and principal component analysis. Note that the above procedure simply mimics the idea of semiparametric partially linear estimation. Steps (b) and (c) play the role of removing the factor component from both $\bx_{i}$ and $\bw_{i}$, and step (d) estimates the low-dimensional slope coefficient $\bvth$. Step (e) extracts the factor component of interest from the residuals obtained in step (d). Matching in this step is implemented on $\mathcal{T}_2$, and the third portion $\mathcal{T}_3$ is used for further local approximation and extracting factor loadings $\widehat{\bLambda}_{\subi}$. 

Three-fold splitting is \textit{not} always necessary. For example, if there is no need to control for the high-rank covariates $\bw_{i}$, two-fold splitting suffices as in the main paper. Also, if one is satisfied with ``local constant'' approximation, then sample splitting is unnecessary.
\end{remark}

\subsubsection{Step 2: Factor-Augmented Regression} \label{subsubsection: step 2}
For the outcome equation \eqref{SA-eq: outcome}, consider a quasi-log-likelihood function $\mathcal{L}_{\tty}(\varsigma, y)$ such that
$\frac{\partial}{\partial \varsigma}
\mathcal{L}_{\tty}(\varsigma,y)=\frac{y-\varsigma}{V_{\tty}(\varsigma)}$.
Then, a local quasi-maximum likelihood estimator of $\varsigma_{i,\jmath}$ is given by
\[
\begin{split}
\widehat{\varsigma}_{i,\jmath}=\psi_{\tty}\Big(\bz_{i}'\widehat{\bbeta}_{\jmath,\subi}+
\widehat{\mu}_\jmath(\balpha_i)\Big),\quad \widehat{\mu}_\jmath(\balpha_i)=
\widehat{\blambda}_{i,\subi}'\widehat{\bb}_{\jmath,\subi},\quad \text{where}\\[1em]
(\widehat{\bbeta}_{\jmath,\subi}',\; \widehat{\bb}_{\jmath,\subi}')'=
\argmax_{(\bbeta', \bb')'\in\mathbb{R}^{\ttd_z+\ttd_\lambda}}\;
\sum_{\ell\in\mathcal{N}_i}
d_\ell(\jmath)\mathcal{L}_{\tty}\Big(\psi_{\tty}(\bz_{\ell}'\bbeta+\widehat{\blambda}_{\ell,\subi}'\bb),\; y_{\ell}\Big).
\end{split}
\]

The treatment equation \eqref{SA-eq: treatment} can be treated similarly with a proper choice of the link function $\bpsi^{-1}_{\tts}(\cdot)$ and the quasi-likelihood $\mathcal{L}_{\tts}(\cdot,\cdot)$ associated with $\{V_{\tts,\jmath}(\cdot)\}_{\jmath\in\mathcal{J}}$ satisfying $\frac{\partial}{\partial\zeta_{\jmath}}\mathcal{L}_{\tts}(\bpsi_{\tts}(\bm{\zeta}),\bm{d})=\frac{d(\jmath)-\psi_{\tts,\jmath}(\bm{\zeta})}{V_{\tts,\jmath}(\bm{\zeta})}$.
The predicted conditional treatment probability is given by
\[
\widehat{\bp}_{i}=\bpsi_{\tts}\Big(\widehat{\bgamma}_i\bz_{i}+\widehat{\bm{\rho}}(\balpha_i)\Big).
\]

\subsubsection{Step 3: Counterfactual Analysis}

The final step is to conduct counterfactual analysis with the preparation above. Consider the mean of the potential outcome at treatment level $\jmath$ for treatment group $\jmath'$: $\theta_{\jmath,\jmath'}:=\E[y_i(\jmath)|s_i=\jmath']$. The estimator of $\theta_{\jmath,\jmath'}$ is
\[
\widehat{\theta}_{\jmath,\jmath'}=
\E_n\left[\frac{d_{i}(\jmath')\widehat{\varsigma}_{i,\jmath}}{\widehat{p}_{\jmath'}}+\frac{\widehat{p}_{i,\jmath'}}{\widehat{p}_{\jmath'}}\frac{d_{i}(\jmath)(y_{i}-\widehat{\varsigma}_{i,\jmath})}{\widehat{p}_{i,\jmath}}\right].
\]
where the inputs $\widehat{\varsigma}_{i,\jmath}$ and $\widehat{p}_{i,\jmath}$ are obtained from the previous step, $p_{\jmath}=\P(s_{i}=\jmath)$, and 
$\widehat{p}_\jmath=\E_n[d_{i}(\jmath)]$. The variance estimator is

\[
\widehat{\sigma}_{\jmath,\jmath'}^2:=
\E_n\bigg[\frac{d_i(\jmath')(\widehat{\varsigma}_{i,\jmath}-\widehat{\theta}_{\jmath,\jmath'})^2}{\widehat{p}_{\jmath'}^2}\bigg]+
\E_n\bigg[\frac{\widehat{p}_{i,\jmath'}^2d_i(\jmath)(y_i-\widehat{\varsigma}_{i,\jmath})^2}{\widehat{p}_{\jmath'}^2\widehat{p}^2_{i,\jmath}}\bigg].		
\]
Pointwise and uniform inference procedures can be constructed as described in the main paper. 

\subsection{Tuning Parameter Selection}

In Section 3 of the main paper, I propose two possible strategies for selecting the number of nearest neighbors $K$, both of which attemp to minimize the prediction error of the factor-augmented regression in Section \ref{subsubsection: step 2}. This subsection provides more implementational details. For simplicity, the following discussion focuses on the step of estimating the conditional expectation of the potential outcome at treatment level $\jmath$, i.e.,  $\varsigma_{i,\jmath}$, based on least squares method and takes  the number of local principal components $\ttd_\lambda$ as fixed. Let $n_\jmath:=\sum_{i=1}^nd_i(\jmath)$.

\subsubsection{Cross Validation}
Split $\{i: d_i(\jmath)=1\}$ into $L$ roughly equal-sized parts. For the $\ell$th part,  search for the $K$ nearest neighbors of each unit $i$ in this part  among all units that do not belong to the $\ell$th part, and implement local PCA accordingly to obtain the local factor loadings $\widehat{\blambda}_{j,\subi}$ for $j\in\mathcal{N}_i$, if necessary. Then, conduct the local regression as described in Section \ref{subsubsection: step 2}, but only using the data that belong to the other $L-1$ parts. It allows us to construct the estimate of the conditional expectation of the outcome for every unit $i$ in the $\ell$th part. We do this for $\ell=1, 2, \cdots, L$, and the goal is to minimize the cross-validation estimate of the prediction error. 

More formally, let $\kappa:\{i: d_i(\jmath)=1\}\mapsto \{1, \cdots, L\}$ be an indexing function indicating the partition to which each unit is allocated by the randomization, and denote by $\widehat{\varsigma}_{i,\jmath}^{-\kappa(i)}(K)$ the fitted value given a particular choice of $K$, computed the way described above (the $\kappa(i)$th part is removed when fitting the model). Choose $K$ that minimizes 
\[
\mathrm{CV}(K)=\frac{1}{n_\jmath}\sum_{i:d_i(\jmath)=1} \Big(y_i-\widehat{\varsigma}_{i,\jmath}^{-\kappa(i)}(K)\Big)^2.
\]

\subsubsection{Direct Plug-in}

Suppose that $\ttd_{\lambda}=\binom{m-1+\ttd_{\alpha}}{\ttd_{\alpha}}$ in part (e) of Step 1 for some $m\geq 1$ and the integrated mean squared error of $\widehat{\varsigma}_{i,\jmath}$ (conditional on the covariates) approximately takes the following expansion
\[
\mathrm{IMSE}(\widehat{\varsigma}_{i,\jmath})\approx \mathscr{V}\times K^{-1} + \mathscr{B}\times (K/n)^{\frac{2m}{\ttd_{\alpha}}},
\]
where $\mathscr{V}$ and $\mathscr{B}$ correspond to the integrated variance and the integrated squared bias. 
Note that for the classical local polynomial regression, $\mathscr{B}=0$ when $m$ is odd and thus the bias is of higher-order. However, due to the feature of indirect matching, this may not be  true in the context of this paper.
If the conditional expectation function of the outcome is sufficiently smooth, an optimal choice of $K$ takes the following form:  $$K_{\mathtt{opt}}=\Big[\Big(\frac{\ttd_{\alpha}\mathscr{V}}{2m\mathscr{B}}\Big)^{\frac{\ttd_{\alpha}}{2m+\ttd_{\alpha}}}n^{\frac{2m}{2m+\ttd_\alpha}}\Big],$$
where $[\cdot]$ denotes a rounding operator.

In practice, choose an initial $K$, denoted by $K_{\mathtt{ini}}$, based on some rule of thumb. Implement $K$-NN matching and local PCA as outlined in Step 1. Run the local (factor-augmented) regression as described in Section \ref{subsubsection: step 2}, and calculate the variance of $\widehat{\varsigma}_{i,\jmath}$, denote by $\widehat{\mathsf{V}}_i$, for each $i\in\{\ell:d_\ell(\jmath)=1\}$, using  the standard formula for the variance in least squares regression. Then, use the average variance $n_\jmath^{-1}\sum_{i:d_i(\jmath)=1}\widehat{\mathsf{V}}_i$ as an approximate of $K^{-1}\mathscr{V}$. Next, when conducting local PCA in part (e) of Step 1,  extract the next $\binom{m+\ttd_{\alpha}-1}{\ttd_{\alpha}-1}$ local factor loadings (ordered by the magnitude of associated local eigenvalues), denoted by $\widehat{\blambda}_{\ell,\subi}^{\mathsf{B}}$ for $\ell\in\mathcal{N}_i$, and include them as additional regressors in the local regression in Step 2. Denote by $\widehat{\bb}_{\jmath,\subi}^{\mathsf{B}}$ the estimated coefficients of these additional terms. Then, take $n_{\jmath}^{-1}\sum_{i:d_i(\jmath)=1}\mathsf{B}_i$ 
as an approximate of $(K/n)^{\frac{2m}{\ttd_{\alpha}}}\mathscr{B}$, where $\mathsf{B}_i=K^{-1}\sum_{\ell\in\mathcal{N}_i}((\widehat{\blambda}_{\ell,\subi}^{\mathsf{B}})'\widehat{\bb}_{\jmath,\subi}^{\mathsf{B}})^2$. Then, a DPI choice of $K$ is given by
\[
\widehat{K}_{\mathtt{DPI}}=\Big[\Big(\frac{\ttd_{\alpha}\sum_{i:d_i(\jmath)=1}\mathsf{V}_i}{2m\sum_{i:d_i(\jmath)=1}\mathsf{B}_i}\Big)^{\frac{\ttd_{\alpha}}{2m+\ttd_{\alpha}}}K_{\mathtt{ini}}\Big].
\]
Intuitively, when the initial choice $K_{\mathtt{ini}}$ is too small, the sum of variance in the numerator may be large relative to the sum of (squared) bias in the denominator, thus making the resulting choice larger. On the other hand, when $K_{\mathtt{ini}}$ is too large, the numerator is small relative to the denominator, leading to a smaller $K$.

Two practical issues need to be noted. First, in finite samples the leading bias in the local regression in Step 2 may be small while the bias that is theoretically of higher order may be large. In this scenario one may want to extract more factor loadings in local PCA in part (e) of Step 1 to  characterize more bias terms. Second, the remaining bias in local PCA in part (e) of Step 1 may be small relative to the noise and the extracted factor loadings no longer characterize the higher-order approximation terms of interest. In this case one can use a larger initial $K$ to reduce the impact of noise. Alternatively, mimicking the idea of local polynomial regression, one can use the polynomial transformation of leading factor loadings associated with larger eigenvalues to characterize higher-order approximation terms. For instance, suppose that $\ttd_{\alpha}=1$ and $\ttd_{\lambda}=2$. The local PCA in step 1 outputs  $\widehat{\blambda}_{\ell,\subi}=(\widehat{\lambda}_{\ell,0,\subi}, \widehat{\lambda}_{\ell,1,\subi})'$ for $\ell\in\mathcal{N}_i$, which are associated with the two leading eigenvalues. According to the discussion in Section 4.2 of the main paper, $\widehat{\lambda}_{\ell,1,\subi}$ may be viewed as a proxy for the linear term in Taylor expansion. Thus, instead of extracting the third local factor loading, use $\widehat{\lambda}_{\ell,1,\subi}^2$ as a proxy for the quadratic term, and add it to the local regression in Step 2. The other steps to obtain $\widehat{K}_{\mathtt{DPI}}$ remain the same.

%%%%%%%%%%%%%%%%%%%%%%%%%%%%%%%%%%%%%%%%%%%%%%%%%%%%%%%%%%%%%%%%%%%%%%

\section{Main Theoretical Results} \label{SA-sec: main results}

\subsection{Assumptions}

The following analysis is based on the main estimation procedure described in Section \ref{SA-sec: estimation}. 
The first assumption concerns unconfoundedness and overlapping.

\begin{assumption}[Unconfoundedness and Overlap] 
	\label{SA-Assumption: ID-counterfactual}
	$\{(y_i,s_i,\bz_i,\balpha_i)\}_{i=1}^n$ is i.i.d over $i$ and satisfies that (a) $y_i(\jmath)\inde d_i(\jmath')|\bz_i,\balpha_i$, $\forall \jmath,\jmath'\in\mathcal{J}$;
	(b) For all $\jmath\in\mathcal{J}$,  $\P(s_i=\jmath|\bz_i, \balpha_i)\geq p_{\min}>0$ for almost surely $\bz_i$ and $\balpha_i$.
\end{assumption}

The next assumption concerns the structure of the high-rank regressors in Equation \eqref{SA-eq: HD covariate}. It is new in this supplement and is not used in the main paper. 

\begin{assumption}[High-Rank Covariates]
	\label{SA-Assumption: high-rank covariates}
	For $\ell=1, \ldots, \ttd_w$, each $\bw_{i,\ell}$ satisfies that
	\[
	w_{it,\ell}=\hbar_{t,\ell}(\bvrho_{i,\ell})+e_{it,\ell}, \quad 
	\E[e_{it,\ell}|\mathcal{F}_\ell]=0,
	\]
	where $\{\bvrho_{i,\ell}\in\mathbb{R}^{\ttd_{\varrho,\ell}}:1\leq i\leq n\}$ is i.i.d and  $\mathcal{F}_\ell$ is the $\sigma$-field generated by $\{\bvrho_{i,\ell}:1\leq i\leq n\}$ and $\{\hbar_{t,\ell}(\cdot):1\leq t\leq T,1\leq \ell\leq \ttd_w\}$.
	Moreover, for some constant $c_{\min}>0$,
	$$s_{\min}\Big(\frac{1}{n|\mathcal{T}_2|}\sum_{i=1}^{n}\sum_{t\in\mathcal{T}_2}
	\be_{it}\be_{it}'\Big)\geq c_{\min} \quad \text{w.p.a } 1,$$
	where $\be_{it}=(e_{it,1}, \cdots, e_{it,\ttd_w})'$.
\end{assumption}

The condition above is akin to that commonly used in partially linear regression. It ensures that $\bw_{i,\ell}$'s are truly ``high-rank'': after partialling out the ``low-rank'' signals (factor components), these covariates are still non-degenerate, thus achieving identifiability of $\bvth$.
Also note that Assumption \ref{SA-Assumption: high-rank covariates} is general in the sense that the latent variables and latent functions associated with each $\bw_{i,\ell}$ could be different across $\ell$. To ease notation, introduce a $\sigma$-field $\mathcal{F}=\cup_{\ell=0}^{\ttd_w}\mathcal{F}_\ell$ and let $\ttd_{\varrho}$ be the number of \textit{distinct} variables among $\balpha_i,\bvrho_{i,1},\cdots, \bvrho_{i,\ttd_w}$.

The next assumption, as a combination of conditions used in Section \ref{SA-sec: general LPSA} (see Assumption \ref{SA Assumption: Matching}, Assumption \ref{SA Assumption: LPCA} and Lemma \ref{lem: verify SA LPCA}), concerns the regularities of the latent structures of $\bx_i$ and $\bw_i$. Assumptions 2(c), 2(d), 2(e), 3, 4, and 5 in the main paper are a simplified version of Assumption \ref{SA-Assumption: latent structure} that suffices for the basic model. %Also note that Assumption \ref{SA-Assumption: latent structure} is a set of lower-level conditions used for the main analysis, and recall that Section \ref{SA-sec: general LPSA} provides higher-level conditions for local PCA. 

\begin{assumption}[Latent Structure] 
	\label{SA-Assumption: latent structure}\leavevmode
	Let $\bar{m}\geq 2$ and $\nu>0$ be some constants.
	\begin{enumerate}[label=(\alph*)]
		\item For all $1\leq t \leq T$, $\hbar_{t,\ell}(\cdot)$ and $\eta_t(\cdot)$ are $\bar{m}$-times continuously differentiable with all partial derivatives of order no greater than $\bar{m}$ bounded by a universal constant;
		
		\item $\{\balpha_i\}_{i=1}^n$ and 
		$\{\bvrho_{i,\ell}\}_{i=1}^n$ for each $\ell=1,\ldots, \ttd_w$ have compact convex supports with densities bounded and bounded away from zero;
		
		\item Conditional on $\mathcal{F}$, $\{(u_{it}, \be_{it}):1\leq i\leq n,1\leq t\leq T\}$ is independent over $i$ and across $t$ with zero means, and 
		$\max_{1\leq i\leq n,1\leq t\leq T}\E[|u_{it}|^{2+\nu}|\mathcal{F}]<\infty$ and $\max_{1\leq i\leq n,1\leq t\leq T}\E[|e_{it}|^{2+\nu}|\mathcal{F}]<\infty$ a.s. on $\mathcal{F}$;
		
		\item For all $1\leq \ell\leq \ttd_w$, $\{\hbar_{t,\ell}(\cdot)\}_{t\in\mathcal{T}_1}$,
		$\{\eta_t(\cdot)+
		\sum_{\ell=1}^{\ttd_w}\hbar_{t,\ell}(\cdot)
		\vartheta_\ell\}_{t\in\mathcal{T}_1}$, and $\{\eta_t(\cdot)\}_{t\in\mathcal{T}_2}$ evaluated on $\{(\balpha_i,\bvrho_{i,1},\cdots, \bvrho_{i,\ttd_w})\}_{i=1}^n$ are asymptotically nonsingular with respect to $\mathfrak{d}_\infty(\cdot,\cdot)$ and non-collapsing; 
		
		\item For all $1\leq \ell\leq \ttd_w$, 
		$\{\eta_t(\cdot)+
		\sum_{\ell=1}^{\ttd_w}\hbar_{t,\ell}(\cdot)
		\vartheta_\ell\}_{t\in\mathcal{T}_1}$, 
		$\{\eta_t(\cdot)+
		\sum_{\ell=1}^{\ttd_w}\hbar_{t,\ell}(\cdot)
		\vartheta_\ell\}_{t\in\mathcal{T}_2}$,  $\{\hbar_{t,\ell}(\cdot)\}_{t\in\mathcal{T}_1}$, $\{\hbar_{t,\ell}(\cdot)\}_{t\in\mathcal{T}_2}$,  $\{\eta_t(\cdot)\}_{t\in\mathcal{T}_2}$ and  $\{\eta_t(\cdot)\}_{t\in\mathcal{T}_3}$ evaluated on $\{(\balpha_i,\bvrho_{i,1},\cdots, \bvrho_{i,\ttd_w})\}_{i=1}^n$ are nondegenerate up to order $m-1$ for some $2\leq m\leq\bar{m}$.
	\end{enumerate}
\end{assumption}

The last assumption concerns the regularities of the local quasi-maximum likelihood estimation (QMLE) procedure.  Let $\bar{\mathcal{F}}=\mathcal{F}\cup\{\bz_i\}_{i=1}^n$ and $\bepsilon_i=(\epsilon_{i,0},\cdots,\epsilon_{i,J})$. Define  $\mathcal{L}_{\ell,\tty}(\zeta,y)=\frac{\partial^\ell}{\partial \zeta^\ell}\mathcal{L}_{\tty}(\psi_{\tty}(\zeta), y)$ for $\ell=1,2$,   $\bm{\mathcal{L}}_{1,\tts}(\bm{\zeta},\bm{d})=\frac{\partial}{\partial \bm{\zeta}}\mathcal{L}_{\tts}(\bpsi_{\tts}(\bm{\zeta}), \bm{d})$, and 
$\bm{\mathcal{L}}_{2,\tts}(\bm{\zeta},\bm{d})=\frac{\partial^2}{\partial \bm{\zeta}\partial\bm{\zeta}'}\mathcal{L}_{\tts}(\bpsi_{\tts}(\bm{\zeta}), \bm{d})$.
%More notation is needed. Let $\zeta_{jt'}=\bx_{jt'}'\bbeta_x(w)+\beta_0(w)+\blambda_{j,\subi}'\bbeta_{\lambda}(w)$. Thus the conditional mean function can be rewritten as $\pi_{jt'}=\psi(\zeta_{jt'})$. 

\begin{assumption}[QMLE] \label{SA-Assumption: QMLE}
	\leavevmode
	\begin{enumerate}[label=(\alph*)]
		\item For some fixed constant $\Delta>0$,
		\[
		\E\bigg[\max_{1\leq i\leq n}
		\frac{1}{K}\sum_{j=1}^{n}\sup_{|\tilde{\zeta}-\zeta|\leq \Delta}\frac{|(\mathcal{L}_{2,\tty}(\tilde{\zeta},y_{j})-\mathcal{L}_{2,\tty}(\zeta,y_{j}))|\I(j\in\mathcal{N}_i)}{|\tilde{\zeta}-\zeta|}\Big|\bar{\mathcal{F}},\{\bx_i,\bw_i\}_{i=1}^n
		\bigg]
		\lesssim_\P 1,
		\]
		and the same condition also holds for every element of  $\bm{\mathcal{L}}_{2,\tts}(\bm{\zeta},\bm{d})$;
		
		\item $\mathcal{L}_{2,\tty}(\zeta,y)<0$ for $\zeta\in\mathbb{R}$ and $y\in\mathcal{Y}$, and $\bm{\mathcal{L}}_{2,\tts}(\bm{\zeta},\bm{d})$ is negative definite for $\bm{\zeta}\in\mathbb{R}^{J}$ and $\bm{d}\in\{0,1\}^{J+1}$;
		
		\item For all $\jmath\in\mathcal{J}$, $\psi_{\tty}(\cdot)$, $\psi_{\tts,\jmath}(\cdot)$, $V_{\tty}(\cdot)$ and $V_{\tts,\jmath}(\cdot)$ are twice continuously differentiable, $V_{\tty}(\psi_{\tty}(\bz'\bbeta_{\jmath}+\mu_{\jmath}(\balpha)))>0$, and $V_{\tts,\jmath}(\bgamma\bz+\bm{\rho}(\balpha))>0$ 
		%and  $\psi_{\tty}'(\bz'\bbeta_{\jmath}+\mu_{\jmath}(\balpha))\neq 0$ 
		over the support of $\balpha$ and $\bz$;
		
		\item For all $\jmath\in\mathcal{J}$, $\mu_{\jmath}(\cdot), \rho_{\jmath}(\cdot)$ are $\bar{m}$-times continuously differentiable;
		
		\item $\bz_i$ has a compact support and satisfies   
		$\E[\tilde{\bz}_i\tilde{\bz}_i'|\balpha_i]>0$ a.s. for $\tilde{\bz}_i=\bz_i-\E[\bz_i|\balpha_i]$. Conditional on $\bar{\mathcal{F}}$, $\{(\bepsilon_i,\bv_i)\}_{i=1}^n$ is independent across $i$ with zero means and independent of $\{(\bx_i, \bw_i)\}_{i=1}^n$, and $\max_{1\leq i\leq n}
		\E[\|\bepsilon_{i}\|_2^{2+\nu}|\bar{\mathcal{F}}]<\infty$ 
		and $\max_{1\leq i\leq n}
		\E[\|\bv_{i}\|_2^{2+\nu}|\bar{\mathcal{F}}]<\infty$
		a.s. on $\bar{\mathcal{F}}$. 
	\end{enumerate}
\end{assumption}
Parts (d) and (e) above are the same as Assumption 2(a) and 2(b) in the main paper, which suffices for the partially linear model. Part (a), (b) and (c) are additional regularity conditions for generalized linear forms.

%%%%%%%%%%%%%%%%%%%%%%%%%%%%%%%%%%%%%%%%%%%%%%%%%%%%%%%%%%%%%%%

\subsection{Main Results}
Throughout the analysis, I denote  $\delta_{KT}=(K^{1/2}\wedge T^{1/2})/\sqrt{\log (n\vee T)}$, $h_{K,\varrho}=(K/n)^{1/\ttd_{\varrho}}$, $h_{K,\alpha}=(K/n)^{1/\ttd_\alpha}$, and $\underline{h}_{K}=(K/n)^{1/\underline{\ttd}_{\varrho}}$ where $\ttd_{\underline{\varrho}}=\min\{\ttd_{\alpha}, \ttd_{\varrho_1}, \cdots, \ttd_{\varrho_{\ttd_w}}\}$. Recall that $K$ is the number of nearest neighbors and $T$ is the dimensionality of $\bx_i$ and $\bw_{i,\ell}$. As in the main paper, attention is restricted to   $\mathfrak{d}(\cdot,\cdot)=\mathfrak{d}_\infty(\cdot,\cdot)$. I assume that  the number of leading components to be extracted, i.e., $\ttd_\lambda$, takes the following values in the procedure for extracting latent variables (see \ref{SA-subsec: latent variable extraction}): $\ttd_\lambda=\binom{m-1+\ttd_{\varrho,\ell}}{\ttd_{\varrho,\ell}}$ for each $\ell$ in Step (b); $\ttd_\lambda=\binom{m-1+\ttd_{\varrho}}{\ttd_{\varrho}}$ in Step (c); and $\ttd_\lambda=\binom{m-1+\ttd_\alpha}{\ttd_\alpha}$ in Step (e).

To begin with, I focus on the covariates equation \eqref{SA-eq: HD covariate}. 
The following lemma derives the rate of convergence for $\widehat{\bvth}$, which makes it possible to separate the factor component of interest from others in Equation \eqref{SA-eq: HD covariate}.

\begin{lem} \label{SA-lem: slope of covariates}
	Under Assumptions \ref{SA-Assumption: high-rank covariates} and \ref{SA-Assumption: latent structure}, if $\delta_{KT}\underline{h}_{K}^{m-1}\rightarrow\infty$,  $\frac{n^{\frac{4}{\nu}}(\log n)^{\frac{\nu-2}{\nu}}}{T}\lesssim 1$, and $(nT)^{\frac{2}{\nu}}\delta_{KT}^{-2}\lesssim 1$, then 
	$\|\widehat{\bvth}-\bvth\|_2\lesssim_\P \delta_{KT}^{-1}+h_{K,\varrho}^{2m}$.
\end{lem}

\begin{remark}
	This is a by-product of my main analysis. In fact, it shows that the low-dimensional parameter in partially linear regression with a nonlinear factor structure can be consistently estimated. The rate of convergence above may not be sharp, since the calculation is simply based on the convergence rates of the underlying nonparametric estimators. 
	
	Note that the rate condition $\delta_{KT}\underline{h}_K^{m-1}\rightarrow\infty$ ensures that $\delta_{KT}h_{K,\alpha}^{m-1}\rightarrow\infty$, $\delta_{KT}h_{K,\varrho}^{m-1}\rightarrow\infty$, and  $\delta_{KT}h_{K,\varrho_\ell}^{m-1}\rightarrow\infty$ for each $1\leq \ell\leq \ttd_w$. Therefore, each time LPSA is applied in Step 1 of the main estimation procedure, the corresponding rate condition required by results in Section \ref{SA-sec: LPCA} is satisfied.
\end{remark}

The next theorem is the key building block of the main results, which shows that the latent variables (and higher-order transformations thereof) can be estimated up to a rotation.

\begin{thm}[Factor Loadings] \label{SA-thm: relevant FE}
	Under Assumptions \ref{SA-Assumption: high-rank covariates} and \ref{SA-Assumption: latent structure},
	if $\delta_{KT}\underline{h}_{K}^{m-1}\rightarrow\infty$, 
	$\delta_{KT}h_{K,\varrho}^{2m}\lesssim 1$, $\frac{n^{\frac{4}{\nu}}(\log n)^{\frac{\nu-2}{\nu}}}{T}\lesssim 1$, and $(nT)^{\frac{2}{\nu}}\delta_{KT}^{-2}\lesssim 1$, then there exists a matrix $\bH_{\subi}$ such that
	\[
    \max_{1\leq i\leq n}
    \|\widehat{\bLambda}_{\subi}-\bLambda_{\subi}\bH_{\subi}\|_{\max}\lesssim_\P
    \delta_{KT}^{-1}+h_{K,\alpha}^{m}+h_{K,\varrho}^{2m}.
	\]
	Moreover, $1\lesssim_\P \min_{1\leq i\leq n}s_{\min}(\bH_{\subi})\leq \max_{1\leq i\leq n}s_{\max}(\bH_{\subi})\lesssim_\P 1$.
\end{thm}

Given the uniformly consistent estimates of relevant factor loadings, the next theorem derives the uniform convergence rates of estimators of $\varsigma_{i,\jmath}$ and $p_{i,\jmath}$.

\begin{thm}[QMLE]\label{SA-thm: QMLE}
	Under Assumptions \ref{SA-Assumption: high-rank covariates}, \ref{SA-Assumption: latent structure} and \ref{SA-Assumption: QMLE},
	if $\delta_{KT}\underline{h}_{K}^{m-1}\rightarrow\infty$,
	$\delta_{KT}h_{K,\varrho}^{2m}\lesssim 1$, $\frac{n^{\frac{4}{\nu}}(\log n)^{\frac{\nu-2}{\nu}}}{T}\lesssim 1$, and $(nT)^{\frac{2}{\nu}}\delta_{KT}^{-2}\lesssim 1$, 
	then for each $\jmath\in\mathcal{J}$, $\max_{1\leq i\leq n}|\widehat{\varsigma}_{i,\jmath}-\varsigma_{i,\jmath}|\lesssim_\P\delta_{KT}^{-1}+h_{K,\alpha}^{m}+h_{K,\varrho}^{2m}$ and
	$\max_{1\leq i\leq n}|\widehat{p}_{i,\jmath}-p_{i,\jmath}|\lesssim_\P\delta_{KT}^{-1}+h_{K,\alpha}^{m}+h_{K,\varrho}^{2m}$. A detailed asymptotic expansion is given by Equation \eqref{eq: asymptotic expansion}.
\end{thm}

With these preparations, I am ready to construct  asymptotic normality of the estimator of the counterfactual mean of the potential outcome.

%If the propensity score estimator is appropriately constructed, then it turns out that by construction of this doubly robust estimator, the first-stage error can be ignored under weak conditions. This idea is used, e.g., \cite{Farrell_2015_JoE} and also closely related to the recent literature on robust inference based on machine learning methods \citep[e.g.][]{Belloni-Chernozhukov-Hansen_2014_RES,Chernozhukov-et-al_2018_EJ}
%A carefully crafted sample splitting scheme will be appealing fot simplying the analysis. It is detailed in the following figure for the binary case:

\begin{thm}[Pointwise Inference] 
	\label{SA-thm: pointwise inference}
	Under Assumptions \ref{SA-Assumption: ID-counterfactual}, \ref{SA-Assumption: high-rank covariates}, \ref{SA-Assumption: latent structure}, and \ref{SA-Assumption: QMLE}, if 
	$\delta_{KT}\underline{h}_{K}^{m-1}\rightarrow\infty$, 
	$\delta_{KT}h_{K,\varrho}^{2m}\lesssim 1$, $\frac{n^{\frac{4}{\nu}}(\log n)^{\frac{\nu-2}{\nu}}}{T}\lesssim 1$, $(nT)^{\frac{2}{\nu}}\delta_{KT}^{-2}\lesssim 1$, and 
	%(i) $\E_n[(\widehat{P}_{it'}-P_{it'})^2]=o_\P(1)$, (ii) $\E_n[(\widehat{L}_{it'}-L_{it'})^2]=o_\P(1)$,
	$\sqrt{n}(\delta_{KT}^{-2}+h_{K,\alpha}^{2m}+h_{K,\varrho}^{4m})=o(1)$, then
	\begin{enumerate}
		\item 
		$\sqrt{n}(\widehat{\theta}_{\jmath,\jmath'}-\theta_{\jmath,\jmath'})=
		\frac{1}{\sqrt{n}}\sum_{i=1}^{n}\varphi_{i,\jmath,\jmath'}
		+o_\P(1)$,
		where $\varphi_{i,\jmath,\jmath'}:=
		\frac{d_i(\jmath')(\varsigma_{i,\jmath}-\theta_{\jmath,\jmath'})}{p_{\jmath'}}+
		\frac{p_{i,\jmath'}}{p_{\jmath'}}\frac{d_i(\jmath)(y_{i}-\varsigma_{i,\jmath})}{p_{i,\jmath}}$;
		
		\item 	$\sqrt{n}(\widehat{\theta}_{\jmath,\jmath'}-\theta_{\jmath,\jmath'})/\widehat{\sigma}_{\jmath,\jmath'}\rightsquigarrow\mathsf{N}(0,1)$.
	\end{enumerate}	
	\end{thm}

%%%%%%%%%%%%%%%%%%%%%%%%%%%%%%%%%%%%%%%%%%%%%%%%%%%%%%%%%
%\section{Extensions} \label{SA-sec: extension}
%\subsection{Uniform Inference on Counterfactual Distribution}
Finally, as in the main paper, I consider uniform inference for counterfactual distributions and functionals thereof. In this specific scenario, the original outcome $y_i$ is transformed by functions in $\mathcal{G}=\{\I(\cdot\leq \tau):\tau\in\mathcal{Y}\}$. I will write  $y_{i,\tau}(\jmath)=\I(y_i(\jmath)\leq \tau)$ and $y_{i,\tau}=\I(y_i\leq \tau)$. Accordingly, for Equation \ref{SA-eq: outcome}, I re-define  $\psi_{\tty}^{-1}(\varsigma_{i,\jmath,\tau})=\bz_i'\bbeta_{\jmath,\tau}+\mu_{\jmath,\tau}(\balpha_i)$ where $\varsigma_{i,\jmath,\tau}=\P(y_i(\jmath)\leq \tau|\bz_i,\balpha_i)$. Let  $\theta_{\jmath,\jmath'}(\tau)=\P(y_i(\jmath)\leq \tau|s_i=\jmath')$. The parameter of interest is  $\theta_{\jmath,\jmath'}(\cdot)=\P(y_i(\jmath)\leq \cdot|s_i=\jmath')$, which is understood as a functional parameter in $\ell^\infty(\mathcal{Y})$, a space of bounded functions on $\mathcal{Y}$ equipped with sup-norm. I need to slightly strengthen some conditions in Assumption \ref{SA-Assumption: QMLE}.

\begin{assumption}[QMLE, Uniform Inference] \label{SA-Assumption: QMLE, uniform}
	\leavevmode
	\begin{enumerate}
		\item For some fixed constant $\Delta>0$,
		\[
		\E\bigg[\sup_{\tau\in\mathcal{Y}}\max_{1\leq i\leq n}
		\frac{1}{K}\sum_{j=1}^{n}\sup_{|\tilde{\zeta}-\zeta|\leq \Delta}\frac{|(\mathcal{L}_{2,\tty}(\tilde{\zeta},y_{j,\tau})-\mathcal{L}_{2,\tty}(\zeta,y_{j,\tau}))|\I(j\in\mathcal{N}_i)}{|\tilde{\zeta}-\zeta|}\Big|\bar{\mathcal{F}}\bigg]
		\lesssim_\P 1;
		\]
		
		\item For every $\tau\in\mathcal{Y}$, $\mu_{\jmath,\tau}(\cdot)$ is $\bar{m}$-times continuously differentiable with all partial derivatives of order no greater than $\bar{m}$ bounded by a universal constant, and $\mu_{\jmath,\tau}(\cdot)$ is Lipschitz with respect to $\tau$ uniformly over the support of $\balpha_i$.
		
		%\item Conditional on $\bar{\mathcal{W}}_n$, $(\epsilon_i,v_i)$ have mean zero and are independent across $i$ and independent of $(\bx_i,\bw_i)$. 
	\end{enumerate}
\end{assumption}

\begin{thm}[Uniform Inference]\label{SA-thm: uniform inference}
	Under Assumptions \ref{SA-Assumption: ID-counterfactual}-\ref{SA-Assumption: QMLE, uniform}, if $\delta_{KT}\underline{h}_{K}^{m-1}\rightarrow\infty$, $\delta_{KT}h_{K,\varrho}^{2m}\lesssim 1$, $\frac{n^{\frac{4}{\nu}}(\log n)^{\frac{\nu-2}{\nu}}}{T}\lesssim 1$, $(nT)^{\frac{2}{\nu}}\delta_{KT}^{-2}\lesssim 1$, and  $\sqrt{n}(\delta_{KT}^{-2}+h_{K,\alpha}^{2m}+h_{K,\varrho}^{4m})=o(1)$, then
	\[
	\sqrt{n}\Big(\theta_{\jmath,\jmath'}(\cdot)-\theta_{\jmath,\jmath'}(\cdot)\Big)=\frac{1}{\sqrt{n}}\sum_{i=1}^{n}\varphi_{i,\jmath,\jmath'}(\cdot)+o_\P(1)\rightsquigarrow \mathsf{Z}_{\jmath,\jmath'}(\cdot)\quad
	\text{in }\; \ell^\infty(\mathcal{Y}),
	\]
	where $\varphi_{i,\jmath,\jmath'}(\cdot):=
	\frac{d_i(\jmath')(\varsigma_{i,\jmath,\cdot}-\theta_{\jmath,\jmath'}(\cdot))}{p_{\jmath'}}+
	\frac{p_{i,\jmath'}}{p_{\jmath'}}\frac{d_i(\jmath)(y_{i,\cdot}-\varsigma_{i,\jmath,\cdot})}{p_{i,\jmath}}$ and $\mathsf{Z}_{\jmath,\jmath'}(\cdot)$ is a zero-mean Gaussian process with covariance kernel $\E[\varphi_{i,\jmath,\jmath'}(\tau_1)\varphi_{i,\jmath,\jmath'}(\tau_2)]$
	for $\tau_1,\tau_2\in\mathcal{Y}$.
\end{thm}

As an immediate result of the above theorem, the following corollary shows  inference on functionals of counterfactual distributions.

\begin{coro}[Functional Delta Method]\label{SA-coro: functional delta method}
	Let the conditions in Theorem \ref{SA-thm: uniform inference} hold. Consider the parameter $\theta$ as an element of a
	parameter space $D\theta\subseteq \ell^\infty(\mathcal{Y})$, a function space of bounded functions on $\mathcal{Y}$, with $D\theta$ containing the true value $\theta_{\jmath,\jmath'}$. Let a functional $\Psi(\theta)$ mapping $D\theta$ to $\ell^\infty(\mathcal{Q})$ be Hadamard differentiable in $\theta$ at $\theta_{\jmath,\jmath'}$ with derivative
	$\Psi'_\theta$. Then,
	$|\sqrt{n}(\Psi(\widehat{\theta}_{\jmath,\jmath'})(\cdot)-\Psi(\theta_{\jmath,\jmath})(\cdot))-
	n^{-1/2}\sum_{i=1}^{n}\Psi'_{\theta}(\varphi_{i,\jmath,\jmath'})(\cdot)|=o_\P(1)$ and $\sqrt{n}(\Psi(\widehat{\theta}_{\jmath,\jmath'})(\cdot)-\Psi(\theta_{\jmath,\jmath'})(\cdot))\rightsquigarrow\Psi'_\theta(\mathsf{Z}_{\jmath,\jmath'})(\cdot)$ that is a Gaussian process  in $\ell^\infty(\mathcal{Q})$ with mean zero and covariance kernel defined by the limit of the second
	moment of $\Psi'_\theta(\varphi_{i,\jmath,\jmath'})$.
\end{coro}

To make the above result practically feasible, consider a multiplier bootstrap procedure which is discussed extensively in the literature (\citealp{Chernozhukov_2013_ECMA, Donald-Hsu_2014_JoE, Ao-Calonico-Lee_2019_JBES}). For completeness, I state it as another corollary. Let $\{\omega_i\}_{i=1}^n$ be
a sequence of i.i.d. random variables with mean zero and variance one which are  independent of the data. Define
$$\widehat{\varphi}_{i,\jmath,\jmath'}(\cdot)=
\frac{d_i(\jmath')(\widehat{\varsigma}_{i,\jmath,\cdot}-\widehat{\theta}_{\jmath,\jmath'}(\cdot))}{\widehat{p}_{\jmath'}}+
\frac{\widehat{p}_{i,\jmath'}}{\widehat{p}_{\jmath'}}\frac{d_i(\jmath)(y_{i,\cdot}-\widehat{\varsigma}_{i,\jmath,\cdot})}{\widehat{p}_{i,\jmath}}.$$ 

\begin{coro}[Multiplier Bootstrap] \label{SA-coro: multiplier bootstrap}
	Let the conditions of Theorem \ref{SA-thm: uniform inference} hold. Then, conditional on the data, $n^{-1/2}\sum_{i=1}^{n}\omega_i\widehat{\varphi}_{i,\jmath,\jmath'}(\cdot)\rightsquigarrow\mathsf{Z}_{\jmath,\jmath'}(\cdot)$ that is the Gaussian process defined in Theorem \ref{SA-thm: uniform inference} with probability approaching one. 
	
	Moreover, if 
	the conditions in Corollary \ref{SA-coro: functional delta method} hold and there exists an estimator $\widehat{\Psi_\theta'(\varphi}_{i,\jmath,\jmath'})$ such that
    $\sup_{y\in\mathcal{Y}}\max_{1\leq i\leq n}|\widehat{\Psi_\theta'(\varphi}_{i,\jmath,\jmath'})(y)-\Psi_\theta'(\varphi_{i,\jmath,\jmath'})(y)|=o_\P(1)$. Then, conditional on the data,
    $\frac{1}{\sqrt{n}}\sum_{i=1}^n\omega_i\widehat{\Psi_\theta'(\varphi}_{i,\jmath,\jmath'})(\cdot)\rightsquigarrow\Psi_\theta'(\mathsf{Z}_{\jmath,\jmath'})(\cdot)$
	with probability approaching one.
\end{coro}

%%%%%%%%%%%%%%%%%%%%%%%%%%%%%%%%%%%%%%%%%%%%%%%%%%%%%%%

\section{Proofs} \label{SA-sec: proofs}

\subsection{Proofs for Section \ref{SA-sec: general LPSA}}

\subsubsection*{Proof of Lemma \ref{lem: direct matching}}
\begin{proof}
	Let $U_K(\bxi_0)=\max_{1\leq k\leq K}\|\bxi_{j_k^*(\bxi_0)}-\bxi_0\|_2$. Define a cube around $\bxi_0$: $\mathcal{H}_\zeta(\bxi_0)=[\bxi_0-\zeta,\, \bxi_0+\zeta)\cap\mathcal{X}_{\xi}$, where $\zeta=(\frac{C'K}{f_{\xi,\min}n})^{1/\ttd_\xi}$ for some absolute constant $C'>1$ and $f_{\xi,\min}$ denotes the minimum of the density of $\bxi_i$. Let $F$ and $F_n$ denote the population and empirical distribution functions for $\bxi_i$ respectively. Specifically, since the density is strictly positive, 
	$\inf_{\bxi_0\in\mathcal{X}_\xi}F(\mathcal{H}_\zeta(\bxi_0))\geq \min\{f_{\xi,\min} \zeta^{\ttd_{\xi}}, 1\}>\frac{K}{n}$.
	On the other hand,
	\begin{align*}
	\P\Big(\sup_{\bxi_0\in\mathcal{X}_{\xi}}U_K(\bxi_0)>\zeta\Big)
	&\leq \P\bigg(\exists \bxi_0\in\mathcal{X}_{\xi}, F_n\Big(\mathcal{H}_\zeta(\bxi_0)\Big)<\frac{K}{n}\bigg)\\
	%&=\P\bigg(\exists \bxi_0\in\mathcal{X}_{\xi}, F_n\Big(\mathcal{H}_\zeta(\bxi_0)\Big)-F\Big(\mathcal{H}_\zeta(\bxi_0)\Big)<\frac{K}{n}-F\Big(\mathcal{H}_\zeta(\bxi_0)\Big)\bigg)\\
	&\leq\P\bigg(\exists \bxi_0\in\mathcal{X}_{\xi}, \Big|F_n\Big(\mathcal{H}_\zeta(\bxi_0)\Big)-F\Big(\mathcal{H}_\zeta(\bxi_0)\Big)\Big|>F\Big(\mathcal{H}_\zeta(\bxi_0)\Big)
	-\frac{K}{n}\bigg)\\
	%&\leq\P\bigg(\exists \bxi_0\in\mathcal{X}_{\xi}, \Big|F_n\Big(\mathcal{H}_\zeta(\bxi_0)\Big)-F\Big(\mathcal{H}_\zeta(\bxi_0)\Big)\Big|>\min\Big\{\frac{(C'-1)K}{n},1-\frac{K}{n}\Big\}\bigg)\\
	&\leq\P\bigg(\sup_{\bxi_0\in\mathcal{X}_{\xi}} \Big|F_n\Big(\mathcal{H}_\zeta(\bxi_0)\Big)-F\Big(\mathcal{H}_\zeta(\bxi_0)\Big)\Big|>\min\Big\{\frac{(C'-1)K}{n},1-\frac{K}{n}\Big\}\bigg).
	\end{align*}
	Define the oscillation modulus $\omega_n(\zeta):=\sup_{\bxi_0\in\mathcal{X}_\xi}
	\sqrt{n}\Big(F_n\Big(\mathcal{H}_{\zeta}(\bxi_0)\Big)-F\Big(\mathcal{H}_\zeta(\bxi_0)\Big)\Big)$.
	By \citet[Theorem 2.3]{Stute_1984_AoP}, if $\frac{(n/K)\log (n/K)}{n}=o(1)$
	and $\frac{K\log n}{n}=o(1)$, then
	$\omega_n(\zeta)\lesssim_\P\sqrt{\zeta^{\ttd_\xi}\log \zeta^{-\ttd_{\xi}}}$.
	This suffices to show that the probability on the last line goes to zero.
	
	On the other hand, since the density of $\bxi_i$ is bounded from above as well, it follows similarly that $\inf_{\bxi_0\in\mathcal{X}_\xi}U_K(\bxi_0)\geq c(K/n)^{1/\ttd_\xi}$ with probability approaching one.
\end{proof}

\subsubsection*{Proof of Lemma \ref{lem: matching discrepancy lower bound}}
\begin{proof}
	By definition, $\max_{1\leq k\leq K}\|\bxi_i-\bxi_{j_k(i)}\|_2\geq \max_{1\leq k\leq K}\|\bxi_i-\bxi_{j^*_k(\bxi_i)}\|_2$. The result follows immediately from Lemma \ref{lem: direct matching}.
\end{proof}

\subsubsection*{Proof of Theorem \ref{thm: IMD hom}}
\begin{proof}
	We first notice that for any pair $(i,j)$,
	%\begin{align*}
	$\mathfrak{d}_2^2(\bA^{\dagger}_{\cdot i}, \bA^{\dagger}_{\cdot j})=\frac{1}{T}\|\bA^{\dagger}_{\cdot i}-\bA^{\dagger}_{\cdot j}\|_2^2
	=\frac{1}{T}\|\bL^{\dagger}_{\cdot i}-\bL^{\dagger}_{\cdot j}\|_2^2+
	\frac{1}{T}\|\bveps^\dagger_{\cdot i}-\bveps^\dagger_{\cdot j}\|_2^2
	+\frac{2}{T}(\bL^{\dagger}_{\cdot i}-\bL^{\dagger}_{\cdot j})' (\bveps^\dagger_{\cdot i}-\bveps^\dagger_{\cdot j})$.
	%\end{align*}
	For the second term,
	\begin{align*}
	\frac{1}{T}\|\bveps^\dagger_{\cdot i}-\bveps^\dagger_{\cdot j}\|^2=2\sigma^2+\frac{1}{T}\sum_{t\in\mathcal{T}_1}(\varepsilon_{it}^2-\sigma^2)
	+\frac{1}{T}\sum_{t\in\mathcal{T}_1}(\varepsilon_{jt}^2-\sigma^2)-\frac{2}{T}\sum_{t\in\mathcal{T}_1}\varepsilon_{it}\varepsilon_{jt}.
	\end{align*}
	Let $\zeta_{it}:=\varepsilon_{it}^2-\sigma^2$ and write $\zeta_{it}=\zeta_{it}^-+\zeta_{it}^+$ where $\zeta_{it}^-:=\zeta_{it}\I(\zeta_{it}\leq \tau_n)-\E[\zeta_{it}\I(\zeta_{it}\leq \tau_n)|\mathcal{F}_A]$ and $\zeta^+_{it}:=\zeta_{it}\I(\zeta_{it}>\tau_n)-\E[\zeta_{it}\I(\zeta_{it}>\tau_n)|\mathcal{F}_A]$ for $\tau_n=\sqrt{T/\log n}$.
	Then, for any $\delta>0$, by Bernstein's inequality,
	\begin{align*}
	\P\Big(\Big|\frac{1}{T}\sum_{t\in\mathcal{T}_1}\zeta_{it}^-\Big|>\delta
	\Big|\mathcal{F}_A\Big)\leq
	2\exp\bigg(-\frac{\delta^2/2}{\frac{1}{T^2}\sum_{t\in\mathcal{T}_1}\E[(\zeta_{it}^-)^2|\mathcal{F}_A]
		+\frac{1}{3T}\tau_n\delta}\bigg).
	\end{align*}
	On the other hand,
	\[
	\P\Big(\max_{1\leq i\leq n}
	\Big|\frac{1}{T}\sum_{t\in\mathcal{T}_1}\zeta_{it}^+\Big|>\delta\Big|\mathcal{F}_A\Big)
	\leq n\max_{1\leq i\leq n}\frac{\sum_{t\in\mathcal{T}_1}\E[(\zeta_{it}^+)^2|\mathcal{F}_A]}
	{T^2\delta^2}
	\lesssim \frac{n}{T\tau_n^\nu\delta^2}.
	\]
	Then, by the rate restriction and setting $\delta=\sqrt{\log n/T}$, we have
	$\max_{1\leq i\leq n}\Big|\frac{1}{T}\sum_{t\in\mathcal{T}_1}(\varepsilon_{it}^2-\sigma^2)\Big|\lesssim_\P \sqrt{\frac{\log n}{T}}$.

	Apply this argument to other terms. Specifically,
	for any $i\neq j$, since $\E[\varepsilon_{it}\varepsilon_{jt}|\mathcal{F}_A]=0$, by the rate restriction,
	$\max_{i\neq j}
	\Big|\frac{1}{T}\sum_{t\in\mathcal{T}_1}\varepsilon_{it}\varepsilon_{jt}\Big|\lesssim_\P\sqrt{\frac{\log n}{T}}$.
	Then, we have
	$\max_{i\neq j}\Big|\frac{1}{T}\|\bveps^\dagger_{\cdot i}-\bveps^\dagger_{\cdot j}\|^2-2\sigma^2\Big|\lesssim_\P\sqrt{\frac{\log n}{T}}$.
	Similarly, by the moment condition, the rate restriction and the fact that $\E[(\mu_{t,A}(\bxi_i)-\mu_{t,A}(\bxi_j))(\varepsilon_{it}-\varepsilon_{jt})]=0$ for all $t$ and $i\neq j$,
	$\max_{i\neq j}|\frac{1}{T}(\bL^{\dagger}_{\cdot i}-\bL^{\dagger}_{\cdot j})'(\bveps^\dagger_{\cdot i}-\bveps^\dagger_{\cdot j})|\lesssim_\P\sqrt{\frac{\log n}{T}}$.
	Next, by Lemma \ref{lem: direct matching},
	$\max_{1\leq i\leq n}\max_{1\leq k\leq K}\|\bxi_i-\bxi_{j^*_k(\bxi_i)}\|_2\lesssim_\P (K/n)^{1/\ttd_\xi}$.
	Recall that $\{j_k(i): k=1, \ldots, K\}$ is the $K$ nearest neighbors of unit $i$ in terms of distance between $\bA^{\dagger}_{\cdot i}$ and $\bA^{\dagger}_{\cdot j}$.
	Therefore, by Assumption \ref{SA Assumption: Matching} and conditional homoskedasticity,
	\[
	\max_{1\leq i\leq n}\max_{1\leq k\leq K}
	\frac{1}{T}\|\bA^{\dagger}_{\cdot i}-\bA^{\dagger}_{\cdot j_k(i)}\|_2^2
	\leq
	\max_{1\leq i\leq n}\max_{1\leq k\leq K}
	\frac{1}{T}\|\bA^{\dagger}_{\cdot i}-\bA^{\dagger}_{\cdot j_k^*(\bxi_i)}\|_2^2
	\lesssim_\P (K/n)^{2/\ttd_\xi}+2\sigma^2+\sqrt{\log n/T}.
	\]
	Since
	$\frac{1}{T}\|\bL^{\dagger}_{\cdot i}-\bL^{\dagger}_{\cdot j_k(i)}\|_2^2=
	\frac{1}{T}\|\bA^{\dagger}_{\cdot i}-\bA^{\dagger}_{\cdot j_k(i)}\|_2^2
	-\frac{1}{T}\|\bveps^\dagger_{\cdot i}-\bveps^\dagger_{\cdot j_k(i)}\|_2^2
	-\frac{2}{T}(\bL^{\dagger}_{\cdot i}-\bL^{\dagger}_{\cdot j_k(i)})' (\bveps^\dagger_{\cdot i}-\bveps^\dagger_{\cdot j_k(i)})$, $\max_{1\leq i\leq n}\max_{1\leq k\leq K}\mathfrak{d}_2(\bL^\dagger_{\cdot i},\bL^\dagger_{\cdot j})=o_\P(1)$.
	
	By Assumption \ref{SA Assumption: Matching}(d), 
	for any $\epsilon>0$ and $\eta>0$, there exists some $\Delta_\epsilon>0$ and $M_\epsilon>0$ such that $\P(\max_{1\leq i\leq n}\max_{\mathfrak{d}_2(\bL^\dagger_{\cdot i},\bL^\dagger_{\cdot j})<\Delta_\epsilon}\|\bxi_i-\bxi_j\|_2>\epsilon)<\eta/2$ for all $n,T>M_\epsilon$. On the other hand, we also have that there exists $M_\epsilon'>0$ such that $\P(\max_{1\leq i,j\leq n}\max_{1\leq k\leq K}\mathfrak{d}_2(\bL^\dagger_{\cdot i},\bL^\dagger_{\cdot j_k(i)})>\Delta_\epsilon)<\eta/2$ for all $n,T>M_\epsilon'$. 
	Then, for all $n,T>M_\epsilon\vee M_\epsilon'$, $\P(\|\bxi_i-\bxi_{j_k(i)}\|_2>\epsilon)<\eta$, i.e., $\max_{1\leq i\leq n}\max_{1\leq k\leq K}\|\bxi_i-\bxi_{j_k(i)}\|_2=o_\P(1)$. Then, we consider a local linearization around $\bxi_i$.
	By Assumption \ref{SA Assumption: Matching}(d), 
	\begin{align*}
	\|\bxi_i-\bxi_{j_k(i)}\|_2^2
	&\lesssim_\P\frac{1}{T}\Big\|\nabla\bmu^\dagger_{A}(\bxi_i)'(\bxi_i-\bxi_{j_k(i)})+\frac{1}{2}(\bxi_i-\bxi_{j_k(i)})'\nabla^2\bmu_A(\tilde{\bxi})'(\bxi_i-\bxi_{j_k(i)})\Big\|_2^2\\
	&=\frac{1}{T}\|\bL^{\dagger}_{\cdot i}-\bL^{\dagger}_{\cdot j_k(i)}\|_2^2,
	%&=\frac{1}{T}\|\bA^{\dagger}_{\cdot i}-\bA^{\dagger}_{\cdot j_k(i)}\|_2^2-\frac{1}{T}\|\bveps^\dagger_{\cdot i}-\bveps^\dagger_{\cdot j_k(i)}\|_2^2
	%-\frac{2}{T}(\bL^{\dagger}_{\cdot i}-\bL^{\dagger}_{\cdot j_k(i)})' (\bveps^\dagger_{\cdot i}-\bveps^\dagger_{\cdot j_k(i)}),
	\end{align*}
	where $\nabla^2\bmu_A(\tilde{\bxi})$ is a $T\times \ttd_\xi\times \ttd_\xi$ array with the $t$th sheet given by the Hessian matrix of $\mu_{t,A}(\cdot)$ with respect to $\bxi$ evaluated at some appropriate point $\tilde{\bxi}_{i,t}$ between $\bxi_i$ and $\bxi_{j_k(i)}$, and $\tilde{\bxi}=(\tilde{\bxi}_{i,1}', \cdots, \tilde{\bxi}_{i,T}')'$.   
	Then, the result follows.
\end{proof}

\subsubsection*{Proof of Theorem \ref{thm: IMD hsk}}
\begin{proof}
	Recall that $\mathcal{N}_{\bxi_i}^*=\{j_k^*(\bxi_i):1\leq k\leq K\}$ denotes the nearest neighbors of unit $i$ in terms of the Euclidean distance between $\bxi_j$'s and $\bxi_i$. Immediately,
	\begin{alignat}{2}
	&\max_{1\leq i\leq n}\max_{1\leq k\leq K} \max_{l\neq i, j_k(i)}
	&&\Big|\frac{1}{T}(\bA^{\dagger}_{\cdot j_k(i)}-\bA^{\dagger}_{\cdot i})'\bA^{\dagger}_{\cdot l}\Big|\nonumber\\
	%\leq& \max_{1\leq i\leq n}\max_{1\leq k\leq K} \max_{l\neq i, j^*_k(\bxi_i)}
	%&&\Big|\frac{1}{T}(\bA^{\dagger}_{\cdot j_k^*(\bxi_i)}-\bA^{\dagger}_{\cdot i})'\bA^{\dagger}_{\cdot l}\Big|\nonumber\\
	\leq &\max_{1\leq i\leq n}\max_{1\leq k\leq K}\max_{l\neq i, j^*_k(\bxi_i)}
	\Big\{&&\Big|\frac{1}{T}(\bL^{\dagger}_{\cdot j_k^*(\bxi_i)}-\bL^{\dagger}_{\cdot i})'\bL^{\dagger}_{\cdot l}\Big|+
	\Big|\frac{1}{T}(\bL^{\dagger}_{\cdot j_k^*(\bxi_i)}-\bL^{\dagger}_{\cdot i})'\bveps^\dagger_{\cdot l}\Big|+\nonumber\\
	&&&\,\Big|\frac{1}{T}(\bveps^\dagger_{\cdot j_k^*(\bxi_i)}-\bveps^\dagger_{\cdot i})'\bL^{\dagger}_{\cdot l}\Big|+
	\Big|\frac{1}{T}(\bveps^\dagger_{\cdot j_k^*(\bxi_i)}-\bveps^\dagger_{\cdot i})'\bveps^\dagger_{\cdot l}\Big|\Big\}. \label{SA-eq: thm-hsk expansion}
	\end{alignat}
	As in the proof of Theorem \ref{thm: IMD hom}, I apply the truncation argument.
	Let $\zeta_{ijt}:=\varepsilon_{it}\varepsilon_{jt}$ and write $\zeta_{ijt}=\zeta_{ijt}^-+\zeta_{ijt}^+$ where $\zeta_{it}^-:=\zeta_{ijt}\I(\zeta_{ijt}\leq \tau_n)-\E[\zeta_{ijt}\I(\zeta_{ijt}\leq \tau_n)|\mathcal{F}_A]$ and $\zeta^+_{ijt}:=\zeta_{ijt}\I(\zeta_{ijt}>\tau_n)-\E[\zeta_{ijt}\I(\zeta_{ijt}>\tau_n)|\mathcal{F}_A]$ for $\tau_n=\sqrt{T/\log n}$.
	Then, for any $\delta>0$, by Bernstein's inequality,
	\begin{align*}
	\P\Big(\Big|\frac{1}{T}\sum_{t\in\mathcal{T}_1}\zeta_{ijt}^-\Big|>\delta
	\Big|\mathcal{F}_A\Big)\leq
	2\exp\bigg(-\frac{\delta^2/2}{\frac{1}{T^2}\sum_{t\in\mathcal{T}_1}
		\E[(\zeta_{ijt}^-)^2|\mathcal{F}_A]
		+\frac{1}{3T}\tau_n\delta}\bigg).
	\end{align*}
	On the other hand,
	\[
	\P\Big(\max_{1\leq i,j\leq n}
	\Big|\frac{1}{T}\sum_{t\in\mathcal{T}_1}\zeta_{ijt}^+\Big|>\delta\Big|\mathcal{F}_A\Big)
	\leq n^2\max_{1\leq i,j\leq n}\frac{\sum_{t\in\mathcal{T}_1}\E[(\zeta_{ijt}^+)^2|\mathcal{F}_A]}
	{T^2\delta^2}
	\lesssim \frac{n^2}{T\tau_n^\nu\delta^2}.
	\]
	Then, by the rate restriction and setting $\delta=\sqrt{\frac{\log n}{T}}$, we have
	$\max_{1\leq i,j\leq n}\Big|\frac{1}{T}\sum_{t\in\mathcal{T}_1}\varepsilon_{it}\varepsilon_{jt}\Big|\lesssim_\P \sqrt{\frac{\log n}{T}}$.
	Note that in this case the moment condition required is weaker than in Theorem \ref{thm: IMD hom}.
	By similar argument, we conclude that the last three terms in Equation \eqref{SA-eq: thm-hsk expansion} are $O_\P(\sqrt{\log n/T})$. The first term, by Lemma \ref{lem: direct matching}, is bounded by
	\[
	\begin{split}
	%&\max_{1\leq i\leq n}\max_{1\leq k\leq K}\max_{l\neq i, j_k^*(\bxi_i)}
	%\Big|\frac{1}{T}\sum_{t\in\mathcal{T}_1}\Big(\mu_{t,A}(\bxi_i)-\mu_t(\bxi_{j_k^*(\bxi_i)})\Big)\mu_{t,A}(\bxi_l)\Big|\\
	&\max_{1\leq i\leq n}\max_{1\leq k\leq K}\max_{l\neq i, j_k^*(\bxi_i)}
	\Big(\frac{1}{T}\sum_{t\in\mathcal{T}_1}\Big(\mu_{t,A}(\bxi_i)-\mu_{t,A}(\bxi_{j_k^*(\bxi_i)})\Big)^2\Big)^{1/2}
	\Big(\frac{1}{T}\sum_{t\in\mathcal{T}_1}\mu_{t,A}(\bxi_l)^2\Big)^{1/2}
	\leq C(K/n)^{1/\ttd_\xi}
	\end{split}
	\]
	w.p.a. $1$ for some $C>0$.
    It follows that
	$\max_{1\leq i\leq n}\max_{1\leq k\leq K} \mathfrak{d}_\infty(\bA^{\dagger}_{\cdot i}, \bA^{\dagger}_{\cdot j_k(i)})\lesssim_\P
	(K/n)^{1/\ttd_\xi}+\sqrt{\log n/T}$.
	In fact, using the argument in the proof of Theorem \ref{thm: IMD hom} again, the above further implies that
	\begin{equation}\label{SA-eq: thm-hsk intermediate result}
	\max_{1\leq i\leq n}\max_{1\leq k\leq K}\max_{l\neq i, j_k(i)}
	\Big|\frac{1}{T}(\bL^{\dagger}_{\cdot i}-\bL^{\dagger}_{\cdot j_k(i)})'\bL^{\dagger}_{\cdot l}\Big|\lesssim_\P (K/n)^{1/\ttd_\xi}+\sqrt{\log n/T}.
	\end{equation}
	As argued in the proof of Theorem \ref{thm: IMD hom},  $\max_{1\leq i\leq n}\max_{1\leq k\leq K}
	\|\bxi_i-\bxi_{j_k(i)}\|=o_\P(1)$ by Assumption \ref{SA Assumption: Matching}(d).
	In the above expression, for fixed $i$ and $k$,  $l$ could take any value from $1$ to $n$ except $i$ and $j_k(i)$. Thus, I can pick the nearest neighbors of units $i$ and $j_k(i)$ among $\{i':i'\neq i, i'\neq j_k(i)\}$, denoted by $l'$ and $l''$ respectively. Then, since
	\[
	\Big|\frac{1}{T}(\bL^{\dagger}_{\cdot i}-\bL^{\dagger}_{\cdot j_k(i), A})'\bL^{\dagger}_{\cdot i}\Big|\leq
	\Big|\frac{1}{T}(\bL^{\dagger}_{\cdot i}-\bL^{\dagger}_{\cdot j_k(i)})'\bL^{\dagger}_{\cdot l'}\Big|+
	\Big|\frac{1}{T}(\bL^{\dagger}_{\cdot i}-\bL^{\dagger}_{\cdot j_k(i)})'(\bL^{\dagger}_{\cdot i}-\bL^{\dagger}_{\cdot l'})\Big|,
	\]
	using the property of nearest neighbors, I have
	$\max_{1\leq i\leq n}\max_{1\leq k\leq K}
	\Big|\frac{1}{T}(\bL^{\dagger}_{\cdot i}-\bL^{\dagger}_{\cdot j_k(i)})'\bL^{\dagger}_{\cdot i}\Big|\lesssim_\P (K/n)^{1/\ttd_\xi}+\sqrt{\log n/T}$. 
	The same bound also holds for $|\frac{1}{T}(\bL^{\dagger}_{\cdot i}-\bL^{\dagger}_{\cdot j_k(i)})'\bL^{\dagger}_{\cdot j_k(i)}|$. Therefore,
	\[
	\max_{1\leq i\leq n}\max_{1\leq k\leq K}
	\Big|\frac{1}{T}(\bL^{\dagger}_{\cdot i}-\bL^{\dagger}_{\cdot j_k(i)})'(\bL^{\dagger}_{\cdot i}-\bL^{\dagger}_{\cdot j_k(i)})\Big|
	\lesssim_\P (K/n)^{1/\ttd_\xi}+\sqrt{\log n/T}.
	\]
	As in the proof of Theorem \ref{thm: IMD hom}, the second-order expansion combined with Assumption \ref{SA Assumption: Matching}(d) implies that
	$\max_{1\leq i\leq n}\max_{1\leq k\leq K}
	\|\bxi_i-\bxi_{j_k(i)}\|_2^2
	\lesssim_\P (K/n)^{1/\ttd_\xi}+\sqrt{\log n/T}$.
	The proof for the first part is complete.
	
	Now, suppose that Assumption \ref{SA Assumption: Matching}(e) also holds. Denote by $\mathcal{M}_n$ the event on which the non-collapsing condition and non-degeneracy conditions hold. Then, $\P(\mathcal{M}_n)=1-o(1)$. Recall that we already have an intermediate result in Equation \eqref{SA-eq: thm-hsk intermediate result}. On $\mathcal{M}_n$,
	for each $\bxi_i$, given the direction $\bxi_i-\bxi_{j_k(i)}$, I can pick a point $\bL^{\dagger}_{\cdot\ell'}=\bmu_A^\dagger(\bxi_{\ell'}):=(\mu_{t,A}(\bxi_{\ell'}))_{t\in\mathcal{T}_1}$ such that  $\mathscr{P}_{\bxi_i}[\bmu_A(\bxi_{\ell'})]=\nabla\bmu^\dagger_{A}(\bxi_i)(r_n(\bxi_i-\bxi_{j_k(i)}))$ for some $r_n$ and it satisfies that  
	$\frac{1}{T}\|\mathscr{P}_{\bxi_i}[\bmu_A(\bxi_{\ell'})]\|_2^2\geq \underline{c}>0$. In view of the non-degeneracy condition in Assumption  \ref{SA Assumption: Matching}(d), 
	$\|r_n(\bxi_i-\bxi_{j_k(i)})\|_2\geq \underline{c}'>0$ for some constant $\underline{c}'>0$. Suppose that $\ell'\neq i, j_k(i)$. Then, we conclude that on $\mathcal{M}_n$,
	\[
	\underline{c}'\|\bxi_i-\bxi_{j_k(i)}\|_2\leq
	\|r_n(\bxi_i-\bxi_{j_k(i)})\|_2^2
	\lesssim\, |r_n|(\bxi_i-\bxi_{j_k(i)})'\Big(\frac{1}{T}\nabla\bmu^\dagger_{A}(\bxi_i)'\nabla_{\bxi}\bmu^\dagger_{A}(\bxi_i)\Big)(\bxi_i-\bxi_{j_k(i)}).
	\]
	In light of Assumption \ref{SA Assumption: Matching}(d),
	these inequalities hold uniformly over $i$ and $k$. 
	On the other hand, notice that by the second-order expansion, for some constant $\bar{c}>0$,
	\[
	\Big|\frac{1}{T}(\bL^{\dagger}_{\cdot i}-\bL^{\dagger}_{\cdot j_k(i)})'\bL^{\dagger}_{\cdot \ell'}\Big|\geq|r_n|(\bxi_i-\bxi_{j_k(i)})'\Big(\frac{1}{T}\nabla\bmu^\dagger_{A}(\bxi_i)'\nabla_{\bxi}\bmu^\dagger_{A}(\bxi_i)\Big)(\bxi_i-\bxi_{j_k(i)})-\bar{c}\|\bxi_i-\bxi_{j_k(i)}\|_2^2.
 	\]
 	By the nonsingularity condition in Assumption \ref{SA Assumption: Matching}(d), we already have $\max_{i,k}\|\bxi_i-\bxi_{j_k(i)}\|_2=o_\P(1)$.
 	Then the desired result follows.
    Moreover, for each $i$ and $k$, if $\ell'=i$ or $j_k(i)$, then take its nearest neighbor other than $i$ and $j_k(i)$. The additional discrepancy induced does not change the upper bound on the right-hand side. Then, the proof for part (b) is complete.
\end{proof}

\subsubsection*{Proof of Lemma \ref{lem: conditional independence of KNN}}
\begin{proof}
	Let $f_{\widehat{R}_i}(\cdot)$ be the density of $\widehat{R}_i$ and $\delta(z, \mathscr{A})$ be an indicator function that is equal to one if $z\in \mathscr{A}$. We have already defined the set of indices for the $K$ nearest neighbors of unit $i$. Now define $\{j_k(i): K+1\leq k\leq n\}$ as the sequence of units that are outside the neighborhood around $\bA^{\dagger}_{\cdot i}$ of radius $\widehat{R}_i$, again arranged according to the original ordering of $\{\bA^{\dagger}_{\cdot i}\}_{i=1}^n$. For $\widehat{R}_i=r$, define $\mathcal{S}_r=\{\bz: \mathfrak{d}(\bz, \bA^{\dagger}_{\cdot i})<r\}$.
	Notice that a generic unit $j$ is included in $\mathcal{N}_i$ if and only if $\mathfrak{d}(\bA^{\dagger}_{\cdot i}, \bA^{\dagger}_{\cdot j})\leq \widehat{R}_i$.
	Since the original sequence $\{\bA^{\dagger}_{\cdot i}:1\leq i\leq n\}$ is i.i.d across $i$, the joint density of $\{\bxi_{j_k(i)}\}_{k=1}^n$ is
	\[
	\begin{split}
	f(\bv_1, \cdots, \bv_{K-1};\bw_1, \cdots, \bw_{N_K};\bz)
	=n\binom{n-1}{K-1}\prod_{k=1}^{K-1}f_\xi(\bv_k)\int f_{A|\xi}(\ba_{k}|\bv_k)\delta(\ba_{k}, \mathcal{S}_{\widehat{R}_i})d\ba_{k}&\\
	\times\prod_{\ell=K+1}^{n}f_\xi(\bw_\ell)
	\int f_{A|\xi}(\ba_{\ell}|\bw_\ell)\delta(\ba_{\ell}, \bar{\mathcal{S}}_{\widehat{R}_i}^c)d\ba_{\ell}
	\times f_\xi(\bz)\int f_{A|\xi}(\ba|\bz)\delta(\ba, \partial \mathcal{S}_{\widehat{R}_i})d\ba&,
	\end{split}
	\]
	where $f_\xi(\cdot)$ is the density of $\bxi_i$, $f_{A|\xi}(\cdot|\cdot)$ denotes the density of $\bA^{\dagger}_{\cdot i}$ conditional on $\bxi_i$ and $\widehat{R}_i$. $\bar{\mathcal{S}}_{\widehat{R}_i}^c$ is the complement of the closure of $\mathcal{S}_{\widehat{R}_i}$ and $\partial \mathcal{S}_{\widehat{R}_i}$ denotes the boundary of $\mathcal{S}_{\widehat{R}_i}$. On the other hand, the density of $\widehat{R}_i$ is
	\[
	n\binom{n-1}{K-1}G(r)^{K-1}(1-G(r))^{n-K}G'(r), \quad G(r)=\P\Big(\{\bA^{\dagger}_{\cdot j}: \mathfrak{d}(\bA^{\dagger}_{\cdot j}, \bA^{\dagger}_{\cdot i})<r\}\Big).
	\]
	According to the above results, $\{\bxi_{j_k(i)}:1\leq k\leq n\}$ is independent across $k$ conditional on $\widehat{R}_i$ and $\bA^{\dagger}_{\cdot i}$ with the joint conditional density given by
	\[
	\begin{split}
	G'(r)^{-1}f_\xi(\bz)\int f_{A|\xi}(\ba|\bz)\delta(\ba, \partial \mathcal{S}_{\widehat{R}_i})d\ba\times&
	\prod_{k=1}^{K-1}G(r)^{-1}f_\xi(\bv_k)
	\int f_{A|\xi}(\ba_{k}|\bv_k)\delta(\ba_{k}, \mathcal{S}_{\widehat{R}_i})d\ba_{k}\\
	\times&\prod_{\ell=K+1}^{N}(1-G(r))^{-1}f_\xi(\bw_\ell)
	\int f_{A|\xi}(\ba_{\ell}|\bw_\ell)\delta(\ba_{\ell}, \bar{\mathcal{S}}_{\widehat{R}_i}^c)d\ba_{\ell}.
	\end{split}
	\]
\end{proof}

\subsubsection*{Proof of Lemma \ref{lem: number of times for matching}}
\begin{proof}
	Let $\widehat{R}_\xi=\max_{1\leq i\leq n}\max_{1\leq k\leq K}\|\bxi_i-\bxi_{j_k(i)}\|_2$. Then,
	$\I(i\in\mathcal{N}_j)\leq \I(\|\bxi_i-\bxi_j\|_2\leq \widehat{R}_\xi)$. By Theorem \ref{thm: IMD hom} or Theorem \ref{thm: IMD hsk}, 
	$\widehat{R}_\xi\lesssim_\P (K/n)^{1/\ttd_\xi}$. On the other hand, for $C>0$ independent of $n$, as in the proof of Theorem \ref{lem: direct matching}, applying Theorem 2.3 of \cite{Stute_1984_AoP} leads to  $n^{-1}\sum_{j=1}^{n}\I(\|\bxi_i-\bxi_j\|_2\leq C(K/n)^{1/\ttd_\xi})-\P(\|\bxi_i-\bxi_j\|_2\leq C(K/n)^{1/\ttd_\xi})=o_\P(K/n) $ uniformly over $i$. This suffices to show that
	$\max_{1\leq i\leq n}\frac{1}{n}S_K(i)\lesssim_\P K/n$.
\end{proof}

%%%%%%%%%%%%%%%%%%%%%%%%%%%%%%%%%%%%%%%%%%%%%
%%%%%%%%%%%%%%%%%%%%%%%%%%%%%%%%%%%%%%%%%%%%%

\subsubsection*{Proof of Lemma \ref{lem: verify SA LPCA}}
\begin{proof}
	I first show part (a) of Assumption \ref{SA Assumption: LPCA} holds.
	By Lemma \ref{lem: matching discrepancy lower bound}, there exists a constant $\underline{c}>0$ such that with probability approaching one, $\min_{1\leq i\leq n}\max_{1\leq k\leq K}\|\bxi_i-\bxi_{j_k(i)}\|_2\geq \underline{c}(K/n)^{1/\ttd_\xi}$. Also, $\max_{1\leq i\leq n}\max_{1\leq k\leq K}\|\bxi_i-\bxi_{j_k(i)}\|_2\lesssim_\P (K/n)^{1/\ttd_\xi}$ by Theorem \ref{thm: IMD hom} or Theorem \ref{thm: IMD hsk} and the rate condition.
	%Then it implies that with probability approaching one, $\widehat{R}_i$ ranges within an  interval $[\underline{C}(K/n)^{1/\ttd_\xi}, \bar{C}(K/n)^{1/\ttd_\xi}]$ for $\underline{C}, \bar{C}>0$. 	
	Simply let $\blambda(\bxi)$ be the $\ttd_\lambda$ power basis of degree no greater than $m-1$ (including the constant) centered at $\bxi_i$. Then, the first result $\|\blambda_{j_k(i)}\bUpsilon^{-1}\|_{\max}\lesssim_\P 1$ immediately follows. Since $\ttd_\lambda$ is fixed, the upper bound on the maximum singular value also follows. Regarding the lower bound on the minimum singular value, by Lemma \ref{lem: matching discrepancy lower bound} and the argument in the proof of Theorem \ref{thm: IMD hsk}, $\min_{1\leq i\leq n}\widehat{R}_i\geq \underline{c}'(K/n)^{1/\ttd_\xi}$ for some absolute constant $\underline{c}'>0$ w.p.a.1, where $\widehat{R}_i$ is the radius defined in Lemma \ref{lem: conditional independence of KNN}. Therefore, there exists $h=\underline{c}''(K/n)^{1/\ttd_\xi}$ for some small enough absolute constant $\underline{c}''>0$ such that w.p.a.1,   $\mathfrak{d}(\bA_{\cdot i}^{\dagger},\bA_{\cdot j}^{\dagger})\leq \widehat{R}_i$ for all $\|\bxi_i-\bxi_j\|_2\leq h$ and $1\leq i\leq n$. On this event,
	$s_{\min}(K^{-1}\sum_{k=1}^{K}\bUpsilon^{-1}\blambda_{j_k(i)}\blambda_{j_k(i)}'\bUpsilon^{-1})\geq s_{\min}(K^{-1}\sum_{j=1}^{n}\bUpsilon^{-1}\blambda_{j}\blambda_{j}'\bUpsilon^{-1}\I(\|\bxi_i-\bxi_j\|\leq h))$.
	Note that $s_{\min}(n^{-1}\sum_{j=1}^{n}\bUpsilon^{-1}\blambda_{j}\blambda_{j}'\bUpsilon^{-1}\I(\|\bxi_i-\bxi_j\|\leq h))\gtrsim h^{\ttd_\xi}$ w.p.a. 1. Then, the desired lower bound follows.
	
	Next, consider part (b). Conditional on $\widehat{R}_i$, $\{\blambda_{j_k(i)}:1\leq k\leq K\}$ is a bounded independent sequence. Then, by applying Bernstein inequality as before,
	$\max_{1\leq i\leq n}\Big|\frac{1}{K}\bUpsilon^{-1}\bLambda_{\subi}'\bLambda_{\subi}\bUpsilon^{-1}
	%:=
	%\frac{1}{K}\sum_{k=1}^{K}\bUpsilon^{-1}\blambda_{j_k(i)}\blambda_{j_k(i)}'\bUpsilon^{-1}
	- \E_{\mathcal{N}_i}[\tilde{\bUpsilon}^{-1}\tilde{\blambda}_{j_k(i)}\tilde{\blambda}_{j_k(i)}'\tilde{\bUpsilon}^{-1}]\Big|=o_\P(1)$.
 \iffalse
	By change of variables, the limit is equal to
	\[
	\int_{\mathbb{R}^{\ttd_\lambda+1}} \bz(\cdot)\bz'(\cdot)dF_{\tilde{\bxi}_{j_k(i)}|\widehat{R}_i}(\cdot|\widehat{R}_i) \asymp_\P \bI_{\ttd_\lambda}\quad 
	\text{uniformly over } i,
	\]
	where $\bz(\cdot)$ is the $\ttd_\xi$-variate power series up to degree $m-1$ and $\tilde{\bxi}_{j_k(i)}=(\bxi_{j_k(i)}-\bxi_i)/\widehat{R}_i$.
	%Now, simply let $\bLambda_{\subi}$ be  $\tilde{\bLambda}-K^{-1}\biota_K\biota_K'\tilde{\bLambda}$ with the first column excluded. This loading matrix is correctly centered (thus satisfying the normalization condition), and by the previous results, $\frac{1}{K}\bLambda_{\subi}'\bLambda_{\subi}\asymp 1$ with probability approaching one. 
	Then, the proof for part (a) is complete.
	\fi
	By Assumption \ref{SA Assumption: Matching} and Taylor expansion, there exists $\tilde{\bbeta}_{t,\subi}$ for $1\leq t\leq T$ such that 
	$\max_{t\in\mathcal{T}_2}\max_{1\leq i\leq n}\max_{j\in\mathcal{N}_i}\Big|\mu_{t,A}(\bxi_j)-\blambda(\bxi_j)'\tilde{\bbeta}_{t,\subi}\Big|\lesssim_\P h_{K,\xi}^m$.
	Let $\tilde{r}_{t,\subi}(\bxi_j):=\mu_{t,A}(\bxi_j)-
	\tilde{\blambda}(\bxi_j)'\tilde{\bbeta}_{\subi}$ and $\bbeta_{\subi}$ be the coefficients of the $L_2$ projection of $\mu_{t,A}(\cdot)$ onto the space spanned by $\blambda(\cdot)$. Then, 
	$\bbeta_{t,\subi}=\tilde{\bbeta}_{t,\subi}+
	\E_{\mathcal{N}_i}[\tilde{\blambda}(\bxi_j)\tilde{\blambda}(\bxi_j)']^{-1}\E_{\mathcal{N}_i}[\tilde{\blambda}(\bxi_j)\tilde{r}_{t,\subi}(\bxi_j)]
	=:\tilde{\bbeta}_{t,\subi}+\Delta_{t,\subi}$.
	By the previous result,  $\bUpsilon^{-1}\E_{\mathcal{N}_i}[\blambda(\bxi_j)\blambda(\bxi_j)']\bUpsilon^{-1}\gtrsim 1$ uniformly over $i$ w.p.a. 1.   Also, $\bUpsilon^{-1}\tilde{\blambda}(\bxi_j)\lesssim 1$ w.p.a.1 and $\min_{j}\Upsilon_{jj}\asymp h_{K,\xi}^{-(m-1)}$,
	it follows that $\max_{1\leq i\leq n}\max_{t\in\mathcal{T}_2}|\Delta_{t,\subi}|=o_\P(1)$. Thus, the result in part (b) follows.
	
	Finally, for part (c), note that 
	$\mu_{t,A}(\bxi_j)-\blambda(\bxi_j)'\bbeta_{t,\subi}
	=\tilde{r}_{t,\subi}(\bxi_j)-\tilde{\blambda}(\bxi_j)'\E_{\mathcal{N}_i}[\blambda(\bxi_j)\blambda(\bxi_j)']^{-1}\times\E_{\mathcal{N}_i}[\blambda(\bxi_j)\tilde{r}_{t,\subi}(\bxi_j)]$.
	Using the argument for part (b) again, we can see that the second term is bounded by $Ch_{K,\xi}^m$ uniformly over $i$ and $t$ w.p.a.1. Then, the proof is complete.
	%The conditional density of $\bxi_j$ given $\widehat{R}_i$ is bounded, which suffices to show that $\E_{\mathcal{N}_i}[\blambda(\bxi_j)\tilde{r}_{t,\subi}(\bxi_j)]$ is bounded by $Ch_{K,\xi}^m$ for some $C>0$ uniformly over $i$ and $t$. Finally, notice that the number $m$ satisfying the restriction in part (c) that $\delta_{KT}^{-1}/h_{K,\xi}^{m-1}\lesssim 1$ exists by the rate condition on $K$.
\end{proof}

\subsubsection*{Proof of Lemma \ref{lem: operator norm of eps}}
\begin{proof}
	Note that $\bveps_{\subi}$ is a $T\times K$ random matrix. Let $\mathcal{M}_n=\{\widehat{R}_i\}_{i=1}^n\cup\mathcal{F}_A$. By Assumption \ref{SA Assumption: Matching} and row-wise sample splitting, conditional on $\widehat{R}_i$, $\bveps_{\subi}$ has independent columns with mean zero and $\E[\bveps^\ddagger_{\cdot j_k(i)}(\bveps^\ddagger_{\cdot j_k(i)})'|\mathcal{M}_n]=\bSigma_{j_k(i)}$ for $1\leq i\leq n$ such that $\max_{1\leq i\leq n}\|\bSigma_{\subi}\|_2\lesssim_\P 1$ for $\bSigma_{\subi}:=\frac{1}{K}\sum_{k=1}^{K}\bSigma_{j_k(i)}$. 
	Write 
	$\frac{1}{K}\sum_{k=1}^{K}\Big(\bveps^\ddagger_{\cdot j_k(i)}
	(\bveps^\ddagger_{\cdot j_k(i)})'-\bSigma_{j_k(i)}\Big)=
	\frac{1}{K}\sum_{k=1}^{K}(\bH_k+\bT_k)$,
	where $\bH_k:=\bveps_{\cdot j_k(i)}^\ddagger(\bveps^\ddagger_{\cdot j_k(i)})'\I(\|\bveps^\ddagger_{\cdot j_k(i)}\|^2_2\leq CT)-\E[\bveps^\ddagger_{\cdot j_k(i)}(\bveps^\ddagger_{\cdot j_k(i)})'\I(\|\bveps^\ddagger_{\cdot j_k(i)}\|^2_2\leq CT)|\mathcal{M}_n]$ and
	$\bT_k:=\bveps^\ddagger_{\cdot j_k(i)}(\bveps^\ddagger_{\cdot j_k(i)})'\I(\|\bveps^\ddagger_{\cdot j_k(i)}\|_2> CT)-\E[\bveps^\ddagger_{\cdot j_k(i)}(\bveps^\ddagger_{\cdot j_k(i)})'\I(\|\bveps^\ddagger_{\cdot j_k(i)}\|_2> CT)|\mathcal{M}_n]$ for some $C>0$. 
	Regarding the truncated part, by Bernstein's inequality for matrices and union bounds,
	for all $\tau>0$,
	%\[
	%\P\Big(\Big\|\frac{1}{K}\sum_{k=1}^{K}\bH_k\Big\|_2>\tau|\mathcal{M}_n\Big)\leq T\exp\Big(-\frac{\tau^2/2}{CT/K+CT\tau/3K}\Big).
	%\]
	%By union bound, 
	\[
	\P\Big(\max_{1\leq i\leq n}\Big\|\frac{1}{K}\sum_{k=1}^{K}\bH_k\Big\|>\tau\Big|\mathcal{M}_n\Big)\leq
	nT\exp\Big(-\frac{\tau^2/2}{CT/K+CT\tau/3K}\Big),
	\]
	which suffices to show that $\max_{1\leq i\leq n}\|\frac{1}{K}\sum_{k=1}^{K}\bH_k\|_2\lesssim_\P\max\{\sqrt{\log(n\vee T)}(T/K)^{1/2},\log(n\vee T)T/K\}$.
	On the other hand, for the tails,
	\[
	\P\Big(\max_{1\leq i\leq n}\Big\|\frac{1}{K}\sum_{k=1}^{K}\bT_k\Big\|_2>\tau\Big|\mathcal{M}_n\Big)\leq\P\Big(\max_{1\leq i\leq n}\|\bveps^\ddagger_{ \cdot j_k(i)}\|_2^2>CT|\mathcal{M}_n\Big).
	\]
	It will be shown later that the right-hand-side can be made arbitrarily small by choosing a sufficiently large but fixed $C>0$ (not varying as $n$ increases).
	Then, we conclude that $\max_{1\leq i\leq n}\|\frac{1}{K}\bveps_{\subi}\bveps_{\subi}'-\bSigma_{\subi}\|_2\lesssim_\P
	\max\{\sqrt{\log(n\vee T)}(T/K)^{1/2},\log(n\vee T)T/K\}$.
	Combine this with the bound on $\bSigma_{\subi}$, we get
	$\max_{1\leq i\leq n}\|\bveps_{\subi}\|_2\lesssim_\P \sqrt{K}+\sqrt{T\log(n\vee T)}$.
	
	In the end, we show the uniform convergence of the second moment of $\bveps^\ddagger_{\cdot j_k(i)}$ which completes the proof.
	The argument is similar to that used in the proof of Theorem \ref{thm: IMD hom}. 
	Let $\zeta_{it}:=\varepsilon_{it}^2-\sigma_{it}^2$, $\sigma_{it}^2=\E[\varepsilon_{it}^2|\mathcal{M}_n]$ and write $\zeta_{it}=\zeta_{it}^-+\zeta_{it}^+$ where $\zeta_{it}^-:=\zeta_{it}\I(\zeta_{it}\leq \tau_n^2)-\E[\zeta_{it}\I(\zeta_{it}\leq \tau_n^2)]$ and $\zeta^+_{it}:=\zeta_{it}\I(\zeta_{it}>\tau_n^2)-\E[\zeta_{it}\I(\zeta_{it}>\tau_n^2)]$ for $\tau_n=(nT)^{1/(2+\nu)}$.
	Then, for any $\delta>0$, by Bernstein's inequality,
	\begin{align*}
	\P\Big(
	\Big|\frac{1}{T}\sum_{t\in\mathcal{T}_2}\zeta_{it}^-\Big|>\delta|\mathcal{M}_n\Big)\leq
	2\exp\bigg(-\frac{\delta^2/2}{\frac{\tau_n^2}{T^2}\sum_{t\in\mathcal{T}_1}\E[(\zeta_{it}^-)|\mathcal{M}_n]
		+\frac{1}{3T}\tau_n^2\delta}\bigg).
	\end{align*}
	On the other hand, by Markov's inequality,
	\[
	\P\Big(\max_{1\leq i\leq n}
	\Big|\frac{1}{T}\sum_{t\in\mathcal{T}_2}\zeta_{it}^+\Big|>\delta|\mathcal{M}_n\Big)
	\leq n\max_{1\leq i\leq n}\frac{\sum_{t\in\mathcal{T}_1}\E[|\zeta_{it}^+||\mathcal{M}_n]}
	{T\delta}
	\lesssim \frac{n}{\tau_n^\nu\delta}.
	\]
	Set $\delta^2=Cn^{2/(\nu+1)}(\log n)^{\nu/(\nu+1)} /T^{\nu/(\nu+1)}$. 
	Then, $\max_{1\leq i\leq n}
	|\frac{1}{T}\sum_{t\in\mathcal{T}_2}\zeta_{it}|\lesssim_\P\delta\rightarrow 0$ by the rate condition. Since  $\max_{1\leq i\leq n}
	T^{-1}\sum_{t\in\mathcal{T}_2}\sigma_{it}^2\lesssim 1$ a.s., the desired result follows.
	\end{proof}

\subsubsection*{Proof of Lemma \ref{lem: eigenstructure 1st order}}
\begin{proof}
	(i):
	Noting the following decomposition
	\[
	\begin{split}
	\bA_{\subi}\bA_{\subi}'
	=\,&\bF_{\subi}\bLambda_{\subi}'\bLambda_{\subi}\bF_{\subi}'+
	(\br_{\subi}+\bveps_{\subi})(\br_{\subi}+\bveps_{\subi})'+\\
	&\bF_{\subi}\bLambda_{\subi}'(\br_{\subi}+\bveps_{\subi})'+
	(\br_{\subi}+\bveps_{\subi})\bLambda_{\subi}\bF_{\subi}'
	=:\bG_1+\bG_2+\bG_3+\bG_4,
	\end{split}
	\]
	by Weyl's theorem, 
	\[
	s_j(\bG_1)+s_{\min}(\bG_2+\bG_3+\bG_4)\leq s_j(\bG_1+\cdots+\bG_4)\leq
	s_j(\bG_1)+s_{\max}(\bG_2+\bG_3+\bG_4).
	\]
	
	First, note  that
	$s_j(\bG_1)=s_j(
	\bLambda_{\subi}\bF_{\subi}'\bF_{\subi}\bLambda_{\subi}')$.
	By Assumption \ref{SA Assumption: LPCA}, 
    $s_j(\frac{1}{TK}\bG_1)\asymp_\P 1$ uniformly over $i$ for $j=1,\cdots, \ttd_{\lambda,0}$.	
	Regarding $\bG_2$, I will analyze the eigenvalue of each component. Clearly, by Assumption \ref{SA Assumption: LPCA}(c), $\max_{1\leq i\leq n}\|\frac{1}{TK}\br_{\subi}\br_{\subi}'\|_2\lesssim_\P h_{K,\xi}^{2m}$. 
	By Lemma \ref{lem: operator norm of eps},
	$\max_{1\leq i\leq n}\|\frac{1}{TK}\bveps_{\subi}\bveps_{\subi}'\|_2\lesssim_\P \log (n\vee T)K^{-1}+T^{-1}$. By Cauchy-Schwarz inequality, $\max_{1\leq i\leq n}\|\frac{1}{TK}(\bveps_{\subi}\br_{\subi}'+\br_{\subi}\bveps_{\subi}')\|_2\lesssim_\P (\log^{1/2}(T\vee n)K^{-1/2}+T^{-1/2})h_{K,\xi}^m$.
	As a result, $\|\frac{1}{TK}\bG_2\|_2\lesssim_\P h_{K,\xi}^{2m}+\frac{\log(T\vee n)}{K}+\frac{1}{T}$ uniformly over $i$.
	
	Regarding $\bG_3+\bG_4$, note 
	$\|\frac{1}{TK}\bF_{\subi}\bLambda_{\subi}'\bveps_{\subi}'\|_2
	\leq\frac{1}{\sqrt{K}}\frac{1}{\sqrt{T}}\|\bF_{\subi}\|_2\|\frac{1}{\sqrt{T}}
	(\frac{1}{\sqrt{K}}\sum_{k=1}^{K} \blambda_{j_k(i)}(\bveps^\ddagger_{ \cdot j_k(i)})')\|_2$
	and $\max_{1\leq i\leq n}\|\bF_{\subi}\|_2\lesssim_\P\sqrt{T}$. Furthermore, conditional on $\widehat{R}_i$ and $\mathcal{F}_A$, $\varepsilon^\ddagger_{tj_k(i)}$ is independent over $k$ and $t$, and $\max_{1\leq i\leq n}\|\bLambda_{\subi}\|_{\max}\lesssim_\P 1$. Applying Bernstein inequality combined with the truncation argument used before leads to $\max_{1\leq i\leq n}\|\frac{1}{TK}\bF_{\subi}\bLambda_{\subi}'\bveps_{\subi}'\|_2\lesssim_\P \sqrt{\log n\vee T}K^{-1/2}$.
	On the other hand, $\bLambda_{\subi}$ is uncorrelated with $\br_{\subi}$ across $1\leq i\leq K$ by construction, and applying Bernstein inequality leads to
	$\max_{1\leq i\leq n}\frac{1}{TK}\|\bF_{\subi}\bLambda_{\subi}'\br_{\subi}\|_2\lesssim_\P \frac{\sqrt{\log n\vee T}h_{K,\xi}^{m}}{\sqrt{K}}$.
	The above fact suffices to show that
	$\|\frac{1}{TK}(\bG_3+\bG_4)\|_2\lesssim_\P \sqrt{\log n\vee T}(K^{-1/2}+K^{-1/2}h_{K,\xi}^{m})$. 
	Then, the desired result for eigenvalues follows.
    \medskip
    
    (ii):
    For eigenvectors, I use the following decomposition:
    \begin{align}
    \widehat{\bF}_{\subi}-\bF_{\subi}\tilde{\bH}_{\subi}
    =\bigg\{&\frac{1}{TK}\bF_{\subi}\bLambda_{\subi}'\bveps_{\subi}'\widehat{\bF}_{\subi}+
    \frac{1}{TK}\bveps_{\subi}\bLambda_{\subi}\bF_{\subi}' \widehat{\bF}_{\subi}+
    \frac{1}{TK}\bF_{\subi}\bLambda_{\subi}'\br_{\subi}'\widehat{\bF}_{\subi}+\nonumber\\
    &\frac{1}{TK}\br_{\subi}\bLambda_{\subi}\bF_{\subi}'\widehat{\bF}_{\subi}+
    \frac{1}{TK}\br_{\subi}\bveps_{\subi}'\widehat{\bF}_{\subi}+
    \frac{1}{TK}\bveps_{\subi}\br_{\subi}'\widehat{\bF}_{\subi}+\nonumber\\
    &\frac{1}{TK}\br_{\subi}\br_{\subi}'\widehat{\bF}_{\subi}+
    \frac{1}{TK}\bveps_{\subi}\bveps_{\subi}'\widehat{\bF}_{\subi}
    \bigg\}\times \widehat{\bV}_{\subi}^{-1} \label{eq: decomposition}
    \end{align}
    where $\tilde{\bH}_{\subi}=\frac{\bLambda_{\subi}'\bLambda_{\subi}}{K}
    \frac{\bF_{\subi}'\widehat{\bF}_{\subi}}{T}\widehat{\bV}_{\subi}^{-1}$.
    Accordingly, a generic $(t,\ell)$th element of $(\widehat{\bF}_{\subi}-\bF_{\subi}\tilde{\bH}_{\subi})$ for $t\in\mathcal{T}_2$, $1\leq\ell \leq \ttd_\lambda$ can be written as 
    $(J_1+\cdots J_8)/\widehat{v}_{\ell,\subi}$ where
    {\footnotesize
    \begin{alignat*}{2}
    &J_1=\frac{1}{T}\sum_{s\in\mathcal{T}_2}\bff_{t,\subi}'\Big(\frac{1}{K}\sum_{k=1}^{K}\blambda_{j_k(i)}\varepsilon_{j_k(i)s}\Big)\widehat{f}_{s \ell,\subi},\qquad
    &&J_2=\Big(\frac{1}{K}\sum_{k=1}^{K}\varepsilon_{j_k(i)t}\blambda_{j_k(i)}'\Big)
    \Big(\frac{1}{T}\sum_{s\in\mathcal{T}_2}\bff_{s,\subi}\widehat{f}_{s\ell,\subi}\Big),\\
    &J_3=\frac{1}{T}\sum_{s\in\mathcal{T}_2}\bff_{t,\subi}'\Big(\frac{1}{K}\sum_{k=1}^{K}\blambda_{j_k(i)}r_{j_k(i)s}\Big)\widehat{f}_{s\ell,\subi},
    &&J_4=\Big(\frac{1}{K}\sum_{k=1}^{K}r_{j_k(i)t}\blambda_{j_k(i)}'\Big)
    \Big(\frac{1}{T}\sum_{s\in\mathcal{T}_2}\bff_{s,\subi}\widehat{f}_{s\ell,\subi}\Big),\\
    &J_5=\frac{1}{T}\sum_{s\in\mathcal{T}_2}
    \Big(\frac{1}{K}\sum_{k=1}^{K}r_{j_k(i)t}\varepsilon_{j_k(i)s}\Big)\widehat{f}_{s\ell,\subi},
    &&J_6=\frac{1}{T}\sum_{s\in\mathcal{T}_2}
    \Big(\frac{1}{K}\sum_{k=1}^{K}\varepsilon_{j_k(i)t}r_{j_k(i)s}\Big)\widehat{f}_{s\ell,\subi},\\
    &J_7=\frac{1}{T}\sum_{s\in\mathcal{T}_2}
    \Big(\frac{1}{K}\sum_{k=1}^{K}r_{j_k(i)t}r_{j_k(i)s}\Big)\widehat{f}_{s\ell,\subi},
    &&J_8=\frac{1}{T}\sum_{s\in\mathcal{T}_2}
    \Big(\frac{1}{K}\sum_{k=1}^{K}\varepsilon_{j_k(i)t}\varepsilon_{j_k(i)s}\Big)\widehat{f}_{s\ell,\subi}.
    \end{alignat*}.
    }
    
	For $J_1$, first note that
	by assumption $\|\frac{1}{T}\sum_{t\in\mathcal{T}_2}\bff_{t,\subi}\bff_{t,\subi}'\|_2\lesssim_\P 1$ and $\frac{1}{T}\sum_{s\in\mathcal{T}_2}\widehat{f}_{s\ell, \subi}^2=1$.
	Also, 
	$\E_{\mathcal{N}_i}[\frac{1}{K}\sum_{k=1}^{K}{\blambda}_{j_k(i)}\varepsilon_{j_k(i),s}]=0$
	and
	%\begin{split}
	$\E_{\mathcal{N}_i}[\|\frac{1}{K}\sum_{k=1}^{K}\blambda_{j_k(i)}\varepsilon_{j_k(i)s}\|_2^2]
	%\leq \frac{1}{K^2}\sum_{\ell=1}^{\ttd_{\lambda,0}}
	%\E_{\mathcal{N}_i}[(\sum_{k=1}^{K}\lambda_{j_k(i),\ell}
	%\varepsilon_{j_k(i),s})^2]
	%&\leq \frac{1}{K^2}\sum_{\ell=1}^{\ttd_{\lambda,0}}\E\bigg[\Big(\sum_{k=1}^{K}\lambda_{j_k(i),\ell}\varepsilon_{j_k(i)s}\Big)^2+
	%\Big(\frac{1}{K}\sum_{k'=1}^{K}\varepsilon_{j_{k'}(i)s}\sum_{k=1}^{K}\lamb%da_{j_k(i),\ell}\Big)^2-\\
	%&\hspace{6em}2\Big(\sum_{k=1}^{K}\lambda_{j_k(i),\ell}\varepsilon_{j_k(i)s}\Big)
	%\Big(\frac{1}{K}\sum_{k=1}^{K}\lambda_{j_k(i),\ell}\sum_{k'=1}^{K}\varepsilon_{j_k(i)s}\Big)
	%\bigg]\\
	\lesssim_\P K^{-1},
	%\end{split}
	$
	which suffice to show that $J_1\lesssim \sqrt{\log n\vee T}K^{-1/2}$ by the truncation argument given in the proof of Theorem \ref{thm: IMD hsk}.
	$J_2$ can be treated similarly.	
	For $J_3$,
	by definition of $\bF_{\subi}$, $\E_{\mathcal{N}_i}[\frac{1}{K}\sum_{k=1}^{K}\blambda_{j_k(i)}r_{j_k(i)s}]=0$, for all $s\in\mathcal{T}_2$, and $\|\br_{\subi}\|_{\max}\lesssim h_{K,\xi}^m$.  Thus,
	$J_3\lesssim_\P \sqrt{\log n\vee T}K^{-1/2}h_{K,\xi}^{m}$. $J_4$ is treated similarly.
	For $J_5$, $\frac{1}{T}\widehat{\bF}_{\subi}'\widehat{\bF}_{\subi}\lesssim_\P 1$, 
	$\E_{\mathcal{N}_i}[\frac{1}{K}\sum_{k=1}^{K}r_{j_k(i)t}\varepsilon_{j_k(i)s}]=0$,
	and
	$\E_{\mathcal{N}_i}[(\frac{1}{K}\sum_{k=1}^K r_{j_k(i)t}\bveps_{j_k(i)s})^2]
	\lesssim_\P K^{-1}h_{K,\xi}^{2m}$.
	Then, $J_5\lesssim_\P \sqrt{\log n\vee T}K^{-1/2}h_{K,\xi}^{m}$. $J_6$ can be treated similarly.
	For $J_7$, using the bound on $\br_{\subi}$, it is immediate to see $J_7\lesssim_\P h_{K,\xi}^{2m}$.
	For $J_{8,t}:=J_8$, it is easy to see that by Lemma \ref{lem: operator norm of eps},
	$\max_{1\leq i\leq n}\frac{1}{T}\sum_{t\in\mathcal{T}_2}J_{8,t}^2=
	\frac{1}{T^3K^2}\widehat{\bff}_{\ell,\subi}'\bveps_{\subi}\bveps_{\subi}'\bveps_{\subi}\bveps_{\subi}'\widehat{\bff}_{\ell,\subi}
	\lesssim_\P \delta_{KT}^{-4}$.
	In sum, 
	$\frac{1}{T}\|\widehat{\bF}_{\gr{0},\subi}-\bF_{\subi}\tilde{\bH}_{\gr{0},\subi}\|_F^2\lesssim_\P\delta_{KT}^{-2}+h_{K,\xi}^{4m}$.
\medskip

	(iii):
	Define a rotation matrix $\tilde{\bH}_{0,\subi}=\frac{\bLambda_{\gr{0},\subi}'\bLambda_{\gr{0},\subi}}{K}
	\frac{\bF_{\gr{0},\subi}'\widehat{\bF}_{\gr{0},\subi}}{T}\widehat{\bV}_{0,\subi}^{-1}$, where $\widehat{\bV}_{0,\subi}$ is the diagonal matrix of the leading $\ttd_{\lambda,0}$ eigenvalues of $\frac{1}{TK}\bA_{\subi}\bA_{\subi}'$. By the same argument in (i),
	\[
	\frac{\widehat{\bF}_{\gr{0},\subi}'\bF_{\gr{0},\subi}}{T}\frac{\bLambda_{\gr{0},\subi}'\bLambda_{\gr{0},\subi}}{K}\frac{\bF_{\gr{0},\subi}'\widehat{\bF}_{\gr{0}}}{T}
	\rightarrow_\P \diag\{\widehat{v}_{1, \subi}, \cdots, \widehat{v}_{\ttd_{\lambda,0}, \subi}\}.
	\]
	Then, by Assumption \ref{SA Assumption: LPCA}, $\frac{1}{T}\bF_{\gr{0}, \subi}'\widehat{\bF}_{\gr{0},\subi}$
	is of full rank, and thus $\tilde{\bH}_{0, \subi}$ is invertible with probability approach one.
	Insert it into the projection matrix:
	$
	%\begin{split}
	\bP_{\widehat{\bF}_{\gr{0},\subi}}-\bP_{\bF_{\gr{0},\subi}}
	%=&\;\frac{1}{T}\widehat{\bF}_{\gr{0},\subi}\widehat{\bF}_{\gr{0},\subi}'-
	%\frac{1}{T}\bF_{\gr{0},\subi}\Big(\frac{1}{T}\bF_{\gr{0},\subi}'\bF_{\gr{0},\subi}\Big)^{-1}\bF_{\gr{0},\subi}'
	=\frac{1}{T}\widehat{\bF}_{\gr{0},\subi}\widehat{\bF}_{\gr{0},\subi}'-
	\frac{1}{T}\bF_{\gr{0},\subi}\tilde{\bH}_{0,\subi}\Big(\frac{1}{T}\tilde{\bH}_{0,\subi}'\bF_{\gr{0},\subi}'\bF_{\gr{0},\subi}\tilde{\bH}_{0,\subi}\Big)^{-1}\tilde{\bH}_{0,\subi}'\bF_{\gr{0},\subi}'.
	%\end{split}
	$	
	By the results in part (ii),
	$\frac{1}{T}\|\widehat{\bF}_{\gr{0},\subi}-\bF_{\gr{0},\subi}\tilde{\bH}_{0,\subi}\|_F^2\lesssim_\P \delta_{KT}^{-2}+h_{K,\xi}^4$ uniformly over $i$.
	Since $\frac{1}{T}\widehat{\bF}_{\gr{0},\subi}'\widehat{\bF}_{\gr{0},\subi}=\bI_{\ttd_{\lambda,0}}$, the matrix in the bracket is also invertible w.p.a.1 and thus the above expression is well defined. Using the fact that for any two invertible matrix $\bA$ and $\bB$, $\bA^{-1}-\bB^{-1}=\bA^{-1}(\bB-\bA)\bB^{-1}$, we can see that
	$\|\bP_{\widehat{\bF}_{\gr{0},\subi}}-\bP_{\bF_{\gr{0},\subi}}\|_F^2\lesssim_\P \delta_{KT}^{-2}+h_{K,\xi}^4$
	uniformly over $i$.
	
	\iffalse
	\[
	\begin{split}
	\|\bP_{\widehat{\bF}_{1:\ttd_{\lambda,1},\subi}}-\bP_{\bF_{1:\ttd_{\lambda,1},\subi}}\|_F^2
	&=
	\Big\|\frac{1}{T_0}\widehat{\bF}_{1:\ttd_{\lambda,1},\subi}\widehat{\bF}_{1:\ttd_{\lambda,1},\subi}'-
	\frac{1}{T_0}\bF_{1:\ttd_{\lambda,1},\subi}\Big(\frac{1}{T_0}\bF_{1:\ttd_{\lambda,1},\subi}\bF_{1:\ttd_{\lambda,1},\subi}'\Big)^{-1}\bF_{1:\ttd_{\lambda,1},\subi}'\Big\|_F^2\\
	&=2\tr\Big(\bI_{\ttd_{\lambda,1}}-\widehat{\bF}_{1:\ttd_{\lambda,1},\subi}'\bP_{\bF_{1:\ttd_{\lambda,1},\subi}}\widehat{\bF}_{1:\ttd_{\lambda,1},\subi}/T_0\Big).
	\end{split}
	\]
	
	Now, note that
	\[
	\begin{split}
	%\frac{1}{T_0}\widehat{\bF}_{1:\ttd_{z,1},\subi}'\bP_{\bF_{1:\ttd_{\lambda,1},\subi}}\widehat{\bF}_{1:\ttd_{\lambda,1},\subi}=
	&\Big(\frac{1}{T_0}\widehat{\bF}_{1:\ttd_{\lambda,1},\subi}'\bF_{1:\ttd_{\lambda,1},\subi}\Big)\Big(\frac{1}{T_0}\bF_{1:\ttd_{\lambda,1},\subi}'\bF_{1:\ttd_{\lambda,1},\subi}\Big)^{-1}\Big(\frac{1}{T_0}\bF_{1:\ttd_{\lambda,1},\subi}'\widehat{\bF}_{1:\ttd_{\lambda,1},\subi}\Big)\\
	=\;&\Big(\frac{1}{T_0}\widehat{\bF}_{1:\ttd_{\lambda,1},\subi}'\Big(\bF_{1:\ttd_{\lambda,1},\subi}\tilde{\bH}_{1,\subi}-\widehat{\bF}_{1:\ttd_{\lambda,1},\subi}+\widehat{\bF}_{1:\ttd_{\lambda,1},\subi}\Big)\Big)\times\\
	&\Big(\frac{1}{T_0}\tilde{\bH}_{1,\subi}'\bF_{1:\ttd_{\lambda,1},\subi}'\bF_{1:\ttd_{\lambda,1},\subi}\tilde{\bH}_{1,\subi}\Big)^{-1}\times\\
	&\Big(\frac{1}{T_0}\Big(\bF_{1:\ttd_{\lambda,1},\subi}\tilde{\bH}_{1,\subi}-\widehat{\bF}_{1:\ttd_{\lambda,1},\subi}+\widehat{\bF}_{1:\ttd_{\lambda,1},\subi}\Big)'\widehat{\bF}_{1:\ttd_{\lambda,1},\subi}\Big).
	\end{split}
	\]
	
	By the same argument as in Lemma B.2 and B.3 of \cite{Bai_2003_ECMA},
	\fi
\end{proof}

\subsubsection*{Proof of Theorem \ref{thm: consistency eigenstructure}}
\begin{proof}
	The proof is divided into several steps.
	
	\textit{Step 1: second-order eigenvalues}.
	The analysis of $\bG_2$ in the proof of Lemma \ref{lem: eigenstructure 1st order} is the same (the projection operator  $\bM_{\widehat{\bF}_{\gr{0},\subi}}$ does not change the upper bound). Regarding $\bG_1$,
	\[
	\begin{split}
	\bG_1=&\bM_{\widehat{\bF}_{\gr{0},\subi}}\bF_{\subi}\bLambda_{\subi}'\bLambda_{\subi}\bF_{\subi}'\bM_{\widehat{\bF}_{\gr{0},\subi}}\\
	=&(\bM_{\widehat{\bF}_{\gr{0},\subi}}-\bM_{\bF_{\gr{0},\subi}})\bF_{\subi}\bLambda_{\subi}'\bLambda_{\subi}\bF_{\subi}'\bM_{\widehat{\bF}_{\gr{0},\subi}}
	+\\
	&\bM_{\bF_{\gr{0},\subi}}\bF_{\subi}\bLambda_{\subi}'\bLambda_{\subi}\bF_{\subi}'(\bM_{\widehat{\bF}_{\gr{0},\subi}}-\bM_{\bF_{\gr{0},\subi}})+\\
	&\bM_{\bF_{\gr{0},\subi}}\bF_{\subi}\bLambda_{\subi}'\bLambda_{\subi}\bF_{\subi}'\bM_{\bF_{\gr{0},\subi}}
	=: \bG_{1,1}+\bG_{1,2}+\bG_{1,3}.
	\end{split}
	\]
	Note that the three terms are defined locally for each neighborhood $\mathcal{N}_i$ and this implicit dependence on $\subi$ is suppressed for simplicity. 
	By Assumption \ref{SA Assumption: LPCA}, it is immediate that $s_j(\frac{1}{TK}\bG_{1,3})\asymp_\P h_{K,\xi}^2$ for for all $1\leq i\leq n$ and $j=1, \ldots, \ttd_{\lambda,1}$. 
	Regarding $\bG_{1,2}$, since $\max_{1\leq i\leq n}\frac{1}{\sqrt{TK}}\|\bM_{\bF_{\gr{0},\subi}}\bF_{\subi}\bLambda_{\subi}'\|_2\lesssim_\P h_{K,\xi}$, using
	part (iii) of Lemma \ref{lem: eigenstructure 1st order}, 
	$\|\frac{1}{TK}\bG_{1,2}\|_2\lesssim_\P
	(\delta_{KT}^{-1}+h_{K,\xi}^2)h_{K,\xi}$ uniformly over $i$.
	For $\bG_{1,1}$, further decompose the projection matrix on the far right: $\bM_{\widehat{\bF}_{\gr{0},\subi}}=\bM_{\widehat{\bF}_{\gr{0},\subi}}-\bM_{\bF_{\gr{0},\subi}}+\bM_{\bF_{\gr{0},\subi}}$. By similar calculation, it can be shown that 
	$\|\frac{1}{TK}\bG_{1,1}\|_2\lesssim_\P
	(\delta_{KT}^{-1}+h_{K,\xi}^2)^2+(\delta_{KT}^{-1}+h_{K,\xi}^2)h_{K,\xi}$ uniformly over $i$.
	Therefore, $\bG_{1,1}$ is dominated by $\bG_{1,3}$ due to the rate condition that $h_{K,\xi}\delta_{KT}\rightarrow\infty$.
	
	For $\bG_3$ or $\bG_4$, notice that 
	$
	%\begin{split}
	\frac{1}{TK}\bM_{\widehat{\bF}_{\gr{0},\subi}}\bF_{\subi}\bLambda_{\subi}'\bveps_{\subi}'\bM_{\widehat{\bF}_{\gr{0},\subi}}
	=\frac{1}{TK}\bM_{\bF_{\gr{0},\subi}}\bF_{\subi}\bLambda_{\subi}'\bveps_{\subi}'\bM_{\widehat{\bF}_{\gr{0},\subi}}\\
	+\frac{1}{TK}(\bM_{\widehat{\bF}_{\gr{0},\subi}}-\bM_{\bF_{\gr{0},\subi}})\bF_{\subi}\bLambda_{\subi}'\bveps_{\subi}'\bM_{\widehat{\bF}_{\gr{0},\subi}}.
	%\end{split}
	$
	By the same truncation argument used before, the first term is $O_\P(\sqrt{\log (n\vee T)}h_{K,\xi}K^{-1/2})$ uniformly over $i$, and the second one is $O_\P((\delta_{KT}^{-1}+h_{K,\xi}^2) K^{-1/2}\sqrt{\log (n\vee T)})$. Then, the result for the second-order eigenvalues follows.
	
	\textit{Step 2: Second-order eigenvectors}. 
	The proof is similar to that of Lemma \ref{lem: eigenstructure 1st order}, but I need to rewrite the identity \eqref{eq: decomposition}:
	\begin{align*}
	&\bM_{\widehat{\bF}_{\gr{0},\subi}}\widehat{\bF}_{\gr{1},\subi}-\bM_{\widehat{\bF}_{\gr{0},\subi}}\bF_{\subi}\tilde{\bH}_{\gr{1},\subi}\\
	=\bigg\{&\frac{1}{TK}\bM_{\widehat{\bF}_{\gr{0},\subi}}\bF_{\subi}\bLambda_{\subi}'\bveps_{\subi}'\widehat{\bF}_{\gr{1},\subi}+
	\frac{1}{TK}\bM_{\widehat{\bF}_{\gr{0},\subi}}\bveps_{\subi}\bLambda_{\subi}\bF_{\subi}' \bM_{\widehat{\bF}_{\gr{0},\subi}}\widehat{\bF}_{\gr{1},\subi}+\nonumber\\
	&\frac{1}{TK}\bM_{\widehat{\bF}_{\gr{0},\subi}}\bF_{\subi}\bLambda_{\subi}'\br_{\subi}'\widehat{\bF}_{\gr{1},\subi}+
	\frac{1}{TK}\bM_{\widehat{\bF}_{\gr{0},\subi}}\br_{\subi}\bLambda_{\subi}\bF_{\subi}'\bM_{\widehat{\bF}_{\gr{0},\subi}}\widehat{\bF}_{\gr{1},\subi}+\nonumber\\
	&\frac{1}{TK}\bM_{\widehat{\bF}_{\gr{0},\subi}}\br_{\subi}\bveps_{\subi}'\widehat{\bF}_{\gr{1},\subi}+
	\frac{1}{TK}\bM_{\widehat{\bF}_{\gr{0},\subi}}\bveps_{\subi}\br_{\subi}'\widehat{\bF}_{\gr{1},\subi}+\nonumber\\
	&\frac{1}{TK}\bM_{\widehat{\bF}_{\gr{0},\subi}}\br_{\subi}\br_{\subi}'\widehat{\bF}_{\gr{1},\subi}+
	\frac{1}{TK}\bM_{\widehat{\bF}_{\gr{0},\subi}}\bveps_{\subi}\bveps_{\subi}'\widehat{\bF}_{\gr{1},\subi}
	\bigg\}\times \widehat{\bV}_{\mathcal{C}_1\mathcal{C}_1,\subi}^{-1},
	\end{align*}
	where $\widehat{\bV}_{\mathcal{C}_1\mathcal{C}_1,\subi}$ is a diagonal matrix that contains the next $\ttd_{\lambda,1}$ leading eigenvalues of $\frac{1}{TK}\bA_{\subi}\bA_{\subi}'$.
	Note that in part (iii) of Lemma \ref{lem: eigenstructure 1st order}, 
	$\max_{1\leq i\leq n}\|\bM_{\widehat{\bF}_{\gr{0},\subi}}-\bM_{\bF_{\gr{0},\subi}}\|_F\lesssim_\P\delta_{KT}^{-1}+h_{K,\xi}^{2}$.
	Repeating the argument in Step 1 and Lemma \ref{lem: eigenstructure 1st order}, I have
	$\max_{1\leq i\leq n}\frac{1}{\sqrt{T}}\|\bM_{\widehat{\bF}_{\gr{0},\subi}}\widehat{\bF}_{\gr{1},\subi}-\bM_{\bF_{\gr{0}, \subi}\tilde{\bH}_{\gr{0},\subi}}\bF_{\subi}\tilde{\bH}_{\gr{1},\subi}\|_F\lesssim_\P \delta_{KT}^{-1}h_{K,\xi}^{-1}+h_{K,\xi}^{2m-2}$.
	Thus, the result for second-order eigenvectors follows.
	
	\textit{Step 3: Extension to higher-order terms}.
	The above calculation can be applied to even higher-order approximation as long as the rate condition $\delta_{KT}^{-1}h_{K,\xi}^{-(m-1)}=o(1)$ is satisfied. For instance, consider the third-order approximation.	
	Define $\bar{\mathcal{C}}_1=\mathcal{C}_0\cap\mathcal{C}_1$.
	To mimic the strategy before, the key is to analyze
	$
	\bM_{\widehat{\bF}_{\cdot\bar{\mathcal{C}}_1,\subi}}\bM_{\widehat{\bF}_{\gr{0},\subi}}\bF_{\cdot\bar{\mathcal{C}}_1,\subi}\bLambda_{\cdot\bar{\mathcal{C}}_1,\subi}'=
	\bM_{\widehat{\bF}_{\cdot\bar{\mathcal{C}}_1,\subi}}\bM_{\widehat{\bF}_{\gr{0},\subi}}\bF_{\gr{0},\subi}\bLambda_{\gr{0},\subi}'+
	\bM_{\widehat{\bF}_{\cdot\bar{\mathcal{C}}_1,\subi}}\bM_{\widehat{\bF}_{\gr{0},\subi}}\bF_{\gr{1}\subi}\bLambda_{\gr{1},\subi}'
	=:I_1+I_2.
	$
	By a similar argument used in the previous step, $\frac{1}{\sqrt{TK}}\|I_2\|_2=o_\P(h_{K,\xi}^2)$ uniformly over $i$. 
	
	Also,  
	$
	%\begin{split}
	-I_1=\bM_{\widehat{\bF}_{\cdot\bar{\mathcal{C}}_1,\subi}}(\bP_{\widehat{\bF}_{\gr{0},\subi}}-\bP_{\bF_{\gr{0},\subi}})\bF_{\gr{0},\subi}\bLambda_{\gr{0},\subi}'
	=\bM_{\widehat{\bF}_{\cdot\bar{\mathcal{C}}_1,\subi}}(
	\frac{1}{T}(\widehat{\bF}_{\gr{0},\subi}-\bF_{\gr{0},\subi}\tilde{\bH}_{0,\subi})\times\widehat{\bF}_{\gr{0},\subi}'+
	\quad\frac{1}{T}\bF_{\gr{0},\subi}\tilde{\bH}_{0,\subi}(\widehat{\bF}_{\gr{0},\subi}'-(\frac{1}{T}\tilde{\bH}_{0,\subi}'\bF_{\gr{0}, \subi}'\bF_{\gr{0}, \subi}\tilde{\bH}_{0,\subi})^{-1}\bF_{\gr{0}, \subi}'))\bF_{\gr{0},\subi}\bLambda_{\gr{0},\subi}'.
	%\end{split}
	$
	By the rate condition and the results in part (iii) of Lemma \ref{lem: eigenstructure 1st order} and step 2 of this proof, the second term divided by $\sqrt{TK}$ is $o_\P(h_{K,\xi}^2)$ uniformly over $i$ in terms of $\|\cdot\|_2$-norm.
	For the first term in the expression for $-I_1$, plug in the expansion for $\widehat{\bF}_{\gr{0},\subi}-\bF_{\gr{0}, \subi}\tilde{\bH}_{i,0}$. By consistency of $\bM_{\widehat{\bF}_{\cdot\bar{\mathcal{C}}_1,\subi}}$, 
	$
	\max_{1\leq i\leq n}\|\frac{1}{T^2K}
	\bM_{\widehat{\bF}_{\cdot\bar{\mathcal{C}}_1,\subi}}
	\bF_{\gr{1},\subi}\bLambda_{\gr{1},\subi}'\bLambda_{\gr{1},\subi}\bF_{\gr{1},\subi}\widehat{\bF}_{\gr{0},\subi}\widehat{\bF}_{\gr{0},\subi}'
	\|_2=o_\P(h_{K,\xi}^2)
	$.
	Other terms in the expansion are at most $O_\P(\delta_{KT}^{-1})=o_\P(h_{K,\xi}^2)$ uniformly over $i$ in terms of $\|\cdot\|_2$-norm. Then, we have $\max_{1\leq i\leq n}\|\frac{1}{\sqrt{TK}}\bM_{\widehat{\bF}_{\cdot\bar{\mathcal{C}}_1,\subi}}\bM_{\widehat{\bF}_{\gr{0},\subi}}\bF_{\cdot\bar{\mathcal{C}}_1,\subi}\bLambda_{\cdot\bar{\mathcal{C}}_1,\subi}'\|_2=o_\P(h_{K,\xi}^2)$.
	With this preparation, the remainder of the proof for higher-order approximations is the same as that used before.
	
	Finally, a typical $j$th column of the re-defined rotation matrix $\check{\bH}_{\subi}$ is given by 
	$\check{\bH}_{\cdot j, \subi}=
	\tilde{\bH}_{\cdot j, \subi}-\tilde{\bH}_{1:(j-1), \subi}(\tilde{\bH}_{1:(j-1), \subi}\bF_{\subi}'\bF_{\subi}\tilde{\bH}_{1:(j-1), \subi})^{-1}\tilde{\bH}_{1:(j-1), \subi}\bF_{\subi}'\bF_{\subi}\tilde{\bH}_{\cdot j,\subi}$.
	where $\tilde{\bH}_{1:(j-1), \subi}$ is the leading $(j-1)$ columns of $\tilde{\bH}_{\subi}$. Therefore,
	$\bF_{\subi}\check{\bH}_{\subi}$ is a columnwise orthogonalized version of $\bF_{\subi}\tilde{\bH}_{\subi}$.
\end{proof}

\subsubsection*{Proof of Lemma \ref{lem: eigenvector bound}}
\begin{proof}
	Throughout the proof, for a matrix $\bM$, $\|\bM\|_{2\rightarrow\infty}=\max_{i}\|\bM_{i\cdot}\|_2$. 
	I will mimic the proof strategy in \cite{Abbe-et-al_2020_AoS} and exploit a symmetric dilation trick.  Specifically, 
	Define 
	\[
	\bG=\left[\begin{array}{cc}
	\bm{0}&\bA_{\subi}\\
	\bA_{\subi}'&\bm{0}	
	\end{array}
	\right]
	\quad \text{and}\quad
	\bG^*=\left[\begin{array}{cc}
	\bm{0}&\bF_{\subi}\bLambda_{\subi}'\\
	\bLambda_{\subi}\bF_{\subi}'&\bm{0}
	\end{array}\right].
	\]
	I suppress the dependence of $\bG$ and $\bG^*$ on $\subi$ for simplicity. 
	By construction, the eigenvalue decomposition of $\bG$ will be
	\begin{scriptsize}
		\[
		\bG=\frac{\sqrt{KT}}{\sqrt{2}}\left[\begin{array}{cc}
		\frac{1}{\sqrt{T}}\widehat{\bF}_{\subi} & \frac{1}{\sqrt{T}}\widehat{\bF}_{\subi}\\
		\frac{1}{\sqrt{K}}\widehat{\bLambda}_{\subi}\widehat{\bV}_{\subi}^{-1/2} & 
		-\frac{1}{\sqrt{K}}\widehat{\bLambda}_{\subi}\widehat{\bV}_{\subi}^{-1/2}
		\end{array}\right]
		\times
		\left[\begin{array}{cc}
		\widehat{\bV}_{\subi}^{1/2}&\bm{0}\\
		\bm{0}&-\widehat{\bV}_{\subi}^{1/2}
		\end{array}\right]
		\times
		\frac{1}{\sqrt{2}}\left[\begin{array}{cc}
		\frac{1}{\sqrt{T}}\widehat{\bF}_{\subi} & \frac{1}{\sqrt{T}}\widehat{\bF}_{\subi}\\
		\frac{1}{\sqrt{K}}\widehat{\bLambda}_{\subi}\widehat{\bV}_{\subi}^{-1/2} & -\frac{1}{\sqrt{K}}\widehat{\bLambda}_{\subi}\widehat{\bV}_{\subi}^{-1/2}
		\end{array}\right]'.
		\]
	\end{scriptsize}
	\vspace{-1.5em}
	
	Now, for any $0\leq \ell\leq m-1$, let 
	\[
	\bar{\bU}=
	\left[
	\begin{array}{c}
	\bar{\bU}_{\mathtt{L}}\\
	\bar{\bU}_{\mathtt{R}}
	\end{array}\right]
	=\frac{1}{\sqrt{2}}\left[\begin{array}{c}
	\frac{1}{\sqrt{T}}\widehat{\bF}_{\gr{\ell},\subi}\\
	\frac{1}{\sqrt{K}}\widehat{\bLambda}_{\gr{\ell},\subi}\widehat{\bV}_{\mathcal{C}_\ell\mathcal{C}_\ell,\subi}^{-1/2}
	\end{array}\right]
	\quad\text{and}\quad
	\bar{\bSigma}=\sqrt{TK}\widehat{\bV}_{\mathcal{C}_\ell\mathcal{C}_\ell,\subi}^{1/2}.
	\]
	Clearly, they are the eigenvectors and eigenvalues of $\bG$ corresponding to the $\ell$th-order approximation.
	Define $\bar{\bU}^*$ and $\bar{\bSigma}^*$ for $\bG^*$ the same way.
	Define an eigengap for this eigenspace:
	$\Delta^*:=\sqrt{TK}((v_{\ttd_{\lambda,\ell-1},\subi}-v_{\ttd_{\lambda,\ell-1}+1,\subi})\wedge
	(v_{\ttd_{\lambda,\ell},\subi}-v_{\ttd_{\lambda,\ell}+1,\subi})\wedge\min_{s\in\mathcal{C}_\ell}|v_{s,\subi}|)$. 
	Similarly, $\Delta:=\sqrt{TK}((\widehat{v}_{\ttd_{\lambda,\ell-1},\subi}-\widehat{v}_{\ttd_{\lambda,\ell-1}+1,\subi})\wedge
	(\widehat{v}_{\ttd_{\lambda,\ell},\subi}-\widehat{v}_{\ttd_{\lambda,\ell}+1,\subi})\wedge\min_{s\in\mathcal{C}_\ell}|\widehat{v}_{s,\subi}|)$.
	Note that for ease of notation I suppress the dependence of these quantities on $\ell$.
			
	First consider any $1\leq t\leq T$.
	By Lemma 1 of \cite{Abbe-et-al_2020_AoS},
	\begin{equation}\label{SA-eq: lemma eigen bound}
	\|(\bar{\bU}\bar{\bH})_{t\cdot}\|_2\lesssim_\P \frac{1}{\sqrt{KT}h^{\ell}}\Big(\|\bG_{t\cdot}\bar{\bU}^*\|_2+\|\bG_{t\cdot}(\bar{\bU}\bar{\bH}-\bar{\bU}^*)\|_2\Big),
	\end{equation}
	since $\max_{1\leq i\leq n}\|\br_{\subi}+\bveps_{\subi}\|_2/\Delta^*=o_\P(1)$ and the eigengap $\Delta^*$ is $O_\P((KT)^{1/2}h^{\ell})$ uniformly over $i$ by Assumption \ref{SA Assumption: LPCA} and Lemma \ref{lem: operator norm of eps}.
	Regarding the first term on the right,
	\[
	\bG_{t\cdot}\bar{\bU}^*=\bar{\bU}_{t\cdot,\mathtt{L}}^*\bSigma^*+
	(\br_{t\cdot,\subi}+\bveps_{t\cdot,\subi})\bar{\bU}_{\mathtt{R}}^*
	\lesssim_\P
	\|\bar{\bSigma}^*\|_2\|\bar{\bU}^*_{t\cdot, \mathtt{L}}\|_2
	+h_{K,\xi}^m\sqrt{K}+
	\|\bveps_{t\cdot,\subi}\bar{\bU}_{\mathtt{R}}^*\|_2.
	\]
	Since $\bar{\bU}_{\mathtt{R}}^*$ is uncorrelated with $\bveps_{t\cdot,\subi}$, the last term is a zero-mean sequence. Apply the truncation argument again. Specifically, let $\mathcal{M}_n$ be the $\sigma$-field generated by $\bar{\bU}_{\mathtt{R}}^*$, and 
	define $\zeta_{tk,\subi}^-=\varepsilon_{tk,\subi}\bar{U}^*_{kj,\mathtt{R}}\I(|\varepsilon_{tk,\subi}|\leq\tau_n)-\E[\varepsilon_{tk,\subi}\bar{U}^*_{kj,\mathtt{R}}\I(|\varepsilon_{tk,\subi}|\leq\tau_n)|\mathcal{M}_n]$ and $\zeta_{tk,\subi}^+=\varepsilon_{tk,\subi}\bar{U}^*_{kj,\mathtt{R}}-\zeta_{tk,\subi}^-$ for $\tau_n\asymp \sqrt{K/\log (n\vee T)}$. By Bernstein inequality, for any $\delta>0$,
	\[
	\P\Big(\Big|\sum_{k=1}^{K}\zeta_{tk,\subi}^-\Big|\geq\delta\Big|\mathcal{M}_n\Big)\leq 2\exp\Big(-\frac{\delta^2/2}{C\|\bar{\bU}^*_{\mathtt{R}}\|^2_2+\|\bar{\bU}^*_{\mathtt{R}}\|_{2\rightarrow\infty}\tau_n\delta/3}\Big),
	\]
	for some constant $C>0$.
	On the other hand,
	\[
	\P\Big(\max_{1\leq i\leq n}\max_{t\in\mathcal{T}_2}\Big|\sum_{k=1}^{K}\zeta_{tk,\subi}^+\Big|\geq\delta\Big|\mathcal{M}_n\Big)\leq nT\delta^{-2}\tau_n^{-\nu}\|\bar{\bU}_{\mathtt{R}}^*\|^2_2.
	\]
	The above suffices to show $\|\bveps_{t\cdot,\subi}\bar{\bU}_{\mathtt{R}}^*\|_2\lesssim_\P
	\sqrt{\log (T\vee n)}(1\vee\sqrt{K}\|\bar{\bU}_{\mathtt{R}}^*\|_{2\rightarrow\infty})$ uniformly over $1\leq t\leq T$ and $1\leq i\leq n$. 
	
	Now, I analyze the second term by using a ``leave-one-out'' trick.
	Specifically,
	for each $1\leq t\leq T$, let $\bar{\bU}^{(t)}$ be the eigenvector of $\bG^{(t)}$ where a generic $(s,i)$th entry of $\bG_{\subi}^{(t)}$ is given by
	$G_{si}^{(t)}=G_{si}\I(s,i\neq t)$. 
	Due to the possibility of equal eigenvalues, introduce a rotation matrix $\bar{\bH}$ and $\bar{\bH}^{(t)}$ as defined in \cite{Abbe-et-al_2020_AoS}:
	$\bar{\bH}=\bar{\bU}'\bar{\bU}^*$ and $\bar{\bH}^{(t)}=(\bar{\bU}^{(t)})'\bar{\bU}^*$.
	Then, I can write
	\[
	\bG_{t\cdot}(\bar{\bU}\bar{\bH}-\bar{\bU}^*)=
	\bG_{t\cdot}(\bar{\bU}\bar{\bH}-\bar{\bU}^{(t)}\bar{\bH}^{(t)})+
	\bG_{t\cdot}(\bar{\bU}^{(t)}\bar{\bH}^{(t)}-\bar{\bU}^*)=:I+II,
	\]
	
	For $I$, by Lemma 3 of \cite{Abbe-et-al_2020_AoS}, $\|\bar{\bU}\bar{\bH}-\bar{\bU}^{(t)}\bar{\bH}^{(t)}\|_2
	\leq\|\bar{\bU}\bar{\bU}'-\bar{\bU}^{(t)}(\bar{\bU}^{(t)})'\|_2\lesssim_\P \|(\bar{\bU}\bar{\bH})_{t\cdot}\|_2$ 
	since by Theorem \ref{thm: consistency eigenstructure}, 
	$\Delta\geq\kappa\Delta^*$ for some $\kappa>0$ with probability approaching one and $\|\bG\|_{2\rightarrow\infty}=o_\P(\Delta^*)$ uniformly over $i$. Therefore,
	$\|\bG_{t\cdot}(\bar{\bU}\bar{\bH}-\bar{\bU}^{(t)}\bar{\bH}^{(t)})\|_2\lesssim \|\bG_{t\cdot}\|_2\|(\bar{\bU}\bar{\bH})_{t\cdot}\|_2\lesssim_\P\sqrt{K}\|(\bar{\bU}\bar{\bH})_{t\cdot}\|_2$ uniformly over $i$.
	
	For $II$, again, by Bernstein inequality and the truncation argument, 
	$$\|\bveps_{t\cdot, \subi}(\bar{\bU}_{\mathtt{R}}^{(t)}\bar{\bH}^{(t)}-\bar{\bU}_{\mathtt{R}}^*)\|_2\lesssim_\P
	\sqrt{\log (T\vee n)}
	(1\vee\sqrt{K}\|(\bar{\bU}_{\mathtt{R}}^{(t)}\bar{\bH}^{(t)}-\bar{\bU}_{\mathtt{R}}^*)\|_{2\rightarrow\infty})$$
	uniformly over $t$ and $i$ by the leave-one-out   construction. 
	By Equation B.13 in Lemma 3 of \cite{Abbe-et-al_2020_AoS}, $\|\bar{\bU}_{\mathtt{R}}^{(t)}\bar{\bH}^{(t)}-\bar{\bU}_{\mathtt{R}}^*\|_{2\rightarrow\infty}\lesssim_\P\|\bar{\bU}_{\mathtt{L}}\bar{\bH}\|_{2\rightarrow\infty}+ \|\bar{\bU}_{\mathtt{R}}\bar{\bH}\|_{2\rightarrow\infty}+\|\bar{\bU}_{\mathtt{R}}^*\|_{2\rightarrow\infty}$.
	Then,
	it remains to bound $\bG^*_{t\cdot}(\bar{\bU}_{\mathtt{R}}^{(t)}\bar{\bH}^{(t)}-\bar{\bU}_{\mathtt{R}}^*)$.
	Recall that by definition of singular vectors, $\bar{\bU}_{\mathtt
	R}$ and $\bar{\bU}_{\mathtt{R}}^*$ are orthogonal to other leading right singular vectors. Thus, I can insert projection matrices $\bM_{\bar{\bU}_{1:(\ell-1),\mathtt{R}}}$ and $\bM_{\bar{\bU}^*_{1:(\ell-1), \mathtt{R}}}$ as follows:
	\[
	\begin{split}
	\bG^*_{t\cdot}(\bar{\bU}_{\mathtt{R}}^{(t)}\bar{\bH}^{(t)}-\bar{\bU}_{\mathtt{R}}^*)
	&=\bG^*_{t\cdot}\bM_{\bar{\bU}^{(t)}_{1:(\ell-1),\mathtt{R}}}\bar{\bU}_{\mathtt{R}}^{(t)}\bar{\bH}^{(t)}-\bG_{t\cdot}^*\bM_{\bar{\bU}^*_{1:(\ell-1),\mathtt{R}}}\bar{\bU}_{\mathtt{R}}^*\\
	&=\bG^*_{t\cdot}(\bM_{\bar{\bU}^{(t)}_{1:(\ell-1),\mathtt{R}}}-\bM_{\Lambda_{1:(\ell-1)}})\bar{\bU}_{\mathtt{R}}^{(t)}\bar{\bH}^{(t)}-
	\bG_{t\cdot}^*(\bM_{\bar{\bU}^*_{1:(\ell-1),\mathtt{R}}}-\bM_{\Lambda_{1:(\ell-1)}})\bar{\bU}_{\mathtt{R}}^*\\
	&\quad+\bG^*_{t\cdot}\bM_{\Lambda_{1:(\ell-1)}}(\bar{\bU}_{\mathtt{R}}^{(t)}\bar{\bH}^{(t)}-\bar{\bU}_{\mathtt{R}}^*).
	\end{split}
	\]
	``$1:(\ell-1)$'' in subscripts denote the leading $\ell-1$ columns of the corresponding matrices.
	By the same argument in the proof of Theorem \ref{thm: consistency eigenstructure},
	$\|\bG^*_{t\cdot}(\bar{\bU}_{\mathtt{R}}^{(t)}\bar{\bH}^{(t)}-\bar{\bU}_{\mathtt{R}}^*)\|_2\lesssim_\P \sqrt{K}h_{K,\xi}^{\ell}$.
	Moreover, note 
	$s_{\min}(\bar{\bSigma}^*\bar{\bU}_{\mathtt{R}}^*)
	\|\bar{\bU}^*_{\mathtt{L}}\|_{2\rightarrow\infty}
	\lesssim\|\bar{\bU}_{\mathtt{L}}^*\bar{\bSigma}^*\bar{\bU}_{\mathtt{R}}^*\|_{2\rightarrow\infty}\leq
	\|\bM_{\bar{\bU}^*_{1:(\ell-1),\mathtt{L}}}\bF_{\subi}\bLambda_{\subi}'\bM_{\bar{\bU}^*_{1:(\ell-1),\mathtt{R}}}\|_{2\rightarrow\infty}\\
	\lesssim_\P h_{K,\xi}^\ell\sqrt{K}$, 
	where $s_{\min}(\bar{\bSigma}^*\bar{\bU}_{\mathtt{R}}^*)\gtrsim_\P\sqrt{TK}h_{K,\xi}^\ell$ by Assumption \ref{SA Assumption: LPCA}.
	Then, $\|\bar{\bU}_{\mathtt{L}}^*\|_{2\rightarrow\infty}\lesssim_\P T^{-1/2}$.
	Now, by plugging in all these bounds and rearranging the terms in Equation \eqref{SA-eq: lemma eigen bound}, we have
	$$\|\bar{\bU}_{\mathtt{L}}\bar{\bH}\|_{2\rightarrow\infty}\lesssim_\P
	%\|\bar{\bU}^*_{\mathtt{L}}\|_{2\rightarrow\infty}+
	\frac{1}{\sqrt{T}}+\frac{\sqrt{\log (n\vee T)}}{\sqrt{T}h^\ell}\|\bU_{\mathtt{R}}\bar{\bH}\|_{2\rightarrow\infty}$$
	uniformly over $\subi$.
	
	The analysis of $\bar{\bU}_{\mathtt{R}}$ is exactly the same by considering $T+1\leq t\leq T+n$, and we have the following bound (uniformly over $\subi$)
	$$\|\bar{\bU}_{\mathtt{R}}\bar{\bH}\|_{2\rightarrow\infty}\lesssim_\P
	%\|\bar{\bU}^*_{\mathtt{R}}\|_{2\rightarrow\infty}+
	\frac{1}{\sqrt{K}}+\frac{\sqrt{\log (n\vee T)}}{\sqrt{K}h^\ell}\|\bU_{\mathtt{L}}\bar{\bH}\|_{2\rightarrow\infty}.$$
    
    The desired sup-norm bound follows by combining the two inequalities.	
	
	\iffalse
	Finally, the same proof strategy can be applied to bound $\widehat{\bLambda}_{\subi}$ by considering $T+1\leq t\leq T+n$. Due to the row-wise demeaning of $\bA$, I need to slightly modify the previous construction so that the leave-one-out trick can be still applied. Note that we can define $\tilde{\bA}_{\subi}=\bF_{\subi}\bLambda_{\subi}'+\br_{\subi}+\bveps_{\subi}$, and by normalization $\dot{\bA}=\tilde{\bA}_{\subi}-\bveps_{\subi}\iota_K\iota_K'/K$. The same argument before can be directly applied to $\tilde{\bA}_{\subi}$ and the bound for its right singular vector can be established. Then, I only need to consider the perturbation resulting from the row-wise means of $\bveps_{ j_k(i)}\subi$. Let $\tilde{\bU}_{\mathtt{P}}$ denote the right singular vector of $\tilde{\bA}$. Then,
	\[
	\|\bar{\bU}_{\mathtt{R}}\bar{\bU}_{\mathtt{R}}'-
	\tilde{\bU}_{\mathtt{R}}\tilde{\bU}_{\mathtt{R}}'\|_2
	\lesssim\|(\tilde{\bA}'\tilde{\bA}-\dot{\bA}'\dot{\bA})\bar{\bU}_{\mathtt{R}}\|_2/\Delta^*=0
	\]
	\fi
\end{proof}

\subsubsection*{Proof of Theorem \ref{thm: uniform convergence of factors}}
\begin{proof}
	Expand the estimator of factor loadings:
	$\widehat{\bLambda}_{\subi}-\bLambda_{\subi}\bH_{\subi}
	=%\frac{1}{T}\bLambda_{\subi}(\bH_{\subi}')^{-1}
	%(\bF_{\subi}\bH_{\subi}-\widehat{\bF}_{\subi})'\widehat{\bF}_{\subi}+
	\frac{1}{T}\br_{\subi}'\widehat{\bF}_{\subi}+
	\frac{1}{T}\bveps_{\subi}'\widehat{\bF}_{\subi}=:I_1+I_2$ 
	for $\bH_{\subi}=\frac{1}{T}\bF_{\subi}'\widehat{\bF}_{\subi}$. 
	Regarding $I_1$,
	$
	\max_{1\leq i\leq n}\max_{1\leq k\leq K}
	\|\frac{1}{T}\sum_{t\in\mathcal{T}_2}
	\widehat{\bF}_{t,\subi}'r_{j_k(i),t}\|_2\lesssim_\P h_{K,\xi}^{m}$.
	
	For $I_2$, again, use the ``leave-one-out'' trick as in the proof of Lemma \ref{lem: eigenvector bound}. Specifically,
	For each $1\leq k\leq K$, let $T^{-1/2}\widehat{\bF}_{\subi}^{(k)}$ be the left singular vector of $\bA_{\subi}^{(k)}$, where a generic $(s,i)$th entry of $\bA_{\subi}^{(k)}$ is given by
	$a_{si,\subi}^{(k)}=a_{si,\subi}\I(i\neq k)$. 
	Due to the possibility of equal eigenvalues, introduce a rotation matrix $\bar{\bH}$ and $\bar{\bH}^{(k)}$ as in Section A.2 of \cite{Abbe-et-al_2020_AoS}.	
	Then, further decompose $I_2$ into
	\[
	I_2\times\bar{\bH}=%\frac{1}{T}\dot{\bveps}_{\subi}'\bF_{\subi}\bH_{\subi}^{(k)}+
	\frac{1}{T}\bveps_{\subi}'\widehat{\bF}_{\subi}^{(k)}\bar{\bH}^{(k)}
	+\frac{1}{T}\bveps_{\subi}'(\widehat{\bF}_{\subi}\bar{\bH}-\widehat{\bF}_{\subi}^{(k)}\bar{\bH}^{(k)}).
	\]
    %Notice that, due to the weak correlation condition and the moment condition, the first term is bounded by $\sqrt{\log N/T}$ uniformly over $1\leq k\leq K$.
    
    By construction, $\bveps_{k\cdot,\subi}$ and $\widehat{\bF}_{\subi}^{(k)}$ are independent. Let $\mathcal{M}_n$ be the $\sigma$-field generated by $\widehat{\bF}_{\subi}^{(k)}$. By the leave-one-out construction,
    $\E[\varepsilon_{ks}\widehat{\bff}_{s,\subi}^{(k)}|\mathcal{M}_n]=0$ and 
    $\V[T^{-1/2}\sum_{s\in\mathcal{T}}\varepsilon_{ks}\widehat{\bff}_{s,\subi}^{(k)}|\mathcal{M}_n]\lesssim_\P 1$. Then, by Lemma \ref{lem: eigenvector bound}, $\|\widehat{\bff}_{s,\subi}\|_{\max}\lesssim_\P 1$, and then by a similar argument as given in the proof of Lemma \ref{thm: IMD hom}, the first term is $O_\P(\delta_{KT}^{-1})$ uniformly over $1\leq i\leq n$ and $1\leq k\leq K$.	
	
	Regarding the second term, for any $1\leq k\leq K$,
	$\|\frac{1}{\sqrt{T}}\bveps_{k\cdot,\subi}'
	(\frac{1}{\sqrt{T}}\widehat{\bF}_{\subi}\bar{\bH}-
	\frac{1}{\sqrt{T}}\widehat{\bF}_{\subi}^{(k)}\bar{\bH}^{(k)})\|_2\leq
	\frac{1}{\sqrt{T}}\|\bveps_{k\cdot,\subi}\|_2
	\|\bP_{\widehat{\bF}_{\subi}}-\bP_{\widehat{\bF}_{\subi}^{(k)}}\|_2$.
	Note $\max_{1\leq i\leq n}\max_{1\leq k\leq K} T^{-1/2}\|\bveps_{k\cdot,\subi}\|_2\lesssim_\P 1$.
	Moreover, by the result given in the proof of Lemma \ref{lem: eigenvector bound}, $\|\bP_{\widehat{\bF}_{\subi}}-\bP_{\widehat{\bF}_{\subi}^{(k)}}\|_2\lesssim\|\bar{\bU}_{k\cdot}\|_2\lesssim_\P\delta_{KT}^{-1}$ uniformly over $i$ and $k$.
	Then, the result for factor loadings follows.
	
	Now, consider the estimated factors:
	{\small
	\begin{equation}\label{SA-eq: decomp of factors}
	\widehat{\bF}_{\subi}\widehat{\bV}_{\subi}=
	\bF_{\subi}(\bH_{\subi}')^{-1}\widehat{\bV}_{\subi}+
	\frac{1}{K}\bF_{\subi}(\bH_{\subi}')^{-1}(\bLambda_{\subi}\bH_{\subi}-\widehat{\bLambda}_{\subi})'\widehat{\bLambda}_{\subi}+
	\frac{1}{K}\br_{\subi}\widehat{\bLambda}_{\subi}+
	\frac{1}{K}\bveps_{\subi}\widehat{\bLambda}_{\subi}.
	\end{equation}
	}
    \vspace{-1.2em}
   
	For the $\ell$th-order approximation (columns with indices in $\mathcal{C}_\ell$), by Lemma \ref{lem: eigenvector bound},
	the second term is $O_\P((\delta_{KT}^{-1}+h_{K,\xi}^m)h_{K,\xi}^{\ell})$ uniformly over $i$ and $t$; 
	the third term is $O_\P(h_{K,\xi}^{m+\ell})$ uniformly over $i$ and $t$;
	the fourth term is $O_\P((\delta_{KT}^{-1}+h_{K,\xi}^m)h_{K,\xi}^{\ell})$ by the same argument used before. Note that $\bH_{\subi}$ is invertible as explained in the proof of Lemma \ref{lem: eigenstructure 1st order}. Moreover,
	$
	\bH_{\subi}\bH_{\subi}'=\frac{1}{T^2}\bF_{\subi}'\widehat{\bF}_{\subi}
	\widehat{\bF}_{\subi}'\bF_{\subi}=\frac{1}{T}\bF_{\subi}'\bP_{\widehat{\bF}_{\subi}}\bF_{\subi}$.
	The eigenvalues of this matrix is bounded both from above and below in probability by Assumption \ref{SA Assumption: LPCA}(b) and the consistency of projection matrices due to Theorem \ref{thm: consistency eigenstructure}.
	Then, the proof is complete.

\end{proof}

\subsubsection*{Proof of Theorem \ref{thm: consistency of latent mean}}
\begin{proof}
	By construction of the estimator, 
	$\widehat{L}_{tk,\subi}-L_{tk,\subi}
	=\widehat{\bff}_{t,\subi}'\widehat{\blambda}_{j_k(i)}-\bff_{t,\subi}'\blambda_{j_k(i),\subi}-r_{tj_k(i)}
	\lesssim_\P h_{K,\xi}^m+
	(\widehat{\bff}_{t,\subi}'-\bff_{t,\subi}'(\bH_{\subi}')^{-1})\widehat{\blambda}_{j_k(i)}+
	\bff_{t,\subi}'(\bH_{\subi}')^{-1}(\widehat{\blambda}_{j_k(i)}-\bH_{\subi}'\blambda_{j_k(i)})$.
	By Theorem \ref{thm: uniform convergence of factors},
	$\widehat{\bff}_{t,\subi}-\bff_{t,\subi}(\bH_{\subi}')^{-1}\lesssim_\P
	(\delta_{KT}^{-1}+h_{K,\xi}^m)(\Upsilon_{11}^{-1},\cdots, \Upsilon_{jj}^{-1})'$, and 
	$\widehat{\blambda}_{j_k(i)}-\bH_{\subi}'\blambda_{j_k(i)}\lesssim_\P\delta_{KT}^{-1}+h_{K,\xi}^m$, which hold uniformly over $t, k$ and $i$. Then, the result follows.
\end{proof}

%%%%%%%%%%%%%%%%%%%%%%%%%%%%%%%%%%%%%%%%%%%%%%%%%%%%%%%%%%%
\subsection{Proofs for Section \ref{SA-sec: main results}}

\subsubsection*{Proof of Lemma \ref{SA-lem: slope of covariates}}
\begin{proof}
	Let $T_2=|\mathcal{T}_2|$. By assumption, I can rewrite the outcome equation as
	\[
	\begin{split}
	x_{it}=\sum_{\ell=1}^{\ttd_w}\hbar_{t,\ell}(\bvrho_{i,\ell})\vartheta_\ell+\sum_{\ell=1}^{\ttd_w}e_{it, \ell}\vartheta_\ell
	+\eta_t(\balpha_i)+u_{it}
	=\hslash_{t}(\bvrho_i)+
	\sum_{\ell=1}^{\ttd_w}e_{it,\ell}\vartheta_\ell+u_{it},
	\end{split}
	\]
	where $\hslash_{t}(\bvrho_{i})=
	\eta_t(\balpha_i)+\sum_{\ell=1}^{\ttd_w}\hbar_{t,\ell}(\bvrho_{i,\ell})
	\vartheta_\ell$ and $\bvrho_{i}$ is a vector collecting all distinct variables among $\balpha_i,\bvrho_{i,1},\cdots, \bvrho_{i,\ttd_w}$. Note that $\balpha_i$ is included in $\bvrho_i$ as a subvector. 
	
	I first prepare some notation. For each $t\in\mathcal{T}_2$, define  $\hslash_{it}:=\hslash_t(\bvrho_i)$ and stack them in a $T_2$-dimensional vector $\bm{\hslash}_{i}$. For each $\ell=1,\ldots, \ttd_w$, $\hbar_{it,\ell}:=\hbar_{t,\ell}(\bvrho_{i,\ell})$ with $t\in\mathcal{T}_2$, and stack them in $\bm{\hbar}_{i,\ell}$. Similarly, let $\be_{i,\ell}$ be a $T_2$-vector with typical elements $e_{it,\ell}$ for $t\in\mathcal{T}_2$ and $\be_i=(\be_{i,1}, \cdots, \be_{i,\ttd_w})'$. The estimators of $\bm{\hbar}_{i,\ell}$, $\bm{\hslash}_i$ and $\be_i$ are denoted by $\widehat{\bm{\hbar}}_{i,\ell}$, $\widehat{\bm{\hslash}}_i$ and $\widehat{\be}_i$.
	Write
	\[
	\begin{split}
	\widehat{\bvth}-\bvth=
	\Big(\frac{1}{nT_2}\sum_{i=1}^{n}\widehat{\be}_i\widehat{\be}_i'\Big)^{-1}
	\bigg\{&\Big(\frac{1}{nT_2}\sum_{i=1}^{n}
	\widehat{\be}_i\bu_i\Big)+
	\Big(\frac{1}{nT_2}\sum_{i=1}^{n}\widehat{\be}_i(\be_i-\widehat{\be}_i)'\bvth\Big)+\\
	&\Big(\frac{1}{nT_2}\sum_{i=1}^{n}\widehat{\be}_i(\bm{\hslash}_{i}-\widehat{\bm{\hslash}}_{i})\Big)\bigg\}
	=\Big(\frac{1}{nT_2}\sum_{i=1}^{n}\widehat{\be}_i\widehat{\be}_i'\Big)^{-1}\times(I_1+I_2+I_3).
	\end{split}
	\]
	
	Now, first notice that
	\[
	\frac{1}{nT_2}\sum_{i=1}^{n}\widehat{\be}_i\widehat{\be}_i'=
	\frac{1}{nT_2}\sum_{i=1}^{n}\be_i\be_i'+\frac{1}{nT_2}\sum_{i=1}^{n}(\widehat{\be}_i-\be_i)(\widehat{\be}_i-\be_i)'+\frac{1}{n}\sum_{i=1}^{n}(\widehat{\be}_i-\be_i)\be_i'+
	\frac{1}{n}\sum_{i=1}^{n}\be_i(\widehat{\be}_i-\be_i)'.
	\]
	By Assumption \ref{SA-Assumption: high-rank covariates}, the first term is bounded away from zero with probability approaching one.  
	Note that for each $1\leq\ell\leq \ttd_w$, $\widehat{\be}_{i,\ell}-\be_{i,\ell}=
	\bm{\hbar}_{i,\ell}-\widehat{\bm{\hbar}}_{i,\ell}$.
	Under Assumptions \ref{SA-Assumption: high-rank covariates} and \ref{SA-Assumption: latent structure}, the conditions of Theorem  \ref{thm: consistency of latent mean} are satisfied and hence 
	$\max_{1\leq i\leq n}
	\|\widehat{\bm{\hbar}}_i-\bm{\hbar}_i\|_{\max}=o_\P(1)$.
	Therefore, the last three terms are $o_\P(1)$.
	
	Next, consider $I_2$. For any $1\leq \ell, \ell'\leq \ttd_w$, by Theorem \ref{thm: consistency of latent mean},
		\[
		\begin{split}
		\frac{1}{nT_2}\sum_{i=1}^{n}\sum_{t\in\mathcal{T}_2}
		\widehat{e}_{it,\ell}(e_{it,\ell'}-&\widehat{e}_{it,\ell'})
		=\frac{1}{nT_2}\sum_{i=1}^{n}\sum_{t\in\mathcal{T}_2}
		e_{it,\ell}(\widehat{\hbar}_{it,\ell'}-\hbar_{it,\ell'})+\\
		&\frac{1}{nT_2}\sum_{i=1}^{n}\sum_{t\in\mathcal{T}_2}
		(\hbar_{it,\ell}-\widehat{\hbar}_{it,\ell})(\widehat{\hbar}_{it,\ell'}-\hbar_{it,\ell'})
		= I_{2,1}+O_\P(\delta_{KT}^{-2}+h_{K,\varrho}^{2m}).
		\end{split}
		\]
	For $I_{2,1}$, by construction, I can write the $\widehat{\hbar}_{it,\ell'}-\hbar_{it,\ell'}=
	%\bar{r}_{t,\ell',\subi}+\bar{e}_{t,\ell',\subi}+
	-r_{it,\ell',\subi}+
	\widehat{\bff}_{t,\subi}'\widehat{\blambda}_{i,\subi}-\bff_{t,\subi}'\blambda_{i,\subi}$. With slight abuse of notation, I use $\widehat{\bff}_{t,\subi}$ and $\widehat{\blambda}_{i,\subi}$ to denote the factors corresponding to time $t$ and factor loadings corresponding to unit $i$ extracted from $\bw_{i,\ell'}$. 
	It is easy to see that %$\bar{r}_{t,\ell',\subi}\lesssim_\P \delta_{KT}^{-1}h_{K,\varrho}^{m}$,
	$\frac{1}{nT_2}\sum_{i=1}^{n}\sum_{t\in\mathcal{T}_2}r_{it,\ell',\subi}e_{it,\ell}\lesssim_\P h_{K,\varrho}^{m}T^{-1/2}$. 
	%and $\frac{1}{nT_2}\sum_{t=1}^{T_2}\sum_{i=1}^{n}
	%\bar{e}_{t,\ell',\subi}e_{it,\ell}\lesssim_\P \delta_{KT}^{-2}$.
	Moreover,
	\[
	\begin{split}
	\frac{1}{nT_2}\sum_{i=1}^{n}\sum_{t\in\mathcal{T}_2}
	(\widehat{\bff}_{t,\subi}'\widehat{\blambda}_{i,\subi}-&\bff_{t,\subi}'\blambda_{i,\subi})e_{it,\ell}
	=\frac{1}{nT_2}\sum_{i=1}^{n}\sum_{t\in\mathcal{T}_2}
	(\widehat{\bff}_{t,\subi}'-\bff_{t,\subi}'(\bH_{\subi}')^{-1})\widehat{\blambda}_{i,\subi}e_{it,\ell}+\\
	&\frac{1}{nT_2}\sum_{i=1}^{n}\sum_{t\in\mathcal{T}_2}
	\bff_{t,\subi}'(\bH_{\subi}')^{-1}(\widehat{\blambda}_{i,\subi}-\bH_{\subi}'\blambda_{i,\subi})e_{it,\ell}
	=:I_{2,1,1}+I_{2,1,2}.
	\end{split}
	\]
	
	Regarding $I_{2,1,1}$, plug in the expansion of the estimated factors as in Equation \eqref{SA-eq: decomp of factors}:
	%By Theorem \ref{thm: uniform convergence of factors}, 
	\[
	\begin{split}
	&\frac{1}{T_2}\sum_{t\in\mathcal{T}_2}(\widehat{\bff}_{t,\subi}'-\bff_{t,\subi}'(\bH_{\subi}')^{-1})e_{it,\ell}\widehat{\blambda}_{i,\subi}
	=\Big\{\frac{1}{T_2K}\sum_{t\in\mathcal{T}_2}\sum_{k=1}^{K}e_{it,\ell}\bff_{t,\subi}'(\bH_{\subi}')^{-1}(\bH_{\subi}'\blambda_{j_k(i)}-\widehat{\blambda}_{j_k(i)})\widehat{\blambda}_{j_k(i)}'\\
	&\hspace{6em}+\frac{1}{T_2K}\sum_{t\in\mathcal{T}_2}\sum_{k=1}^{K}e_{it,\ell}e_{j_k(i)t,\ell}\widehat{\blambda}_{j_k(i)}'+
	\frac{1}{T_2K}\sum_{t\in\mathcal{T}_2}\sum_{k=1}^{K}e_{it,\ell}r_{j_k(i)t}\widehat{\blambda}_{j_k(i)}'\Big\}\times\widehat{\bV}_{\subi}^{-1}\widehat{\blambda}_{i,\subi}.
	\end{split}
	\]
	By the argument in the proof of Theorem \ref{thm: uniform convergence of factors}, $\frac{1}{T_2K}\sum_{t\in\mathcal{T}_2}\sum_{k=1}^{K}e_{it,\ell}e_{j_k(i)t,\ell}\widehat{\blambda}_{j_k(i)}'\widehat{\bV}_{\subi}^{-1/2}\lesssim_\P\delta_{KT}^{-1}$. 
	By Assumption \ref{SA-Assumption: high-rank covariates} and \ref{SA-Assumption: latent structure}, $\frac{1}{T_2}\sum_{t\in\mathcal{T}_2}e_{it,\ell}r_{j_k(i)t}\lesssim_\P h_{K,\varrho}^{m}\delta_{KT}^{-1}$ uniformly over $k$ and $i$. By Theorem \ref{thm: uniform convergence of factors} and the fact that  
	$\frac{1}{T_2}\sum_{t\in\mathcal{T}_2}\bff_{t,\subi}'e_{it,\ell}
	\lesssim_\P \delta_{KT}^{-1}$ uniformly over $k$ and $i$, the first term in $I_{2,1,1}$ is of smaller order.
	Then, it follows that $I_{2,1,1}=O_\P(\delta_{KT}^{-1}+h_{K,\varrho}^{m}\delta_{KT}^{-1})$. 
	Moreover, by Theorem \ref{thm: uniform convergence of factors}, 
	$I_{2,1,2}=O_\P(\delta_{KT}^{-1}(\delta_{KT}^{-1}+h_{K,\varrho}^{m}))$.
	$I_3$ can be treated similarly. 
	
	Finally, for $I_1$,
	$\frac{1}{nT_2}\sum_{i=1}^{n}
	\widehat{\be}_i\bu_i=
	\frac{1}{nT_2}\sum_{i=1}^{n}
	\be_i\bu_i+\frac{1}{nT_2}\sum_{i=1}^{n}
	(\widehat{\be}_i-\be_i)\bu_i$. 
	Note that $\E[\bu_i|\bw_i]=0$ and $\E[\bu_i|\mathcal{F}]=0$ imply that $\bu_i$ is uncorrelated with $\be_i$.  
	Then, by Assumption \ref{SA-Assumption: latent structure}, the first term is $O_\P(1/\sqrt{nT})$. The second term is mean zero and of smaller order due to the consistency of $\widehat{\be}_i$. Then, the proof is complete.
\end{proof}

\subsubsection*{Proof of Theorem \ref{SA-thm: relevant FE}}
\begin{proof}
	By construction, I use the subsample $\mathcal{T}_1$ for initial matching on $\bx_i$'s and $\bw_i$'s, and then apply local PCA to the subsample $\mathcal{T}_2$ to obtain  $\widehat{\bvth}$. Consider the following steps.
	
	\textit{Step 1: Matching.} Apply the matching procedure to $\bA_i:=\bx_i-\bW_i\widehat{\bvth}$  on $\mathcal{T}_2$. Let $T_2=|\mathcal{T}_2|$.
	\[
	\mathfrak{d}_\infty(\bA_i,\bA_j)
	=\max_{l\neq i,j}
	\Big|\frac{1}{T_2}(\bW_l(\bvth-\widehat{\bvth})+\bu_l+\bmeta_l)'\Big((\bW_i-\bW_j)(\bvth-\widehat{\bvth})+(\bu_i-\bu_j)+(\bmeta_i-\bmeta_j)\Big)\Big|.
	\]
	There are nine terms after the expansion of the product. However, the product between $(\bu_l+\bmeta_l)$ and $(\bu_i-\bu_j)+(\bmeta_i-\bmeta_j)$ can be treated exactly the same way as in Lemma \ref{thm: IMD hsk}, and hence I only need to analyze the remainders. Clearly, 
	$$\max_{1\leq i,j\leq n}\max_{l\neq i, j}
	\Big|\frac{1}{T_2}(\bvth-\widehat{\bvth})'\bW_l'(\bW_i-\bW_j)
	(\bvth-\widehat{\bvth})\Big|\lesssim_\P\|\bvth-\widehat{\bvth}\|_2^2.$$
	Also,  note that $\E[\bw_{lt}u_{it}]=0$ for any $l, i,t$. Then, $\max_{i,j}\max_{l\neq i, j}
	|\frac{1}{T_2}(\bvth-\widehat{\bvth})'\bW_l'(\bu_i-\bu_j)|\lesssim_\P\frac{\sqrt{\log n}}{\sqrt{T}}
	\|\bvth-\widehat{\bvth}\|_2$ by the moment conditions in Assumption \ref{SA-Assumption: latent structure}(c) and application of maximal inequality as before. Finally,
	$\max_{1\leq i,j\leq n}\max_{l\neq i, j}
	 \Big|\frac{1}{T_2}(\bvth-\widehat{\bvth})'\bW_l'(\bmeta_i-\bmeta_j)\Big|\lesssim_\P\|\widehat{\bvth}-\bvth\|_2$.
	
	Using the argument in the proof of Lemma \ref{thm: IMD hsk} again, I have the following bound on the matching discrepancy: 
	$$\max_{1\leq i\leq n}\max_{1\leq k\leq K}\|\balpha_i-\balpha_{j_k(i)}\|_2\lesssim_\P
	(K/n)^{1/\ttd_\alpha}
	+\delta_{KT}^{-1}+h_{K,\varrho}^{2m}.$$
	
	\textit{Step 2: Local PCA.} As shown in Section \ref{SA-sec: general LPSA}, I apply the local PCA procedure to the subsample $\mathcal{T}_3$ to ensure the factor components and noises are uncorrelated. 
	Let $T_3=|\mathcal{T}_3|$. 
	I can apply the results of Theorem \ref{thm: uniform convergence of factors} with minor modification. Specifically, 
	\[
	\widehat{\bLambda}_{\subi}-\bLambda_{\subi}\bH_{\subi}
	=%\frac{1}{T}\bLambda_{\subi}(\bH_{\subi}')^{-1}
	%(\bF_{\subi}\bH_{\subi}-\widehat{\bF}_{\subi})'\widehat{\bF}_{\subi}+
	\frac{1}{T_3}\br_{\subi}'\widehat{\bF}_{\subi}+
	\frac{1}{T_3}\bu_{\subi}'\widehat{\bF}_{\subi}+
	\frac{1}{T_3}(\bvth-\widehat{\bvth})'\tilde{\bW}_{\subi}'\widehat{\bF}_{\subi}
	\]
	where $\tilde{\bW}_{\subi}$ is a $T_3\times K\times \ttd_w$ matrix with $\ell$th sheet given by $(\bw_{\mathcal{T}_3,j_1(i),\ell}, \cdots, \bw_{\mathcal{T}_3,j_K(i),\ell})$ associated with the $\ttd_w$-dimensional coefficient $\bvth$. Here $\bw_{\mathcal{T}_3,j_k(i),\ell}$ is the subvector of $\bw_{j_k(i),\ell}$ with the indices in $\mathcal{T}_3$. Note that the rate condition $\delta_{KT}h_{K,\varrho}^{2m}\lesssim 1$ implies that $h_{K,\varrho}^{2m}\lesssim h_{K,\alpha}^{m-1}$. Thus, additional approximation error arising from $\bW_i(\widehat{\bvth}-\bvth)$ is still dominated by leading approximation errors for $\eta_t(\balpha)$.  Then, the first two terms in the above decomposition can be treated exactly the same way as in the proof of Theorem \ref{thm: uniform convergence of factors}, and the third term is trivially $O_\P(\|\bvth-\widehat{\bvth}\|_2)$. Then, the result follows from Lemma \ref{SA-lem: slope of covariates}.
\end{proof}

\subsubsection*{Proof of Theorem \ref{SA-thm: QMLE}}
\begin{proof}
	I will only study the outcome equation; the treatment equation can be treated exactly the same way. I use $\bar{O}_\P$ and $\bar{o}_\P$ to denote the probability bound holds uniformly over $\subi$, where $\subi$ indexes local neighborhoods for unit $i$. The proof is divided into several steps.
	
	\textit{Step 0:} I first prepare some necessary notation and useful facts.
	For each $i$, a neighborhood $\mathcal{N}_i$ is obtained from the previous steps. Then, for $j\in\mathcal{N}_i$, $\mu_{\jmath}(\balpha_j)=
	\blambda_{j,\subi}'\bb_{\jmath,\subi}+r_{\jmath,\subi}(\balpha_j)$, where $\blambda_{j,\subi}'\bb_{\jmath,\subi}$ is the $L_2$ projection of $\mu_{\jmath}(\cdot)$ onto the space spanned by the monomial basis $\blambda_{j,\subi}$ described in the proof of Lemma \ref{lem: verify SA LPCA} (and in the main paper), and $r_{\jmath,\subi}(\balpha_j)$ is the resulting approximation error. By Assumption \ref{SA-Assumption: QMLE}(d), $\max_{1\leq i\leq n}\max_{j\in\mathcal{N}_i}|r_{\jmath,\subi}(\balpha_j)|\lesssim h_{K,\alpha}^{m}$. Note that $\bb_{\jmath,\subi}$ and $r_{\jmath,\subi}(\balpha_j)$ are defined with the subscript $\subi$, denoting that they implicitly depend on $i$, or more precisely, $\mathcal{N}_i$, due to the localization. 
	Also, recall that we can only identify $\bLambda_{\subi}$ up to a rotation $\bH_{\subi}$ used in Theorem \ref{thm: uniform convergence of factors}. However, we are free to insert $\bH_{\subi}$ and its inverse in the leading approximation terms $\blambda_{j,\subi}'\bb_{\jmath,\subi}$ without changing the approximation error. I will assume $\bb_{\jmath,\subi}$ and $\blambda_{j,\subi}$ have been rotated accordingly and thus omit $\bH_{\subi}$ to simplify notation.
	
	Let $\zeta_{j}=\bz_{j}'\bbeta_{\jmath}+\blambda_{j,\subi}'\bb_{\jmath,\subi}$ and $\widehat{\zeta}_{j}=\bz_{j}'\bbeta_{\jmath}+
	\widehat{\blambda}_{j,\subi}'\bb_{\jmath,\subi}$. The dependence of $\zeta_j$ and $\widehat{\zeta}_j$ on $\jmath$ and $\subi$ is suppressed. Then, $\widehat{\zeta}_j$ is the transformed mean with generated regressors. For $(\check{\bbeta}_{\jmath}', \check{\bb}_{\jmath,\subi}')'\in\mathbb{R}^{\ttd_z+\ttd_\lambda}$, define 
	\[
	\begin{split}
	&\bb^\dagger=\Big((\check{\bbeta}_{\jmath}-\bbeta_{\jmath})',\;
	(\bUpsilon(\check{\bb}_{\jmath,\subi}-\bb_{\jmath,\subi}))'\Big)',\quad
	\widehat{\bpi}_{j}=(\bz_{j}',\, \widehat{\blambda}_{j,\subi}'\bUpsilon^{-1})',\quad
	\widehat{\bG}_{j}=\widehat{\bpi}_{j}\widehat{\bpi}_{j}',\\
	&\bpi_{j}=(\bz_{j}',\, \blambda_{j,\subi}'\bUpsilon^{-1})',\quad
	\bG_{j}=\bpi_{j}\bpi_{j}', \quad
	\bUpsilon=\diag\{\bI_{\ttd_{\lambda,0}},\; h_{K,\alpha}\bI_{\ttd_{\lambda,1}},\;\cdots,\; h_{K,\alpha}^{m-1}\bI_{\ttd_{\lambda,m-1}}\}.
	\end{split}
	\]
	Note that $\bUpsilon$ is a normalizing diagonal matrix defined the same way as in Section \ref{SA-subsec: local factor structure}.
	The dependence of $\bb^\dagger$ on $\jmath$ and $\subi$ and the dependence of $\bpi_j$ and $\widehat{\bpi}_j$ on $\subi$ are  suppressed for simplicity. 
	In addition, for each $\jmath$, I can re-define the local neighborhood $\mathcal{N}_i$ by further selecting the subsample with $s_i=\jmath$. The renewed neighborhood is denoted by $\mathcal{N}_{i,\jmath}$.
	Now, I rewrite the objective function as
	\[
	l_n(\bb^\dagger):=\frac{1}{K}\sum_{j\in\mathcal{N}_{i,\jmath}}\Big(
	\mathcal{L}_{\tty}(\psi_{\tty}(\widehat{\zeta}_{j}+\widehat{\bpi}_{j}'\bb^\dagger), y_{j})-
	\mathcal{L}_{\tty}(\psi_{\tty}(\widehat{\zeta}_{j}), y_{j})\Big),
	\]
	and by optimization $l_n(\widehat{\bb}^\dagger)\geq 0$ for $\widehat{\bb}^\dagger=((\widehat{\bbeta}_{\jmath,\subi}-\bbeta_{\jmath})', (\bUpsilon(\widehat{\bb}_{\jmath,\subi}-\bb_{\jmath,\subi}))')'$.
	
	By Taylor expansion of $\mathcal{L}_{\tty}(\cdot,\cdot)$ around $\widehat{\zeta}_j$,
	\[
	\begin{split}
	l_n(\bb^\dagger)=\frac{1}{K}\sum_{j\in\mathcal{N}_{i,\jmath}}
	\mathcal{L}_{1,\tty}(\widehat{\zeta}_{j},y_{j})\widehat{\bpi}_{j}'\bb^{\dagger}+
	\frac{1}{2K}\sum_{j\in\mathcal{N}_{i,\jmath}}
	\mathcal{L}_{2,\tty}(\bar{\zeta}_{j},y_{j})(\bb^{\dagger})'\widehat{\bG}_{j}\bb^{\dagger}=:\bA_n\bb^\dagger+(\bb^\dagger)'\bQ_n\bb^\dagger/2,
	\end{split}
	\]	
	where $\bar{\zeta}_{j}$ is between $\widehat{\zeta}_{j}$ and $\widehat{\zeta}_{j}+\widehat{\bpi}_{j}'\bb^\dagger$. 
	
	\textit{Step 1:} Consider $\bA_n$ first. Rewrite it as
	\[
	\begin{split}
	\bA_n=&\frac{1}{K}\sum_{j\in\mathcal{N}_{i,\jmath}}\mathcal{L}_{1,\tty}(\zeta_{j}, y_{j})\bpi_{j}+
	\frac{1}{K}\sum_{j\in\mathcal{N}_{i,\jmath}}\mathcal{L}_{1,\tty}(\zeta_{j}, y_{j})(\widehat{\bpi}_{j}-\bpi_{j})+\\
	&\frac{1}{K}\sum_{j\in\mathcal{N}_{i,\jmath}}(\mathcal{L}_{1,\tty}(\widehat{\zeta}_{j}, y_{j})-\mathcal{L}_{1,\tty}(\zeta_{j}, y_{j}))\widehat{\bpi}_{j}
	=:J_1+J_2+J_3.
	\end{split}
	\]
	Let $\psi_{\tty}'(\zeta)=\frac{\partial}{\partial\zeta}\psi_{\tty}(\zeta)$. Recall that $\mathcal{L}_{1,\tty}(\zeta_{j}, y_{j}(\jmath))=(y_{j}(\jmath)-\psi_{\tty}(\zeta_j))/\bar{V}_{\tty}(\zeta_{j})=(\epsilon_{j,\jmath}+\bar{r}_{j,\jmath})/\bar{V}_{\tty}(\zeta_{j})$, $\bar{V}_{\tty}(\zeta_{j})=V_{\tty}(\zeta_{j})/\psi_{\tty}'(\zeta_{j})$ and
	$\bar{r}_{j,\jmath}=\psi_{\tty}(\bz_j'\bbeta_{\jmath}+\mu(\balpha_j))-\psi_{\tty}(\zeta_j)\lesssim h_{K,\alpha}^m$. 
	Only the generated regressors $\widehat{\blambda}_{j,\subi}$  contribute to $(\widehat{\bpi}_{j}-\bpi_{j})$. 
	Let $\mathcal{H}=\bar{\mathcal{F}}\cup\{\bm{d}_j\}_{j=1}^n\cup\{(\bx_i,\bw_i)\}_{i=1}^n$. $\{\epsilon_{j,\jmath}\}_{j=1}^n$ is independent over $j$ with mean zero conditional on $\mathcal{H}$.
	Thus, applying the maximal inequality as before, we have  $J_1=\bar{O}_\P(\sqrt{\log n}K^{-1/2}+h_{K,\alpha}^m)$.
	
	Next, by Theorem \ref{SA-thm: relevant FE},
	\[
	J_2=\bUpsilon^{-1}\times
	\frac{1}{K}\sum_{j\in\mathcal{N}_{i,\jmath}}
	\bar{V}_{\tty}(\zeta_{j})^{-1}
	\epsilon_{j,\jmath}(\widehat{\blambda}_{j,\subi}-\blambda_{j,\subi})+
	\bar{O}_\P(h_{K,\alpha}^m(\delta_{KT}^{-1}+h_{K,\alpha}^m+h_{K,\varrho}^{2m})).
	\]
	Since $\widehat{\blambda}_{j,\subi}$ is obtained using the covariates information only, the first term is a conditional mean zero sequence. By the truncation argument used before, it is $\bar{O}_\P(\sqrt{\log n}K^{-1/2}(\delta_{KT}^{-1}+h_{K,\alpha}^m+h_{K,\varrho}^{2m}))$, 
	
	\iffalse
	\[
	\begin{split}
	&\bUpsilon^{-1}\frac{1}{\sqrt{K}}\sum_{j\in\mathcal{N}_i}
	\bar{V}(\zeta_{jt'})^{-1}
	v_{jt'}(\widehat{\blambda}_{j}-\blambda_{j})\\
	=\;&\bUpsilon^{-1}\cdot\sqrt{K}\cdot \frac{1}{K}\sum_{j\in\mathcal{N}_i}\bar{V}(\zeta_{jt'})^{-1}
	v_{jt'}\Big(\frac{1}{T}\br_{\cdot j,\subi}'\widehat{\bF}_{\subi}+\frac{1}{T}\bveps_{\cdot j,\subi}'\widehat{\bF}_{\subi}\Big)\\
	\lesssim_\P\;& \bUpsilon^{-1}\times\Big(\sqrt{K}\delta_{KT}^{-1}K^{-1/2}+\sqrt{K}((KT)^{-1/2}+T^{-1})
	+\sqrt{K}\cdot\frac{1}{KT_\mathtt{P}}\sum_{j\in\mathcal{N}_i}
	\sum_{t=1}^{T}v_{jt'}\varepsilon_{jt}(\widehat{\bff}_{t,\subi}-\bff_{t,\subi}(\bH')^{-1})\\
	\lesssim_\P\;&\delta_{KT}^{-1}+\frac{\sqrt{K}}{T}+
	\delta_{KT}^{-1}h_K^{-m+1}\lesssim 1.
	\end{split}
	\]
	\fi
	
	$J_3$ can be written as
	\[
	\begin{split}
	&-\frac{1}{K}\sum_{j\in\mathcal{N}_{i,\jmath}}
	\Big(\frac{\psi_{\tty}(\widehat{\zeta}_{j})-\psi_{\tty}(\zeta_{j})}{\bar{V}_{\tty}(\zeta_{j})}\Big)\bpi_{j}+
	\frac{1}{K}\sum_{j\in\mathcal{N}_{i,\jmath}}
	\Big(\bar{V}_{\tty}(\widehat{\zeta}_{j})^{-1}-
	\bar{V}_{\tty}(\zeta_{j})^{-1}\Big)(\epsilon_{j,\jmath}+\varsigma_{j,\jmath}-\psi_{\tty}(\widehat{\zeta}_{j}))\bpi_{j}\\
	&+\frac{1}{K}\sum_{j\in\mathcal{N}_{i,\jmath}}
	\Big(\frac{y_j-\psi_{\tty}(\widehat{\zeta}_{j})}{\bar{V}_{\tty}(\widehat{\zeta}_{j})}-\frac{y_j-\psi_{\tty}(\zeta_{j})}{\bar{V}_{\tty}(\zeta_{j})}\Big)(\widehat{\bpi}_{j}-\bpi_{j})
	= -J_{3,1}+J_{3,2}+J_{3,3}.
	\end{split}
	\]
	Now, by Taylor expansion, Theorem \ref{SA-thm: relevant FE} and Assumption \ref{SA-Assumption: QMLE},
	\[
	J_{3,1}=\frac{1}{K}\sum_{j\in\mathcal{N}_{i,\jmath}}
	\frac{\bpi_{j}\psi_{\tty}'(\tilde{\zeta}_{j})(\widehat{\zeta}_j-\zeta_j)}{\bar{V}_{\tty}(\zeta_{j})}=\bar{O}_\P(\delta_{KT}^{-1}+h_{K,\alpha}^m+h_{K,\varrho}^{2m}),
	\]
	where $\tilde{\zeta}_j$ is between $\zeta_j$ and $\widehat{\zeta}_j$.
	By a similar argument used for $J_2$ and $J_{3,1}$, it follows that 
	$J_{3,2}$ and $J_{3,3}$ are 
	$\bar{O}_\P(\delta_{KT}^{-2}+h_{K,\alpha}^{2m}+h_{K,\varrho}^{4m})$.
	
	\textit{Step 2:} Consider $\bQ_n$. 
	Notice that 
	$$\mathcal{L}_{2,\tty}(\bar{\zeta}_j, y_j(\jmath))=-\frac{(y_j(\jmath)-\bar{\zeta}_j)\bar{V}_{\tty}'(\bar\zeta_j)}{\bar{V}^2_{\tty}(\bar{\zeta}_j)}-\frac{(\psi_{\tty}'(\bar{\zeta_j}))^2}{V_{\tty}(\bar{\zeta}_j)}=
	:-\frac{\epsilon_{j,\jmath}\bar{V}_{\tty}'(\bar\zeta_j)}{\bar{V}^2_{\tty}(\bar{\zeta}_j)}-\tilde{\mathcal{L}}(\bar{\zeta}_j,\varsigma_{j,\jmath}),$$ 
	where $\tilde{\mathcal{L}}(\bar{\zeta}_j,\varsigma_{j,\jmath})=\frac{(\varsigma_{j,\jmath}-\bar{\zeta}_j)\bar{V}_{\tty}'(\bar\zeta_j)}{\bar{V}^2_{\tty}(\bar{\zeta}_j)}+\frac{(\psi_{\tty}'(\bar{\zeta_j}))^2}{V_{\tty}(\bar{\zeta}_j)}$. Then,
	\[
	-\bQ_n=\frac{1}{K}\sum_{j\in\mathcal{N}_{i,\jmath}}\frac{\epsilon_{j,\jmath}\bar{V}_{\tty}'(\bar\zeta_j)}{\bar{V}^2_{\tty}(\bar{\zeta}_j)}\widehat{\bpi}_j\widehat{\bpi}_j'+\frac{1}{K}\sum_{j\in\mathcal{N}_{i,\jmath}}\tilde{\mathcal{L}}(\bar{\zeta}_j,\varsigma_{j,\jmath})\widehat{\bpi}_j\widehat{\bpi}_j'.
	\]
	
	For the second term, note 
	$
	\frac{1}{K}\sum_{j\in\mathcal{N}_{i,\jmath}}\tilde{\mathcal{L}}(\varsigma_{j,\jmath},\varsigma_{j,\jmath})\widehat{\bpi}_j\widehat{\bpi}_j'\gtrsim
	\frac{1}{K}\sum_{j\in\mathcal{N}_{i,\jmath}}\widehat{\bpi}_j\widehat{\bpi}_j'\gtrsim
	\frac{1}{K}\sum_{j\in\mathcal{N}_{i,\jmath}}\bpi_j\bpi_j'\gtrsim 1$,
	uniformly over $i$ w.p.a 1, where the first inequality follows by the boundedness of $\tilde{\mathcal{L}}(\varsigma_{j,\jmath},\varsigma_{j,\jmath})$ from below implied by Assumption \ref{SA-Assumption: QMLE}(b)(c)(e), the second inequality by the uniform convergence of $\widehat{\bpi}_j$ implied by Theorem \ref{SA-thm: relevant FE}, and the last by the non-collinearity condition given in Assumption \ref{SA-Assumption: QMLE}(e) and overlapping condition in Assumption \ref{SA-Assumption: ID-counterfactual}. Therefore, there exists a compact neighborhood $\mathscr{B}$ around zero such that for all $\breve{\bb}^\dagger\in\mathscr{B}$, the above lower bound still holds with $\tilde{\mathcal{L}}(\varsigma_{j,\jmath},\varsigma_{j,\jmath})$ replaced by $\tilde{\mathcal{L}}(\widehat{\zeta}_j+\widehat{\bpi}'\breve{\bb}^\dagger,\varsigma_{j,\jmath})$. 
	
	Regarding the first term, note that $\{\epsilon_{j,\jmath}\}$ is independent over $j$ with mean zero conditional on $\mathcal{H}=\bar{\mathcal{F}}\cup\{\bm{d}_j\}_{j=1}^n\cup\{(\bx_i,\bw_i)\}_{i=1}^n$. Again, apply a truncation argument to show uniform convergence of the first term. Define $\epsilon_{j,\jmath}^-=\epsilon_{j,\jmath}\I(|\epsilon_{j,\jmath}|\leq \tau_n)$ and $\epsilon_{j,\jmath}^+=\epsilon_{j,\jmath}-\epsilon_{j,\jmath}^-$ and $\tau_n\asymp\sqrt{K/\log (n\vee T)}$. For the truncated part, conditional on the data, define
	\[
	\begin{split}
	\mathcal{T}=\Big\{\bt=(t_1,\cdots, t_n)\in\mathbb{R}^n:\; &t_j=\frac{d_{j}(\jmath)\I(j\in\mathcal{N}_i)\bar{V}_{\tty}'(\widehat{\zeta}_j+\widehat{\bpi}_{j}\bb^\dagger)\widehat{\pi}_{k,j}\widehat{\pi}_{l,j}'}{\bar{V}^2_{\tty}(\widehat{\zeta}_j+\widehat{\bpi}_j\check{\bb})}\Big(\epsilon_{j,\jmath}^--\E[\epsilon_{j,\jmath}^-|\mathcal{H}]\Big),\\
	&\check{\bb}^\dagger\in\mathscr{B}, 1\leq i\leq n, 1\leq k, l\leq \ttd_z+\ttd_\lambda
	\Big\}.
	\end{split}
	\]
	Define the norm $\|\cdot\|_{n,2}$ on $\mathbb{R}^n$ by $\|\bt\|^2_{n,2}=\E_n[t_j^2]$. For any $\varepsilon>0$, the covering number $N(\mathcal{T},\|\cdot\|_{n,2},\varepsilon)$ is the infimum of the cardinality of $\varepsilon$-nets of $\mathcal{T}$.
	Let $\{\omega_i\}_{i=1}^n$ be a sequence of independent Rademacher random variables that are independent of the data, and $\E_{\bomega}[\cdot]$ denotes the expectation with respect to the distribution of $\bomega=(\omega_1,\cdots,\omega_n)$.
	By Symmetrization Inequality and Dudley's inequality \citep{Dudley_1967_JFA},
	{\small
	\[
	\E\Big[\max_{1\leq i\leq n,\atop 1\leq k,l\leq \ttd_z+\ttd_\lambda}\sup_{\breve{\bb}^\dagger\in\mathbb{R}}|\frac{1}{\sqrt{n}}
	\sum_{j=1}^{n}t_j|\Big|\mathcal{H}\Big]
	\leq 2\E\Big[\E_{\bomega}\Big[\sup_{\tau\in\mathbb{R}}|\frac{1}{\sqrt{n}}
	\sum_{j=1}^{n}t_j\omega_j|\Big]\Big|\mathcal{H}\Big]
	\lesssim
	\int_0^{\Theta}\sqrt{\log N(\mathcal{T},\|\cdot\|_{n,2},\varepsilon)}d\varepsilon,
	\]
    }

	\noindent where the diameter $\Theta:=2\sup_{\bt\in\mathcal{T}}\|\bt\|_{n,2}\lesssim_\P\tau_n\sqrt{K/n}$ by truncation.
	Since $\mathscr{B}$ is compact and $\bar{V}_{\tty}'$ and $\bar{V}_{\tty}$ are Lipschitz with respect to $\check{\bb}^\dagger$, it is well known that the covering number for $\mathcal{T}$ is $N(\mathcal{T},\|\cdot\|_{n,2},\varepsilon)\lesssim n(1/\varepsilon)^2$, which leads to $\sup_{\breve{\bb}\in\mathscr{B}}\max_{i,k,l}|\frac{n}{K}\E_n[t_j]|\lesssim_\P\sqrt{\log n}\tau_n/\sqrt{K}=o_\P(1)$. For the tails, 
	it is $o_\P(1)$ uniformly over $i,k,l$ and $\breve{\bb}^\dagger$ by Markov inequality, the rate condition and the boundedness condition implied by Assumption \ref{SA-Assumption: QMLE}(c)(d)(e).  Thus, the first term in the decomposition of $\bQ_n$ is $o_\P(1)$ uniformly over $1\leq i\leq n$ and $\breve{\bb}^\dagger\in\mathscr{B}$.
	
	Therefore, if the maximizer $\widehat{\bb}^{\dagger}$ is searched within $\mathscr{B}$, by optimality, the above results suffices to show that  $\widehat{\bb}^{\dagger}=\bar{O}_\P(\delta_{KT}^{-1}+h_{K,\alpha}^m+h_{K,\varrho}^{2m})$. But note that by concavity of $\mathcal{L}_{\tty}(\cdot, \cdot)$ assumed in Assumption \ref{SA-Assumption: QMLE}(b), it is also the maximizer over the whole parameter space.
		
	\textit{Step 3:} To derive the asymptotic expansion, note that the first-order condition leads to
	\[
	\begin{split}
	0&=\frac{1}{K}\sum_{j\in\mathcal{N}_{i,\jmath}}\mathcal{L}_{1,\tty}(\widehat{\zeta}_j+\widehat{\bpi}'_{j}\widehat{\bb}^\dagger,y_j)\widehat{\bpi}_j\\
	&=\frac{1}{K}\sum_{j\in\mathcal{N}_{i,\jmath}}\mathcal{L}_{1,\tty}(\widehat{\zeta}_j,y_j)\widehat{\bpi}_j+
	\frac{1}{K}\sum_{j\in\mathcal{N}_{i,\jmath}}\mathcal{L}_{2,\tty}(\tilde{\zeta}_j,y_j)\widehat{\bpi}_j\widehat{\bpi}_j'\widehat{\bb}^\dagger
	=\bA_n+\bV_n\widehat{\bb}^\dagger.
	\end{split}
	\]
	where $\tilde{\zeta}_j$ is between $\widehat{\zeta}_j$ and $\widehat{\zeta}_j+\widehat{\bpi}_j'\widehat{\bb}^\dagger$.
	$\bA_n$ has been analyzed before. Now consider $\bV_n$: 
	\[
	\begin{split}
	\bV_n=&\frac{1}{K}\sum_{j\in\mathcal{N}_{i,\jmath}}\mathcal{L}_{2,\tty}(\zeta_{j},y_{j})\bG_{j}
	+\frac{1}{K}\sum_{j\in\mathcal{N}_{i,\jmath}}\mathcal{L}_{2,\tty}(\zeta_{j},y_{j})(\widehat{\bG}_{j}-\bG_j)+\\
	&\frac{1}{K}\sum_{j\in\mathcal{N}_{i,\jmath}}(\mathcal{L}_{2,\tty}(\tilde{\zeta}_{j},y_{j})-\mathcal{L}_{2,\tty}(\zeta_{j},y_{j}))\bG_{j}+
	\frac{1}{K}\sum_{j\in\mathcal{N}_{i,\jmath}}(\mathcal{L}_{2,\tty}(\tilde{\zeta}_{j},y_{j})-\mathcal{L}_{2,\tty}(\zeta_{j},y_{j}))(\widehat{\bG}_{j}-\bG_j).
	\end{split}
	\]
	By Lemma \ref{thm: uniform convergence of factors}, $\max_{1\leq i\leq n}\|\widehat{\bpi}_{i}-\bpi_{i}\|_2\lesssim_\P\delta_{KT}^{-1}+h_{K,\alpha}^m+h_{K,\varrho}^{2m}$.
    Then, by Assumption \ref{SA-Assumption: QMLE}(e), the second and the fourth terms are all $\bar{O}_\P(\delta_{KT}^{-1}+h_{K,\alpha}^m+h_{K,\varrho}^{2m})$.
	By Assumption \ref{SA-Assumption: QMLE}(a), the third term is $\bar{O}_\P(\|\widehat{\bb}^\dagger\|_2)$.  
	Finally, the first term, by Assumption \ref{SA-Assumption: QMLE}(b)(e), is strictly negative definite uniformly over $i$.
	In fact, it satisfies that
	\[
	\max_{1\leq i\leq n}
	\Big|\frac{1}{K}\sum_{j\in\mathcal{N}_{i,\jmath}}\mathcal{L}_{2,\tty}(\psi_{\tty}^{-1}(\varsigma_{j,\jmath}),y_{j})\bG_{j}-
	\E\Big[\frac{1}{K}\sum_{j\in\mathcal{N}_{i,\jmath}}\mathcal{L}_{2,\tty}(\psi_{\tty}^{-1}(\varsigma_{j,\jmath}),y_{j})\bG_{j}\Big|\bar{\mathcal{F}},\{\bx_i,\bw_i\}_{i=1}^n\Big]\Big|\lesssim_\P\delta_{KT}^{-1}
	\]
	by Assumption \ref{SA-Assumption: QMLE}(c)(d)(e) and the rate condition. Also by Assumption \ref{SA-Assumption: QMLE}(a), 
	$$\max_{1\leq i\leq n}
	\Big|\frac{1}{K}\sum_{j\in\mathcal{N}_{i,\jmath}}(\mathcal{L}_{2,\tty}(\zeta_j,y_j)-\mathcal{L}_{2,\tty}(\psi_{\tty}^{-1}(\varsigma_{j,\jmath},y_{j}))\bG_{j}\Big|\lesssim_\P h_{K,\alpha}^m.$$ 
	Then, by power series expansion of matrix inverse, we have $\bV_n^{-1}-\bV_{\subi}^{-1}=\bar{O}_\P(\delta_{KT}^{-1}+h_{K,\alpha}^m+h_{K,\varrho}^{2m})$ where
	$\bV_{\subi}:=\frac{1}{K}\E[\sum_{j\in\mathcal{N}_{i,\jmath}}\mathcal{L}_{2,\tty}(\psi_{\tty}^{-1}(\varsigma_{j,\jmath}),y_{j})\bG_{j}|\bar{\mathcal{F}},\{\bx_i,\bw_i\}_{i=1}^n]$.

	Now, further decompose the following difference: 
	$(\bz_{i}'\widehat{\bbeta}_{\jmath,\subi}+\widehat{\blambda}_{i,\subi}'\widehat{\bb}_{\jmath,\subi})-
	(\bz_{i}'\bbeta_\jmath+\mu_\jmath(\balpha_i))
	=(\bz_{i}'\widehat{\bbeta}_{\jmath,\subi}+\widehat{\blambda}_{i,\subi}'\widehat{\bb}_{\jmath,\subi}-
	\bz_{i}'\bbeta_\jmath-\widehat{\blambda}_{i,\subi}'\bb_{\jmath,\subi})+
	(\widehat{\blambda}_{i,\subi}'\bb_{\jmath,\subi}-\blambda_{i,\subi}'\bb_{\jmath,\subi})+
	(\blambda_{i,\subi}'\bb_{\jmath,\subi}-\mu_\jmath(\balpha_i))$.
	The previous steps have constructed bounds for the first term that corresponds to the convergence of the estimated coefficients; the second term corresponds to the convergence of generated regressors and hence can be bounded via Theorem \ref{SA-thm: QMLE}; and the last term is simply the approximation error. Therefore, this difference is  $\bar{O}_\P(\delta_{KT}^{-1}+h_{K,\alpha}^m+h_{K,\varrho}^{2m})$. Since $\psi_{\tty}'(\cdot)$ is assumed to be continuous, the first result follows.
	
	The asymptotic expansion then is given by
	\begin{equation}\label{eq: asymptotic expansion}
	\begin{split}
	\widehat{\varsigma}_{i,\jmath}-\varsigma_{i,\jmath}=&
	\psi_{\tty}'\Big(\psi_{\tty}^{-1}(\varsigma_{i,\jmath})\Big)\times
	\bigg\{\bpi_i'\bV_{\subi}^{-1}
	\Big[\frac{1}{K}\sum_{j\in\mathcal{N}_{i,\jmath}}
	\Big(\mathcal{L}_{1,\tty}(\psi_{\tty}^{-1}(\varsigma_{j,\jmath}), y_{j})-\\
	&\frac{\psi_{\tty}'(\psi_{\tty}^{-1}(\varsigma_{i,\jmath}))}{\bar{V}_{\tty}(\psi_{\tty}^{-1}(\varsigma_{i,\jmath}))}(\widehat{\blambda}_{j,\subi}-\blambda_{j,\subi})'\bb_{\jmath,\subi}\Big)\bpi_j\Big]
	+(\widehat{\blambda}_{i,\subi}-\blambda_{i,\subi})'\bb_{\jmath,\subi}+r_{\jmath,\subi}(\balpha_i)\bigg\}\\
	&+\bar{O}_\P(\delta_{KT}^{-2}+h_{K,\alpha}^{2m}+h_{K,\varrho}^{4m}),
	\end{split}.
	\end{equation}
\end{proof}

\subsubsection*{Proof of Theorem \ref{SA-thm: pointwise inference}}
\begin{proof}
	Let $\tilde{\varphi}_{i,\jmath,\jmath'}:=\frac{d_i(\jmath')\varsigma_{i,\jmath}}{p_{\jmath'}}+\frac{p_{i,\jmath'}d_i(\jmath)(y_i-\varsigma_{i,\jmath})}{p_{\jmath'}p_{i,\jmath}}-\theta_{\jmath,\jmath'}$.
	By some algebra, 
	\begin{align*}
	\sqrt{n}(\widehat{\theta}_{\jmath,\jmath'}-
	\theta_{\jmath,\jmath'})
	%=\,&\frac{1}{\sqrt{n}}\sum_{i=1}^{n}\tilde{\varphi}_{i,\jmath,\jmath'}+
	%\frac{1}{\sqrt{n}}\sum_{i=1}^n\bigg[\frac{d_i(\jmath')\widehat{\varsigma}_{i,\jmath}}{\widehat{p}_{\jmath'}}
	%-\frac{d_i(\jmath')\varsigma_{i,\jmath}}{p_{\jmath'}}
	%+\frac{\widehat{p}_{i,\jmath'}}{\widehat{p}_{\jmath'}}\frac{d_i(\jmath)(y_{i}-\widehat{\varsigma}_{i,\jmath})}{\widehat{p}_{i,\jmath}}
	%-\frac{p_{i,\jmath'}}{p_{\jmath'}}\frac{d_i(\jmath)(y_{i}-\varsigma_{i,\jmath})}{p_{i,\jmath}}\bigg]\\
	%=\,&\frac{1}{\sqrt{n}}\sum_{i=1}^n\tilde{\varphi}_{i,\jmath,\jmath'}+\frac{1}{\sqrt{n}}\sum_{i=1}^n\mathscr{R}_{i}
	%+\Big(\frac{p_{\jmath'}}{\widehat{p}_{\jmath'}}-
	%\frac{p_{\jmath'}}{p_{\jmath'}}\Big)\cdot\frac{1}{\sqrt{n}}\sum_{i=1}^n\mathscr{R}_{i}+\\
	%&\qquad\Big(\frac{p_{\jmath'}}{\widehat{p}_{\jmath'}}-
	%\frac{p_{\jmath'}}{p_{\jmath'}}\Big)\cdot
	%\frac{1}{\sqrt{n}}\sum_{i=1}^n\bigg[
	%\frac{d_i(\jmath')\varsigma_{i,\jmath}}{p_{\jmath'}}+
	%\frac{p_{i,\jmath'}}{p_{\jmath'}}\frac{d_i(\jmath)(y_{i}-\varsigma_{i,\jmath})}{p_{i,\jmath}}
	%\bigg]\\
	%=\,&\frac{1}{\sqrt{n}}\sum_{i=1}^n\tilde{\varphi}_{i,\jmath,\jmath'}+\frac{1}{\sqrt{n}}\sum_{i=1}^n\mathscr{R}_{i}+
	%\Big(\frac{p_{\jmath'}}{\widehat{p}_{\jmath'}}-
	%\frac{p_{\jmath'}}{p_{\jmath'}}\Big)\cdot\frac{1}{\sqrt{n}}\sum_{i=1}^n\mathscr{R}_{i}+\\
	%&\qquad\sqrt{n}\frac{p_{\jmath'}-\widehat{p}_{\jmath'}}{\widehat{p}_{\jmath'}}\E_n\bigg[
	%\frac{d_i(\jmath')\varsigma_{i,\jmath}}{p_{\jmath'}}+
	%\frac{p_{i,\jmath'}}{p_{\jmath'}}\frac{d_i(\jmath)(y_{i}-\varsigma_{i,\jmath})}{p_{i,\jmath}}\bigg]\\
	=&\frac{1}{\sqrt{n}}\sum_{i=1}^n\tilde{\varphi}_{i,\jmath,\jmath'}+\frac{1}{\sqrt{n}}\sum_{i=1}^n\mathscr{R}_{i}+\Big(\frac{p_{\jmath'}}{\widehat{p}_{\jmath'}}-\frac{p_{\jmath'}}{p_{\jmath'}}\Big)\cdot\frac{1}{\sqrt{n}}\sum_{i=1}^n\mathscr{R}_{i}+
	\sqrt{n}\frac{p_{\jmath'}-\widehat{p}_{\jmath'}}{p_{\jmath'}}\theta_{\jmath,\jmath'}+\\
	\sqrt{n}(p_{\jmath'}-\widehat{p}_{\jmath'})&\theta_{\jmath,\jmath'}\Big(\frac{1}{\widehat{p}_{\jmath'}}-\frac{1}{p_{\jmath'}}\Big)
	+\sqrt{n}\frac{p_{\jmath'}-\widehat{p}_{\jmath'}}{\widehat{p}_{\jmath'}}\Big(\E_n\left[
	\frac{d_i(\jmath')\varsigma_{i,\jmath}}{p_{\jmath'}}+
	\frac{p_{i,\jmath'}}{p_{\jmath'}}\frac{d_i(\jmath)(y_{i}-\varsigma_{i,\jmath})}{p_{i,\jmath}}\right]-\theta_{\jmath,\jmath'}\Big)\\
	=&\frac{1}{\sqrt{n}}\sum_{i=1}^n\varphi_{i,\jmath,\jmath'}+o_\P(1),
	\end{align*}
	where $\frac{1}{\sqrt{n}}\sum_{i=1}^n\mathscr{R}_{i}$ is given by
	\begin{align*}
	&\frac{1}{\sqrt{n}}\sum_{i=1}^n\bigg[\frac{p_{i,\jmath'}}{p_{\jmath'}}d_i(\jmath)(y_{i}-\varsigma_{i,\jmath})\Big(
	\frac{1}{\widehat{p}_{i,\jmath}}-\frac{1}{p_{i,\jmath}}\Big)\bigg]+
	\frac{1}{\sqrt{n}}\sum_{i=1}^n\bigg[\Big(\frac{\widehat{p}_{i,\jmath'}-p_{i,\jmath'}}{p_{\jmath'}}\Big)\frac{d_i(\jmath)(y_{i}-\varsigma_{i,\jmath})}{\widehat{p}_{i,\jmath}}\bigg]\\
	&+\frac{1}{\sqrt{n}}\sum_{i=1}^n\bigg[\Big(\frac{d_i(\jmath')}{p_{\jmath'}}-
	\frac{\widehat{p}_{i,\jmath'}d_i(\jmath)}{p_{\jmath'}\widehat{p}_{i,\jmath}}\Big)(\widehat{\varsigma}_{i,\jmath}-\varsigma_{i,\jmath})\bigg]
	=:I_1+I_2+I_3.
	\end{align*}
	The last step in the above calculation follows by the following argument. For $I_1$,
	define a conditioning set $\mathcal{H}=\{\bm{d}_{i}\}_{i=1}^n\cup\bar{\mathcal{F}}\cup\{\bx_i,\bw_i\}_{i=1}^n$. By Assumption \ref{SA-Assumption: ID-counterfactual} and \ref{SA-Assumption: QMLE}, $I_1$ is mean zero conditional on $\mathcal{H}$ with
	$\E[I_1^2|\mathcal{H}]
	\lesssim \frac{1}{n}\sum_{i=1}^n(\widehat{p}_{i,\jmath'}-p_{i,\jmath'})^2=o_\P(1)$.
	$I_2$ can be treated similarly.	
	
	For $I_3$,
	$p_{\jmath'}I_3=\frac{1}{\sqrt{n}}\sum_{i=1}^n[(\widehat{\varsigma}_{i,\jmath}-\varsigma_{i,\jmath})(d_i(\jmath')-\frac{p_{i,\jmath'}d_i(\jmath)}{p_{i,\jmath}})]+
	\frac{1}{\sqrt{n}}\sum_{i=1}^n[(\widehat{\varsigma}_{i,\jmath}-\varsigma_{i,\jmath})(\frac{p_{i,\jmath'}d_i(\jmath)}{p_{i,\jmath}}-\frac{\widehat{p}_{i,\jmath'}d_i(\jmath)}{\widehat{p}_{i,\jmath}})]
	=:I_{3,1}+I_{3,2}$. 
	Regarding $I_{3,2}$, by Cauchy-Schwarz inequality, Theorem \ref{SA-thm: QMLE} and the rate condition, 
	$|I_{3,2}|\lesssim \sqrt{n}(\E_n[(\widehat{\varsigma}_{i,\jmath}-\varsigma_{i,\jmath})^2])^{1/2}(\E_n[(\widehat{p}_{i,\jmath'}-p_{i,\jmath'})^2])^{1/2}=o_\P(1)$.
	For $I_{3,1}$, first notice that
	$I_{3,1}=\frac{1}{\sqrt{n}}\sum_{i=1}^n[(\widehat{\varsigma}_{i,\jmath}-\varsigma_{i,\jmath})v_{i,\jmath'}]-
	\frac{1}{\sqrt{n}}\sum_{i=1}^n[(\widehat{\varsigma}_{i,\jmath}-\varsigma_{i,\jmath})v_{i,\jmath}\frac{p_{i,\jmath'}}{p_{i,\jmath}}]=:I_{3,1,1}+I_{3,1,2}$.
	Recall that $v_{i,\jmath}=d_{i}(\jmath)-\E[d_i(\jmath)|\bz_i,\balpha_i]$. I will focus on the first term only and the second one can be treated similarly. Further expand $I_{3,1,1}$:
	\[
	\begin{split}
	I_{3,1,1}%&=\sqrt{n}\cdot\frac{1}{n}\sum_{i=1}^{n}v_{i,\jmath'}
	%(\psi_{\tty}(\bz_i'\widehat{\bbeta}_{\jmath,\subi}+\widehat{\lambda}_i'\widehat{\bb}_{\lambda,\jmath})-\varsigma_{i,\jmath})\\ 
	&=\sqrt{n}\cdot\frac{1}{n}\sum_{i=1}^{n}v_{i,\jmath'}
	\Big(\psi_{\tty}(\bz_i'\widehat{\bbeta}_{\jmath,\subi}+\widehat{\blambda}_{i,\subi}'\widehat{\bb}_{\jmath,\subi})-
	\psi_{\tty}(\bz_i'\bbeta_{\jmath}+\blambda_{i,\subi}'\bb_{\jmath,\subi})-r_{\jmath,\subi}(\balpha_i)\Big)\\
	&=\sqrt{n}\cdot\frac{1}{n}\sum_{i=1}^{n}v_{i,\jmath'}
	\Big(\psi_{\tty}(\bz_i'\widehat{\bbeta}_{\jmath,\subi}+\widehat{\blambda}_{i,\subi}'\widehat{\bb}_{\jmath,\subi})-
	\psi_{\tty}(\bz_i'\bbeta_{\jmath}+\blambda_{i,\subi}'\bb_{\jmath,\subi})\Big)+o_\P(1)\\
	&=\sqrt{n}\cdot\frac{1}{n}\sum_{i=1}^{n}v_{i,\jmath'}
	\Big(\psi_{\tty}(\bz_i'\widehat{\bbeta}_{\jmath,\subi}+\widehat{\blambda}_{i,\subi}'\widehat{\bb}_{\jmath,\subi})-
	\psi_{\tty}(\bz_i'\bbeta_{\jmath}+\widehat{\blambda}_{i,\subi}'\bb_{\jmath,\subi})\Big)+o_\P(1)\\
	&=\sqrt{n}\cdot\frac{1}{n}\sum_{i=1}^{n}v_{i,\jmath'}\psi_{\tty}'(\bz_i\bbeta_{\jmath}+\mu(\balpha_i))
	\Big(\bz_i'(\widehat{\bbeta}_{\jmath,\subi}-\bbeta_{\jmath})+\blambda_{i,\subi}'(\widehat{\bb}_{\jmath,\subi}-\bb_{\jmath,\subi})\Big)+o_\P(1),
	\end{split}
	\]
	where the second line holds by $\max_{i}|r_{\jmath,\subi}(\balpha_i)|\lesssim h_{K,\alpha}^{m}$, the third by the fact that the generated regressors do not depend on $d_{i}(\jmath')$ and are consistent, and the last line by Taylor expansion of $\psi_{\tty}(\cdot)$ and the rate condition. Importing the notation from the proof of Theorem \ref{SA-thm: QMLE}, I further plug in the asymptotic linear expansion \eqref{eq: asymptotic expansion} for $\widehat{\varsigma}_{i,\jmath}$, and the leading term in the last line then becomes
	\[
	\begin{split}
	&%\sqrt{n}\cdot\frac{1}{n}\sum_{i=1}^{n}v_{i,\jmath'}\psi_{\tty}'(\psi_{\tty}^{-1}(\varsigma_{i,\jmath}))
	%\Big(\bpi_{i,\subi}'(\widehat{\bb}^\dagger_{\jmath,\subi}-\bb^\dagger_{\jmath,\subi})\Big)=
	\sqrt{n}\cdot\frac{1}{Kn}\sum_{i=1}^{n}v_{i,\jmath'}\psi_{\tty}'(\zeta_{i,\jmath,\subi})\bpi_{i,\subi}'\bV_{\subi}^{-1}\times
	\bigg[\sum_{j\in\mathcal{N}_{i,\jmath}}
	\Big(\mathcal{L}_{1,\tty}(\psi_{\tty}^{-1}(\varsigma_{j,\jmath}),y_j)-\\
	&\hspace{15em}\frac{\psi_{\tty}'(\psi_{\tty}^{-1}(\varsigma_{i,\jmath}))}{\bar{V}_{\tty}(\psi_{\tty}^{-1}(\varsigma_{i,\jmath}))}(\widehat{\blambda}_{j,\subi}-\blambda_{j,\subi})'\bb_{\jmath,\subi}\Big)\bpi_{j,\subi}\bigg]+o_\P(1)
	\end{split}
	\]
	by the rate condition. Note that for clarity of expression, I add back the subscript $\subi$ to $\bpi_j$ defined in the proof of Theorem \ref{SA-thm: QMLE}.
	There are two terms in the square brackets.  Specifically,
	the first term we need to consider is
	{\small
	\[
	\begin{split}
	&\sqrt{n}\cdot\frac{1}{Kn}\sum_{i=1}^{n}v_{i,\jmath'}\psi_{\tty}'(\psi_{\tty}^{-1}(\varsigma_{j,\jmath}))
	\bpi_{i,\subi}'\bV_{\subi}^{-1}\sum_{j=1}^{n}\bpi_{j,\subi}d_j(\jmath)\I(j\in\mathcal{N}_i)\epsilon_{j,\jmath}/\bar{V}_{\tty}(\psi_{\tty}^{-1}(\varsigma_{j,\jmath}))\\
	=&\sqrt{n}\cdot\frac{1}{n}
	\sum_{j=1}^{n}\Big\{\epsilon_{j,\jmath}d_j(\jmath)/\bar{V}_{\tty}(\psi_{\tty}^{-1}(\varsigma_{j,\jmath}))
	\Big(\frac{1}{K}\sum_{i=1}^{n}v_{i,\jmath'}
	\psi_{\tty}'(\psi_{\tty}^{-1}(\varsigma_{j,\jmath}))
	\bpi_{i,\subi}'\bV_{\subi}^{-1}\bpi_{j,\subi}
	\I(j\in\mathcal{N}_i)\Big)\Big\}\\
	=&:\sqrt{n}\cdot\frac{1}{n}
	\sum_{j=1}^{n}\epsilon_{j,\jmath}d_j(\jmath)/\bar{V}_{\tty}(\psi_{\tty}^{-1}(\varsigma_{j,\jmath}))a_j,
	\end{split}
	\] 
    }
    
    \vspace{-1em}
	\noindent which is mean zero conditional on $\mathcal{H}$ and $\frac{1}{n}\sum_{j=1}^{n}a_j^2=o_\P(1)$ since $\{v_{i,\jmath}\}$ is independent of $\{\mathcal{N}_i\}$ and the number of $j$ used for matching satisfies that
	$S_j:=\sum_{i=1}^{n}\I(j\in\mathcal{N}_i)\lesssim_\P K$ 
	by Lemma \ref{lem: number of times for matching}.	
	For the second term, 
	\begin{small}
	\[
	\begin{split}
	&\quad\;\sqrt{n}\cdot\frac{1}{Kn}\sum_{i=1}^{n}v_{i,\jmath'}\psi_{\tty}'(\psi_{\tty}^{-1}(\varsigma_{i,\jmath}))
	\bpi_{i,\subi}'\bV_{\subi}^{-1}
	\sum_{j=1}^{n}\frac{\psi_{\tty}'(\psi_{\tty}^{-1}(\varsigma_{j,\jmath}))}{\bar{V}_{\tty}(\psi_{\tty}^{-1}(\varsigma_{j,\jmath}))}(\widehat{\blambda}_{j,\subi}-\blambda_{j,\subi})'\bb_{\jmath,\subi}\bpi_{j,\subi}d_j(\jmath)\I(j\in\mathcal{N}_i)\\
	&=\sqrt{n}\cdot\frac{1}{Kn}
	\sum_{j=1}^{n}\frac{d_j(\jmath)\psi_{\tty}'(\psi_{\tty}^{-1}(\varsigma_{j,\jmath}))}{\bar{V}_{\tty}(\psi_{\tty}^{-1}(\varsigma_{j,\jmath}))}
	\sum_{i=1}^{n}v_{i,\jmath'}\psi_{\tty}'(\psi_{\tty}^{-1}(\varsigma_{i,\jmath}))
	\bpi_{i,\subi}'\bV_{\subi}^{-1}\bpi_{j,\subi}\I(j\in\mathcal{N}_i)(\widehat{\blambda}_{j,\subi}-\blambda_{j,\subi})'\bb_{\jmath,\subi}\\	
	%&\quad\;\sqrt{n}\cdot\frac{1}{Kn}\sum_{i=1}^{n}v_{i,\jmath'}\psi_{\tty}'(\zeta_{i,\jmath,\subi})
	%\bpi_{i,\subi}'\bV_{\subi}^{-1}\sum_{j=1}^{n}\bpi_{j,\subi}d_j(\jmath)\I(j\in\mathcal{N}_i)(\psi_{\tty}(\widehat{\zeta}_{j,\jmath})-\psi_{\tty}(\zeta_{j,\jmath}))/\bar{V}(\zeta_{j,\jmath})\\
	%&=\sqrt{n}\cdot\frac{1}{Kn}\sum_{i=1}^{n}v_{i,\jmath'}\psi_{\tty}'(\zeta_{i,\jmath,\subi})
	%\bpi_{i,\subi}'\bV_{\subi}^{-1}\sum_{j=1}^{n}\bpi_{j,\subi}d_j(\jmath)\I(j\in\mathcal{N}_i)\psi_{\tty}'(\zeta_{j,\jmath})(\widehat{\zeta}_{j,\jmath}-\zeta_{j,\jmath})/\bar{V}(\zeta_{j,\jmath})+o_\P(1)\\
	%&=\sqrt{n}\cdot\frac{1}{Kn}
	%\sum_{j=1}^{n}d_j(\jmath)
	%\sum_{i=1}^{n}v_{i,\jmath'}\psi_{\tty}'(\zeta_{i,\jmath,\subi})
	%\bpi_{i,\subi}'\bV_{\subi}^{-1}\bpi_j\I(j\in\mathcal{N}_i)\psi_{\tty}'(\zeta_j)(\widehat{\zeta}_j-\zeta_j)/\bar{V}(\zeta_{j,\jmath})+o_\P(1)\\
	&\lesssim_\P\sqrt{n}K^{-1/2}(
	\delta_{KT}^{-1}+h_{K,\alpha}^m+h_{K,\varrho}^{2m}).
	\end{split}
	\]
	\end{small}
    
    \vspace{-1em}
	\noindent The last step follows by the fact that $\{v_{i,\jmath'}\}$ is independent of $\{\mathcal{N}_i\}$ and $\{\widehat{\blambda}_{j,\subi}\}$ and Lemma \ref{lem: number of times for matching}.
	
	%the sample splitting scheme, conditional on $\mathcal{A}_2$
	%\[
	%\E[R_{31}^2|\mathcal{A}_2]\lesssim 
	%\frac{1}{N}\sum_{i\in\mathcal{N}_1}(\widehat{\varsigma}_{t}(\bx_{it},\balpha_i)-\varsigma_{i}(\bx_{it},\balpha_i))^2=o_\P(1).
	%\]

	Finally, since  $\sqrt{n}(\widehat{p}_{\jmath'}-p_{\jmath'})=O_\P(1)$, 
	the desired result in (i) follow.
	
	Now, consider the variance estimation. Note that
	\[
	\sigma_{\jmath,\jmath'}^2:=\V[\varphi_{i,\jmath,\jmath'}]=\E\Big[\frac{p_{i,\jmath'}(\varsigma_{i,\jmath}-\theta_{\jmath,\jmath'})^2}{p_{\jmath'}^2}\Big]+
	\E\Big[\frac{p_{i,\jmath'}^2\sigma_{i,\jmath}^2}{p_{\jmath'}^2p_{i,\jmath}}\Big]=:\mathscr{V}_1+\mathscr{V}_2.
	\]
	The proposed variance estimator is
	\[
	\widehat{\sigma}_{\jmath,\jmath'}^2=
	\E_n\Big[\frac{d_i(\jmath')(\widehat{\varsigma}_{i,\jmath}-\widehat{\theta}_{\jmath,\jmath'})^2}{\widehat{p}_{\jmath'}^2}\Big]+
	\E_n\Big[\frac{\widehat{p}_{i,\jmath'}^2d_i(\jmath)(y_i-\widehat{\varsigma}_{i,\jmath})^2}{\widehat{p}_{\jmath'}^2\widehat{p}^2_{i,\jmath}}\Big]
	=:\widehat{\mathscr{V}}_1+\widehat{\mathscr{V}}_2.
	\]
	I begin with $\widehat{\mathscr{V}}_1$.
	\begin{align*}
	\widehat{\mathscr{V}}_1=&\E_n\Big[\frac{d_i(\jmath')(\varsigma_{i,\jmath}-\theta_{\jmath,\jmath'})^2}{p_{\jmath'}^2}\Big]+
	\E_n\Big[\frac{d_i(\jmath')(\varsigma_{i,\jmath}-\theta_{\jmath,\jmath'})^2}{\widehat{p}_{\jmath'}^2p_{\jmath'}^2}(p_{\jmath'}-\widehat{p}_{\jmath'})(p_{\jmath'}+\widehat{p}_{\jmath'})\Big]+\\
	&\E_n\Big[\frac{d_i(\jmath')[(\widehat{\varsigma}_{i,\jmath}-\widehat{\theta}_{\jmath,\jmath'})^2-(\varsigma_{i,\jmath}-\theta_{\jmath,\jmath'})^2]}{\widehat{p}_{\jmath'}^2}\Big].
	\end{align*}
	The first term is consistent for $\mathscr{V}_1$ under Assumptions \ref{SA-Assumption: ID-counterfactual} and \ref{SA-Assumption: QMLE}.
	Since $\widehat{p}_{\jmath'}=p_{\jmath'}+o_\P(1)$, the second term is $o_\P(1)$ due to Assumption \ref{SA-Assumption: ID-counterfactual}. For the third term, note 
	\[
	(\widehat{\varsigma}_{i,\jmath}-\widehat{\theta}_{\jmath,\jmath'})^2-(\varsigma_{i,\jmath}-\theta_{\jmath,\jmath'})^2=(\widehat{\varsigma}_{i,\jmath}^2-\varsigma_{i,\jmath}^2)+(\widehat{\theta}_{\jmath,\jmath'}^2-\theta_{\jmath,\jmath}^2)-2(\widehat{\theta}_{\jmath,\jmath'}-\theta_{\jmath,\jmath'})\widehat{\varsigma}_{i,\jmath}-2\theta_{\jmath,\jmath'}(\widehat{\varsigma}_{i,\jmath}-\varsigma_{i,\jmath}).
	\]
	Due to the uniform consistency shown in Theorem \ref{SA-thm: QMLE}, the third term is $o_\P(1)$ as well.
	
	Moreover,
	\[
	\begin{split}
	\widehat{\mathscr{V}}_2=
	&\E_n\bigg[\frac{p_{i,\jmath'}^2d_i(\jmath)\epsilon_{i,\jmath}^2}{p_{\jmath'}^2p_{i,\jmath}^2}\bigg]+
	\E_n\bigg[\frac{p_{i,\jmath'}^2d_i(\jmath)\epsilon_{i,\jmath}^2}{p_{i,\jmath}^2}\bigg](\widehat{p}_{\jmath'}^{-2}-p_{\jmath'}^{-2})+
	\E_n\bigg[\frac{p_{i,\jmath'}^2d_i(\jmath)\epsilon_{i,\jmath}^2}{\widehat{p}_{\jmath'}^2}(p_{i,\jmath}^{-2}-\widehat{p}_{i,\jmath}^{-2})\bigg]+\\
	&\E_n\bigg[\frac{(\widehat{p}_{i,\jmath'}^2-p_{i,\jmath'}^2)d_i(\jmath)\epsilon_{i,\jmath}^2}{\widehat{p}_{\jmath'}^2\widehat{p}_{i,\jmath}^2}\bigg]+
	\E_n\bigg[\frac{\widehat{p}_{i,\jmath'}^2d_i(\jmath)((\epsilon_{i,\jmath}+\varsigma_{i,\jmath}-\widehat{\varsigma}_{i,\jmath})^2-\epsilon_{i,\jmath}^2)}{\widehat{p}_{\jmath'}^2\widehat{p}_{i,\jmath}^2}\bigg].
	\end{split}
	\]
	By Assumption \ref{SA-Assumption: QMLE}, the first term is consistent for $\mathscr{V}_2$ and the remainders are all $o_\P(1)$. The desired result in part (ii) then follows by the consistency of the variance estimator and part (i).
\end{proof}

\subsubsection*{Proof of Theorem \ref{SA-thm: uniform inference}}
\begin{proof}
    By definition, in this context $\varsigma_{i,\jmath,\tau}=\P(y_i(\jmath)\leq \tau|\balpha_i,\bz_i)$,  $y_{i,\tau}=\sum_{\jmath=0}^{J}d_i(\jmath)\I(y_i(\jmath)\leq \tau)$, and the expansion for $\widehat{\theta}_{\jmath,\jmath'}(\tau)$ given in the proof of Theorem \ref{SA-thm: pointwise inference} becomes
	\[
	\begin{split}
	\sqrt{n}(\widehat{\theta}_{\jmath,\jmath'}(\tau)-
	\theta_{\jmath,\jmath'}(\tau))=&
	\frac{1}{\sqrt{n}}\sum_{i=1}^n\varphi_{i,\jmath,\jmath'}(\tau)+
	\frac{1}{\sqrt{n}}\sum_{i=1}^n\mathscr{R}_{i,\tau}+
	\Big(\frac{p_{\jmath'}}{\widehat{p}_{\jmath'}}-\frac{p_{\jmath'}}{p_{\jmath'}}\Big)\cdot\frac{1}{\sqrt{n}}\sum_{i=1}^n\mathscr{R}_{i,\tau}+\\
	&\sqrt{n}\theta_{\jmath,\jmath'}(\tau)(p_{\jmath'}-\widehat{p}_{\jmath'})\Big(\frac{1}{\widehat{p}_{\jmath'}}-\frac{1}{p_{\jmath'}}\Big)+\\
	&\sqrt{n}\frac{p_{\jmath'}-\widehat{p}_{\jmath'}}{\widehat{p}_{\jmath'}}\left(\E_n\left[
	\frac{d_i(\jmath')\varsigma_{i,\jmath,\tau}}{p_{\jmath'}}+
	\frac{p_{i,\jmath'}}{p_{\jmath'}}\frac{d_i(\jmath)(y_{i,\tau}-\varsigma_{i,\jmath,\tau})}{p_{i,\jmath}}\right]-\theta_{\jmath,\jmath'}(\tau)\right).
	\end{split}
	\]
	The definition of $\mathscr{R}_{i,\tau}$ is the same, but I make 
	its dependence on $\tau$ explicit.
	
	Regarding the first term, by Lemma A.2 of \cite{Donald-Hsu_2014_JoE}, the function class
	$\Big\{(\balpha_i,\bz_i,s_i,y_i)\mapsto\varphi_{i,\jmath,\jmath'}(\tau): \tau\in\mathcal{Y}
	\Big\}$
	is Donsker, and thus the weak convergence follows by Donsker's Theorem \citep[][Section 2.8.2]{vandeVaart_book_1996}. 
	
	Then, it remains to show that the remainder of the above expansion is $o_\P(1)$ uniformly over $\tau\in\mathcal{Y}$, denoted by $\tilde{o}_\P(1)$ within this proof. In the fourth term, $\theta_{\jmath,\jmath'}(\tau)$ is bounded uniformly over $\tau$ and $\widehat{p}_{\jmath'}$ does not depend on $\tau$. Thus, it is $\tilde{o}_\P(1)$. Regarding the last term, $\sqrt{n}(p_{\jmath'}-\widehat{p}_{\jmath'})/\widehat{p}_{\jmath}=O_\P(1)$,which does not depend on $\tau$, and the terms in the bracket is $\tilde{o}_\P(1)$ by uniform law of large numbers. Then, it remains to bound the second term since the third one must be of smaller order. Recall that $\frac{1}{\sqrt{n}}\sum_{i=1}^n\mathscr{R}_{i,\tau}$ can be decomposed into
	\begin{align*}
	&\frac{1}{\sqrt{n}}\sum_{i=1}^n\bigg[\frac{p_{i,\jmath'}}{p_{\jmath'}}d_i(\jmath)(y_{i,\tau}-\varsigma_{i,\jmath,\tau})\Big(
	\frac{1}{\widehat{p}_{i,\jmath}}-\frac{1}{p_{i,\jmath}}\Big)\bigg]+
	\frac{1}{\sqrt{n}}\sum_{i=1}^n\bigg[\Big(\frac{\widehat{p}_{i,\jmath'}-p_{i,\jmath'}}{p_{\jmath'}}\Big)\frac{d_i(\jmath)(y_{i,\tau}-\varsigma_{i,\jmath,\tau})}{\widehat{p}_{i,\jmath}}\bigg]\\
	&+\frac{1}{\sqrt{n}}\sum_{i=1}^n\bigg[\Big(\frac{d_i(\jmath')}{p_{\jmath'}}-
	\frac{\widehat{p}_{i,\jmath'}d_i(\jmath)}{p_{\jmath'}\widehat{p}_{i,\jmath}}\Big)(\widehat{\varsigma}_{i,\jmath,\tau}-\varsigma_{i,\jmath,\tau})\bigg]=:I_1+I_2+I_3.
	\end{align*}
	
	For $I_1$, first notice that conditional on $\mathcal{H}=\{\bm{d}_{i}\}_{i=1}^n\cup\bar{\mathcal{F}}\cup\{\bx_i,\bw_i\}_{i=1}^n$, as defined in the proof of Theorem \ref{SA-thm: pointwise inference}, the summand in $I_1$ is mean zero for any $\tau$, and $\widehat{p}_{i,\jmath}$ and $p_{i,\jmath}$ do not depend on $\tau$.
	Then, conditional on the data, define
	\[
	\mathcal{T}=\Big\{\bt=(t_1,\cdots, t_n)\in\mathbb{R}^n: t_i=p_{i,\jmath'}d_i(\jmath)\epsilon_{i,\jmath,\tau}\Big(\frac{1}{\widehat{p}_{i,\jmath}}-\frac{1}{p_{i,\jmath}}\Big),\tau\in\mathbb{R}\Big\},
	\]
	where $\epsilon_{i,\jmath,\tau}=\I(y_i(\jmath)\leq \tau)-\varsigma_{i,\jmath,\tau}$.
	Define the norm $\|\cdot\|_{n,2}$ on $\mathbb{R}^n$ by $\|\bt\|^2_{n,2}=\E_n[t_i^2]$. For any $\varepsilon>0$, the covering number $N(\mathcal{T},\|\cdot\|_{n,2},\varepsilon)$ is the infimum of the cardinality of $\varepsilon$-nets of $\mathcal{T}$.
	
	Then, let $\{\omega_i\}_{i=1}^n$ be a sequence of independent Rademacher random variables that are independent of the data, and $\E_{\bomega}[\cdot]$ denotes the expectation with respect to the distribution of $\bomega=(\omega_1,\cdots,\omega_n)$.
	By Symmetrization Inequality and Dudley's inequality,
	\[
	\E\Big[\sup_{\tau\in\mathbb{R}}|\frac{1}{\sqrt{n}}
	\sum_{i=1}^{n}t_i|\Big|\mathcal{H}\Big]
	\leq 2\E\Big[\E_{\bomega}\Big[\sup_{\tau\in\mathbb{R}}|\frac{1}{\sqrt{n}}
	\sum_{i=1}^{n}t_i\omega_i|\Big]\Big|\mathcal{H}\Big]
	\lesssim
	\int_0^{\Theta}\sqrt{\log N(\mathcal{T},\|\cdot\|_{n,2},\varepsilon)}d\varepsilon,
	\]
	where $$\Theta:=2\sup_{\bt\in\mathcal{T}}\|\bt\|_{n,2}=
	2\sup_{\bt\in\mathcal{T}}\Big(\E_n\Big[p_{i,\jmath'}^2d_i(\jmath)\epsilon_{i,\jmath,\tau}^2\Big(\frac{1}{\widehat{p}_{i,\jmath}}-\frac{1}{p_{i,\jmath}}\Big)^2\Big]\Big)^{1/2}\lesssim\Big(\E_n\Big[(\widehat{p}_{i,\jmath}^{-1}-p_{i,\jmath}^{-1})^2\Big]\Big)^{1/2}.$$
	The last inequality follows by the boundedness of the indicators and conditional distribution functions.
	Also, by properties of indicator functions and conditional distribution functions and using Theorem \ref{SA-thm: QMLE}, $N(\mathcal{T},\|\cdot\|_{n,2},\varepsilon)\lesssim (\Theta/\varepsilon)^2$ 
	and $\int_{0}^{\Theta}\sqrt{\log N(\mathcal{T},\|\cdot\|_{n,2}, \varepsilon)}d\varepsilon\lesssim_\P \delta_{KT}^{-1}+h_{K,\alpha}^m+h_{K,\varrho}^{2m}$, which suffices to show that $I_1=\tilde{o}_\P(1)$.
	$I_2$ can be treated similarly.
	
	Regarding $I_3$, recall that
	$p_{\jmath'}I_3=\frac{1}{\sqrt{n}}\sum_{i=1}^n
	[(\widehat{\varsigma}_{i,\jmath,\tau}-\varsigma_{i,\jmath,\tau})(d_i(\jmath')-\frac{p_{i,\jmath'}d_i(\jmath)}{p_{i,\jmath}})]+
	\frac{1}{\sqrt{n}}\sum_{i=1}^n[(\widehat{\varsigma}_{i,\jmath,\tau}-\varsigma_{i,\jmath,\tau})(\frac{p_{i,\jmath'}d_i(\jmath)}{p_{i,\jmath}}-\frac{\widehat{p}_{i,\jmath'}d_i(\jmath)}{\widehat{p}_{i,\jmath}})]
	=:I_{3,1}+I_{3,2}$.
	For $I_{3,1}$, use the decomposition in the proof of Theorem \ref{SA-thm: pointwise inference} and the argument for $I_{1}$, and then it follows that $I_{3,1}=\tilde{o}_\P(1)$. 
	
	Finally, I claim that
	$\widehat{\varsigma}_{i,\jmath,\tau}-\varsigma_{i,\jmath,\tau}=\tilde{O}_\P(\delta_{KT}^{-1}+h_{K,\alpha}^m+h_{K,\varrho}^{2m})$,  which is proved below, and then it follows that $I_{3,2}=\tilde{o}_\P(1)$, which completes the proof.
	
	I will follow the notation used in the proof of Theorem \ref{SA-thm: QMLE}. 
	For $J_1$ in $\bA_n$, by Assumption \ref{SA-Assumption: QMLE, uniform}(b),  $\frac{1}{K}\sum_{j\in\mathcal{N}_{i,\jmath}}\frac{\bpi_j\bar{r}_{j,\jmath,\tau}}{\bar{V}_{\tty}(\zeta_j)}=\tilde{O}_\P(h_{K,\alpha}^m)$, where $\bar{r}_{j,\jmath,\tau}$ is the approximation error defined as before for each $\tau$. On the other hand,
	define the set
	\[
	\mathcal{T}=\Big\{\bt=(t_1,\cdots, t_n)\in\mathbb{R}^n: t_j=\frac{d_{j}(\jmath)\I(j\in\mathcal{N}_i)\epsilon_{j,\jmath,\tau}\bpi_{j,\subi}}{\bar{V}_{\tty}(\psi_{\tty}^{-1}(\varsigma_{j,\jmath,\tau}))},\tau\in\mathcal{Y}, 1\leq i\leq n
	\Big\}.
	\]
	Note that $(n/K)\E_n[t_j]=\frac{1}{K}\sum_{j\in\mathcal{N}_{i,\jmath}}\bpi_{j,\subi}\epsilon_{j,\jmath,\tau}/\bar{V}_{\tty}(\psi_{\tty}^{-1}(\varsigma_{j,\jmath,\tau}))$ has mean zero conditional on $\mathcal{H}$ and can be treated exactly the same way as for $I_1$ before. Note that I also require uniformity across $1\leq i\leq n$. Thus, in this case the diameter $\Theta\lesssim_\P\sqrt{K/n}$ and the covering number $N(\mathcal{T},\|\cdot\|_{n,2},\varepsilon)\lesssim n(1/\varepsilon)^2$, which leads to $\sup_{\tau\in\mathcal{Y}}\max_{1\leq i\leq n}|\frac{n}{K}\E_n[t_j]|\lesssim_\P\sqrt{\log n}/\sqrt{K}$.
	The other terms in $\bA_n$ can be handled similarly. The analysis of $\bV_n$ is similar to that in the proof of Theorem \ref{SA-thm: QMLE} by noting that in this case  $\psi_{\tty}^{-1}(\varsigma_{i,\jmath,\tau})$ must be contained in a compact set by definition.
\end{proof}

\subsubsection*{Proof of Corollary \ref{SA-coro: functional delta method}}
\begin{proof}
By the functional delta method \citep[e.g.,][Theorem 3.9.4]{vandeVaart_book_1996} and the
linearity of the Hadamard derivative, the weak convergence to a Gaussian process is implied.
\end{proof}

\subsubsection*{Proof of Corollary \ref{SA-coro: multiplier bootstrap}}
\begin{proof}
	The result follows by Corollary 2 of \cite{Ao-Calonico-Lee_2019_JBES}, and more detailed proof strategy can be found in \cite{Donald-Hsu_2014_JoE}. Note that for the first part, a uniformly consistent estimator of $\varphi_{i,\jmath,\jmath'}$ is readily available by Theorem \ref{SA-thm: QMLE}.
\end{proof}

\subsection{Proofs for Main Paper}
\subsubsection*{Proof of Theorem 4.1}
\begin{proof}
	The result follows by the second par of Theorem \ref{thm: IMD hsk}.
\end{proof}

\subsubsection*{Proof of Theorem 4.2}
\begin{proof}
	The result follows by Theorem \ref{thm: uniform convergence of factors}.
\end{proof}

\subsubsection*{Proof of Theorem 4.3}
\begin{proof}
	The result follows by Theorem \ref{thm: consistency of latent mean}.
\end{proof}

\subsubsection*{Proof of Theorem 4.4}
\begin{proof}
	The result follows by Theorem \ref{SA-thm: QMLE}. Note that for the local least squares regressions, Assumption \ref{SA-Assumption: QMLE}(a),(b), and (c) are trivially satisfied. Since there is no additional high-rank regressors, the rate condition $\delta_{KT}h_{K,\varrho}^{2m}\lesssim 1$ is unnecessary.
\end{proof}

\subsubsection*{Proof of Theorem 4.5}
\begin{proof}
	The result follows by Theorem \ref{SA-thm: pointwise inference}. Since there are no additional high-rank regressors, the rate conditions $\delta_{KT}h_{K,\varrho}\lesssim 1$ and $\sqrt{n}h_{K,\varrho}^{4m}$ are unnecessary.
\end{proof}

\subsubsection*{Proof of Theorem 5.1}
\begin{proof}
	The result follows by Theorem \ref{SA-thm: uniform inference}.
\end{proof}

\subsubsection*{Proof of Corollary 5.1.1}
\begin{proof}
	The result follows by Corollary \ref{SA-coro: multiplier bootstrap}.
\end{proof}

\bibliography{Feng_2021--Bibliography}
\bibliographystyle{econometrica}

\end{document}
